# Supplementary material for: UniLab: A Heterogeneous Architecture for Robot RL Beyond GPU-Dominant Paradigms
Source: arXiv:2605.30313 source file (2026-06-02)
Supplement: Supplementary file 1 [file 8_Appendix.tex]

\clearpage
\onecolumn

\makeatletter
\@ifundefined{appendices}{\appendix}{\appendices}
\makeatother

% Change subsection numbering in the appendix from A-A to A.1.

\makeatletter
\@ifundefined{thesubsectiondis}{}{%
}

% Match the IEEE appendix heading style used in the reference draft:
% "Appendix A. Title" instead of "Appendix A" followed by "Title".
\@ifundefined{@IEEEprocessthesectionargument}{}{%
  \def\@IEEEprocessthesectionargument#1{%
  \@ifmtarg{#1}{%
  \@IEEEappendixsavesection*{\appendixname~\thesectiondis}%
  \addcontentsline{toc}{section}{\appendixname~\thesection}}{%
  \@IEEEappendixsavesection*{\appendixname~\thesectiondis. #1}%
  \addcontentsline{toc}{section}{\appendixname~\thesection. #1}}}%
}
\makeatother

\newpage

% Prevent floats from taking the top of the appendix title page.
\makeatletter
\global\@topnum 0
\makeatother

\addtocontents{toc}{\protect\setcounter{tocdepth}{3}}

\begin{center}
    \Huge \textbf{Appendix}
\end{center}

\etocsettocstyle{\section*{Table of Contents}}{}
\tableofcontents

\vspace{1em}
\hrule
\vspace{2em}

\makeatletter
\global\@topnum 0
\makeatother

\section{Off-Policy Replay Path Case Study}
\label{app:offpolicy_replay_case_study}

% 本节补充主文的 System Attribution 小节，给出 SAC replay-based execution path 的系统归因案例研究。
This section complements the system-attribution analysis in Section~\ref{subsec:end_to_end_training} with a detailed case study of the SAC replay-based execution path.

% 除非另有说明，本节（Appendix~\ref{app:offpolicy_replay_case_study}）所有 timeline statistics 都来自同一台 A100 机器上的 Perfetto traces。该机器使用单张 NVIDIA A100 80GB PCIe GPU、driver 560.35.05、CUDA 12.6、双路 Intel Xeon Gold 5320 CPU 和 188GiB system memory。learner cycle 从一次 learner/weight_sync_write 结束到下一次结束；丢弃前五个 warmup cycles；每个 retained cycle 对应 2048 environment steps；per-cycle 数值报告 retained cycles 的均值。
Unless otherwise stated, all timeline statistics in this section (Appendix~\ref{app:offpolicy_replay_case_study}) are computed from Perfetto traces collected on the same A100 machine: one NVIDIA A100 80\,GB PCIe GPU with driver 560.35.05 and CUDA~12.6, two Intel Xeon Gold 5320 CPUs with 104 logical CPU threads, and 188\,GiB system memory. A learner cycle is measured from the end of one \texttt{learner/weight\_sync\_write} event to the end of the next such event; the first five cycles are discarded as warmup, and each retained cycle corresponds to 2048 environment steps. Reported per-cycle values are means over the retained cycles.

\subsection{Baseline GPU-Cache SAC Path}
\label{app:baseline_gpu_cache_sac}

% 这里先定义 SAC-A：本文中 SAC-A 指用于对比的 straightforward baseline，不是新的 SAC 算法；它对应 sample-before-transfer pipeline 之前的 GPU-cache replay path。这个 baseline 仍然是 heterogeneous design：CPU collector 用 learner 同步来的 actor 权重推进 batched environment 并写入 CPU shared replay storage；learner 在 accelerator 上持有 SAC actor/critic 并周期性把更新后的 actor 权重发回 collector。
We use SAC-A to denote the straightforward SAC baseline used for comparison in this case study, not a separate SAC algorithm. It corresponds to the GPU-cache replay path before the sample-before-transfer pipeline. This baseline is already a heterogeneous design: a CPU collector process runs a CPU actor synchronized from learner weights, advances the batched environment, and writes transitions into shared CPU replay storage. The learner process holds the SAC actor and critic networks on the accelerator and periodically publishes updated actor weights back to the collector. This organization already separates CPU simulation from GPU learning.

% 剩余成本在 replay boundary：CUDA 路径由 learner 维护 device-side replay cache；采样时新增 replay rows 会 lazy sync 到 GPU cache，random indices 被移到 device，然后从 cached replay tensors gather sampled batch，因此 replay-cache maintenance 和 random replay access 进入 learner hot update path。
The remaining cost lies in the replay boundary. In the CUDA path, the learner maintains a device-side replay cache. When the learner samples, newly appended replay rows are lazily synchronized into this GPU cache, random indices are moved to the device, and the sampled batch is gathered from the cached replay tensors before SAC updates are performed. Thus, replay-cache maintenance and random replay access are part of the learner's hot update path. This increases GPU-resident replay storage and inserts replay-management work before the critic, actor, and target-network updates.

\subsection{Sample-Before-Transfer Replay Pipeline}
\label{app:sample_before_transfer}

% \method{} 将 replay boundary 从 replay buffer 移到 sampled batch。collector 继续做 CPU actor inference、environment stepping 和 replay insertion；当 learner 请求下一批训练数据时，collector 在 CPU replay snapshot 上采样并 pack 到两个 shared pack slots 之一，CUDA 下这些 slots 作为 pinned H2D 源，由 learner-side background H2D submit thread 异步传入 cold GPU batch slot，同时 learner 使用当前 hot slot。
\method{} moves the replay boundary from the replay buffer to the sampled batch. The collector still performs CPU actor inference, environment stepping, and replay insertion. Once the learner requests the next training batch, the collector samples rows from a replay snapshot on the CPU and packs them into one of two shared pack slots. On CUDA, these pack slots are registered as pinned host-memory sources for asynchronous H2D transfer. A learner-side background H2D submit thread then transfers the packed batch into the cold GPU batch slot while the learner consumes the current hot slot.

% 这个 distinction 对理解 memory path 很重要：main replay storage 仍然是 CPU shared replay storage；CUDA-specific pinned-memory path 只作用在作为 H2D 源的 shared pack slots。learner 从 hot GPU batch slot 的 device-resident views 读取数据，执行 SAC 更新，并在下一次 batch handoff 交换 hot/cold slots。
This distinction matters for interpreting the memory path. The main replay storage remains CPU shared replay storage; the CUDA-specific pinned-memory path applies to the shared pack slots used as H2D sources. The learner consumes device-resident views from the hot GPU batch slot, executes SAC critic, actor, entropy-temperature, and target-network updates, and swaps the hot and cold slots at the next batch handoff.

% 图~\ref{fig:app_sac_old_new_timeline} 把 baseline 和 double-buffer path 放在同一个 retained learner cycle 时间轴上。图中的 env/replay/H2D/sync/stall/gap 分别表示 environment stepping、replay insertion、host-to-device transfer、actor-weight publication/consumption、等待，以及从 learner weight publication 结束到下一次 learner update 开始之间的 resume gap。关键比较是 replay ownership 和 timing 的变化：baseline 把 replay sampling 和 lazy synchronization 留在 learner hot path，double-buffer path 则提前准备下一批 sampled batch，使 CPU packing 和 H2D transfer 与 GPU learner updates 重叠。
Figure~\ref{fig:app_sac_old_new_timeline} places the baseline and double-buffer paths on the same retained learner-cycle time axis. In the figure, \emph{env}, \emph{replay}, \emph{H2D}, \emph{sync}, \emph{stall}, and \emph{gap} denote environment stepping, replay-buffer insertion, host-to-device transfer, actor-weight publication or consumption, waiting, and the delay from learner weight publication to the next first learner update, respectively. The key comparison is the change in replay ownership and timing: the baseline keeps replay sampling and lazy synchronization on the learner-side critical path, whereas the double-buffer path prepares the next sampled batch early enough to overlap CPU packing and H2D transfer with GPU learner updates.

\begin{figure}[!htbp]
    \centering
    \includegraphics[width=0.85\columnwidth]{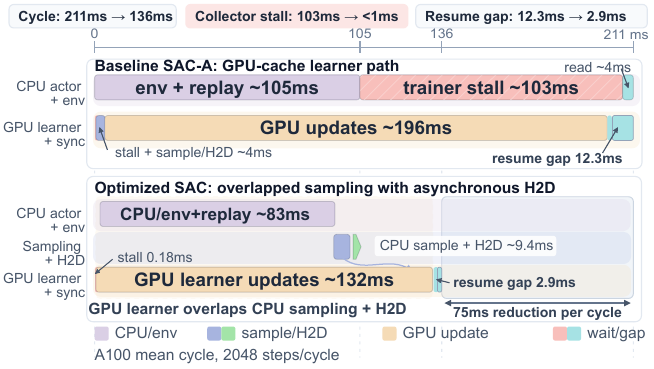}
    \caption{Baseline SAC-A and optimized SAC learner-cycle timelines on A100. Durations are means per retained learner cycle using the cycle definition above; each cycle corresponds to 2048 environment steps. The optimized double-buffer path reduces cycle time from 211\,ms to 136\,ms, collector stall from 103\,ms to below 1\,ms, and resume gap from 12.3\,ms to 2.9\,ms.}
    \label{fig:app_sac_old_new_timeline}
\end{figure}

\subsection{Trace-Based Attribution}
\label{app:trace_based_attribution}

% 本节分析 baseline GPU-cache SAC path 和 \method{} double-buffer path 的 A100 Perfetto traces。这些 traces 提供机制和时序证据，说明 replay sampling、H2D transfer、learner updates 和 weight publication 发生在哪里；由于两个 traces 中 learner update kernels 的时长也不同，归因需要和后续 ablation 一起解释。
We analyze A100 Perfetto traces for the baseline GPU-cache SAC path and the \method{} double-buffer path. These traces provide mechanism and timing evidence: they show where replay sampling, H2D transfer, learner updates, and weight publication occur. Because learner-update kernels also differ in duration across traces, the attribution is interpreted together with the ablation below.

\begin{figure}[!htbp]
    \centering
    \includegraphics[width=\linewidth]{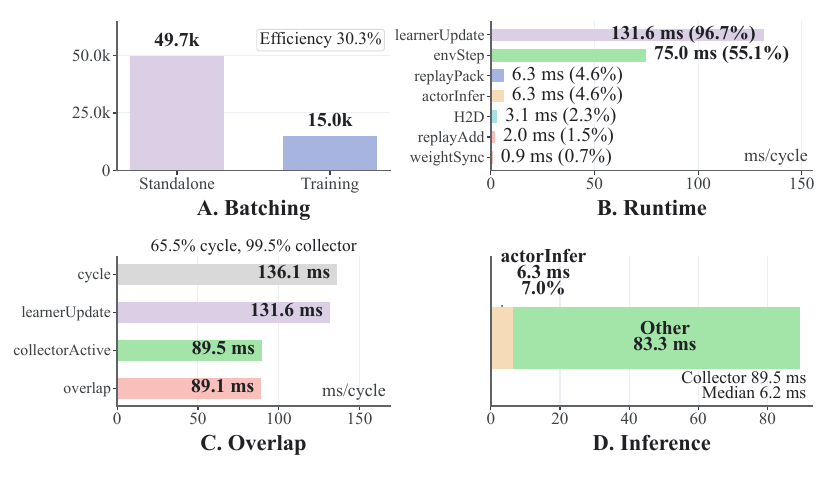}
    % 图注只保留 panel 级读法，详细缩写和统计口径在正文中说明。
    \caption{System-attribution summary for the optimized SAC trace. Panel A reports batching efficiency, with \emph{Eff.} defined as training-pipeline throughput divided by standalone simulator throughput. Panels B--D summarize runtime components, simulation-learning overlap, and collector-side CPU actor-inference cost.}
    \label{fig:app_sac_system_attribution}
\end{figure}

% 图~\ref{fig:app_sac_system_attribution} 从四个互补视角总结 optimized trace：A 面板比较 standalone simulator throughput 和 SAC training pipeline 内的 throughput，Eff. 是两者比值；B--D 面板使用前述 retained learner-cycle 定义并报告 per-cycle means。B 面板中的 Lrn/Env/Pack/Inf/H2D/Add/Sync 分别对应 learner update、environment stepping、CPU replay sampling and batch packing、collector CPU actor inference、host-to-device batch transfer、replay-buffer insertion 和 actor-weight publication/consumption。C 面板把 cycle-level timing terms 汇总为 Cyc/Lrn/Col/Ovl，分别表示 learner-cycle duration、learner-update time、collector-active time 及二者 overlap。D 面板进一步把 collector-active time 与 CPU actor-inference share 分离出来。
Figure~\ref{fig:app_sac_system_attribution} summarizes the optimized trace from four complementary views. Panel A compares standalone simulator throughput with throughput inside the SAC training pipeline; the reported efficiency is their ratio. Panels B--D use the retained learner-cycle definition above and report per-cycle means. In Panel B, \emph{Lrn}, \emph{Env}, \emph{Pack}, \emph{Inf}, \emph{H2D}, \emph{Add}, and \emph{Sync} denote learner update, environment stepping, CPU replay sampling and batch packing, collector CPU actor inference, host-to-device batch transfer, replay-buffer insertion, and actor-weight publication or consumption. Panel C groups the cycle-level timing terms: \emph{Cyc}, \emph{Lrn}, \emph{Col}, and \emph{Ovl} denote learner-cycle duration, learner-update time, collector-active time, and their overlap. Panel D isolates collector-side actor inference by comparing it with total collector-active time.

% 在 traced 500-iteration window 中，double-buffer path 将训练时间从 107.50s 降到 70.58s；丢弃前五个 cycles 后，mean learner cycle 从 211.31ms 降到 136.10ms。每个 cycle 对应 2048 environment steps，因此 throughput 从 9.69k 提升到 15.05k environment steps per second。
In the traced 500-iteration window, the double-buffer path reduces training time from 107.50\,s to 70.58\,s, a 34.34\% reduction in wall-clock time. After dropping the first five cycles, the mean learner cycle decreases from 211.31\,ms to 136.10\,ms. With 2048 environment steps per learner cycle, this corresponds to an increase from 9.69k to 15.05k environment steps per second.

% 最清晰的变化在 replay hot path：baseline 中 learner/replay_sample 平均 3.64ms，并包含 lazy replay synchronization；\method{} 中 learner-side replay consumption 降到 0.23ms。replay preparation 仍然存在，但被移出 learner hot path：CPU packing 为 6.30ms，GPU H2D transfer 为 3.13ms，且 collector-active time 的 99.50% 与 learner updates 重叠；剩余 H2D handoff wait 约为 0.055ms/cycle。
The clearest change is on the replay hot path. In the baseline trace, \texttt{learner/replay\_sample} takes 3.64\,ms on average and includes lazy replay synchronization, with \texttt{replay/h2d\_lazy\_sync} taking 1.88\,ms on the CPU wrapper path and \texttt{gpu/replay\_h2d\_lazy\_sync} taking 1.84\,ms on the GPU event path. In the \method{} trace, learner-side replay consumption is reduced to 0.23\,ms on average. Replay preparation still exists, but it is moved out of the learner hot path: CPU packing takes 6.30\,ms, and GPU H2D transfer takes 3.13\,ms, while 99.50\% of collector-active time overlaps with learner updates. The remaining H2D handoff wait is about 0.055\,ms per cycle.

\subsection{Ablating the Path from GPU-Cache SAC to Sample-Before-Transfer}
\label{app:sac_replay_ablation_c_to_baseline}

% trace-based attribution 给出了 replay path 变化的时序证据，但还需要消融来区分 GPU-cache residency、sampled-batch transfer 和 transfer orchestration。本小节在同一 A100 机器上比较四个 SAC replay path 变体；这些变体保持 SAC objective 和 update equations 不变，只移动 replay boundary。
The trace-based attribution gives timing evidence for the replay-path change, but it does not by itself separate replay-data residency from transfer orchestration. We run a SAC replay-path ablation on the same A100 machine. The four variants preserve SAC's objective and update equations; only the replay boundary changes, moving from learner-side GPU-cache replay to sampled-batch transfer and then to the CPU-pinned double-buffer path.

% 四个变体构成一条受控迁移链。C 是 old-SAC-like GPU-cache compatibility control，保留 learner-side GPU replay cache、lazy sync newly appended replay rows 和 GPU-cache random gather；B 保留 GPU-cache replay，但使用现代 ablation framework，因此主要体现 GPU-cache 路径中的调度改善；A 移除 GPU-cache residency，转为 sampled-batch transfer，但没有完整 pinned/asynchronous overlap；baseline 在 A 的 CPU-resident sampled-batch 边界上加入 pinned pack slots、one-tick async H2D 和 hot/cold GPU batch slots。
The variants form a controlled migration chain. C is the old-SAC-like GPU-cache compatibility control: replay samples are still served through a learner-side GPU replay cache with lazy synchronization of newly appended rows and random gather from cached replay tensors. B keeps the same GPU-cache replay organization, but uses the modern ablation framework; its improvement over C therefore primarily reflects scheduling and runner-level overlap rather than a change in replay residency. A removes the GPU-cache resident replay component and moves the boundary to sampled-batch transfer, but it uses a synchronous/pageable transfer path rather than the full pinned asynchronous pipeline. The baseline keeps A's CPU-resident sampled-batch boundary and adds registered pinned pack slots, one-tick asynchronous H2D, and hot/cold GPU batch slots.

% 图中的统计口径也需要明确。Panel A 的 E2E 结果报告三次 seed 的均值和 sample standard deviation；Panel B 报告 learner-cycle median 和 p95；Panel C 区分 learner/replay_sample 事件和 learner-side boundary wait，其中 GPU wait 不是 kernel-level GPU idle；Panel D 报告 peak CUDA reserved memory，并把 learner-side GPU replay cache 贡献的部分单独列为 GPU-cache component。
The figure reports four complementary measurements. Panel A reports wall-clock E2E time as means over three seeds, with sample-standard-deviation error bars. Panel B reports learner-cycle medians, with diamonds marking p95 cycle time. Panel C focuses on the learner-side replay boundary. We report \emph{Replay sample mean} using the learner-side \texttt{learner/replay\_sample} event: in GPU-cache variants, this event includes learner-side sampling, gather, and lazy replay-cache synchronization; in sampled-batch variants, it measures the learner-side batch handoff and consumption path, not the CPU packing work that is scheduled earlier. \emph{GPU wait mean} reports learner-side boundary waiting before update computation, including waiting for data or replay-batch readiness, and should not be read as total kernel-level GPU idle time. The black marks indicate the corresponding medians. Panel D reports the mean peak CUDA reserved memory and separates the replay-cache portion as the GPU-cache component. This component is present in C and B because the learner maintains a full GPU replay cache, and absent in A and the baseline because they keep replay CPU-resident and retain only sampled GPU batch slots.

\begin{figure}[!htbp]
    \centering
    \includegraphics[width=\linewidth]{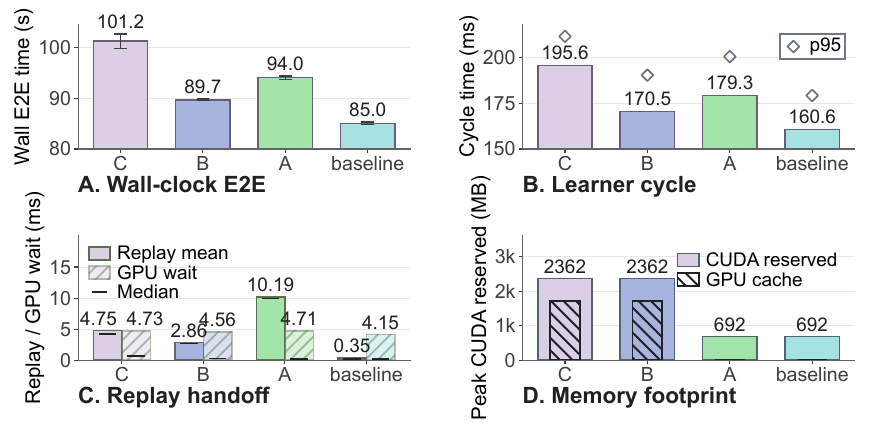}
    \caption{C-to-baseline ablation for the SAC replay path. Wall-clock E2E bars are three-seed means with sample-standard-deviation error bars. Learner-cycle bars are medians, with diamonds marking p95 cycle time. Panel C reports learner-side replay-sample and boundary-wait statistics; Panel D reports peak CUDA reserved memory and the measured GPU-cache component.}
    \label{fig:app_sac_replay_ablation}
\end{figure}

% 结果显示，不同技术差距对应不同指标变化。C 到 B 改善 E2E，主要来自 GPU-cache family 内部的调度改善；B 到 A 移除 GPU-cache component，显著降低 CUDA reserved memory，但同步/pageable sampled-batch handoff 暴露在 learner boundary 上，导致 replay sample time 和 E2E 变差；A 到 baseline 不重新引入 GPU cache，而是优化 transfer orchestration，因此恢复吞吐并保持低显存。
With these definitions, Figure~\ref{fig:app_sac_replay_ablation} shows that the variants affect different metrics for different reasons. Moving from C to B improves wall-clock time within the GPU-cache family, while CUDA reserved memory remains unchanged; this is consistent with a scheduling improvement rather than a memory-residency change. Moving from B to A removes the measured GPU-cache component and reduces peak CUDA reserved memory from 2362\,MB to 692\,MB, but the synchronous/pageable sampled-batch handoff becomes visible on the learner boundary, increasing replay-sample time and hurting E2E time. Moving from A to the baseline keeps the low-memory CPU-resident replay design and changes the transfer mechanism instead: pinned shared pack slots, one-tick asynchronous H2D, and hot/cold GPU slots reduce learner-side replay consumption from 10.19\,ms to 0.35\,ms and reduce wall time from 94.04\,s to 85.04\,s without reintroducing the GPU-cache component. Relative to C, the final baseline reduces wall time from 101.23\,s to 85.04\,s while also removing the measured GPU-cache footprint.

% 因此，消融把 trace-based attribution 与端到端收益连接起来：收益来自 replay runtime boundary 的重放置，而不是 SAC loss 的改变。replay work 仍然存在，但 ownership 和 timing 发生转移，使 learner 消费 ready device batches，而不是在 hot path 中维护和采样 capacity-scaled GPU replay cache。
This ablation connects the trace-based attribution to the end-to-end result. The gain comes from relocating the replay-runtime boundary, not from changing the SAC loss. Replay work remains, but shifts in ownership and timing: the learner consumes ready device batches instead of maintaining and sampling a capacity-scaled GPU replay cache on the hot update path.
\begin{figure}[!htbp]
    \centering
    \includegraphics[width=\columnwidth]{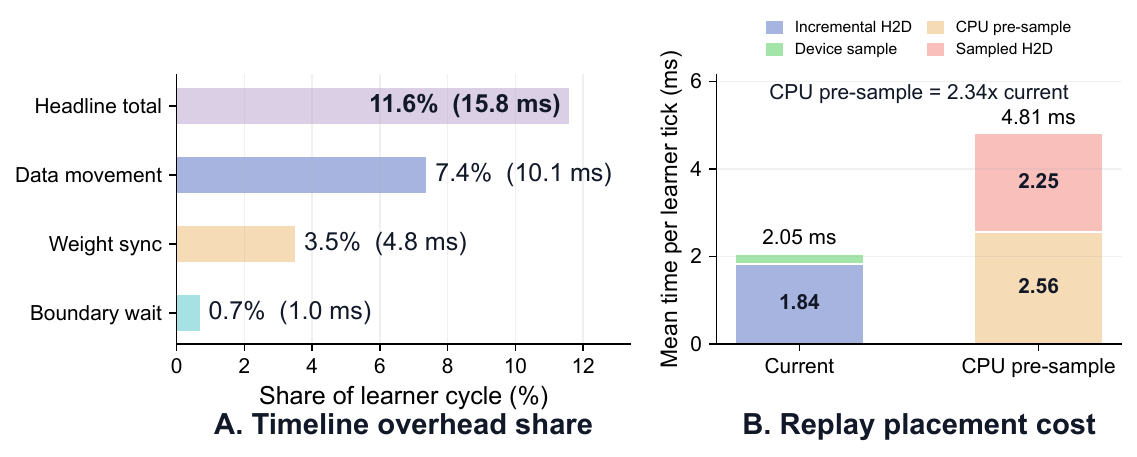}
    \caption{SAC buffer and communication overhead. Values in Panel A are means per retained learner cycle from the optimized SAC timeline; Panel A groups counted data-movement, weight-synchronization, and boundary-wait overhead by share of the mean learner cycle, with signal-ready context shown separately. Panel B reports an auxiliary replay-placement benchmark comparing current incremental-transfer/device-sampling and CPU pre-sample plus sampled-batch H2D schemes.}
    \label{fig:app_sac_buffer_communication}
\end{figure}

\subsection{Buffer and Communication Overhead}
\label{app:buffer_communication_overhead}

% 图~\ref{fig:app_sac_buffer_communication} 分解 optimized SAC timeline 中的数据移动、同步和残余等待，并把计入 headline overhead 的项与只作为调度/背压上下文报告的项分开。Data movement 包括 CPU-side replay sampling and packing、H2D submission、H2D transfer 和 transfer-completion wait；weight sync 包括 learner weight publication、D2H weight copy 和 collector-side weight read/update checking；boundary wait 包括 collector 和 learner 在 cycle boundary 的等待。Signal-ready context 单独报告：collector 已经准备好下一批数据并发出 ready signal，但 learner 尚未到达下一次 batch boundary；它表示 scheduling/backpressure slack，而不是额外 data-copy cost 或 learner-update waiting。
Figure~\ref{fig:app_sac_buffer_communication} combines a timeline overhead breakdown with an auxiliary replay-placement benchmark. Panel~A breaks down the data movement, synchronization, and residual waiting observed inside the optimized SAC timeline. We separate the counted overhead into three groups. \emph{Data movement} covers CPU-side replay sampling and batch packing, H2D submission, H2D transfer, and transfer-completion wait. \emph{Weight sync} covers learner weight publication, device-to-host (D2H) weight copy, and collector-side weight read/update checking. \emph{Boundary wait} covers collector and learner waiting at the cycle boundary. The figure also reports signal-ready context separately: the collector has already prepared the next batch and issued a ready signal, while the learner has not yet reached the next batch boundary. We treat this interval as scheduling and backpressure context rather than data-copy cost or learner-update waiting, so it is excluded from the counted overhead total.

% 在该 trace 中，主要计入的 data-movement、synchronization 和 boundary-wait overhead 合计为 15.82ms/cycle，即 136.10ms mean learner cycle 的 11.62%。其中 data movement 为 10.07ms/cycle，weight synchronization 为 4.79ms，residual boundary waiting 为 0.96ms。Signal-ready interval 较大但不计入 headline total，因为它描述 readiness/backpressure context，而不是直接 data-copy 或 learner-wait cost。
In this trace, the counted data-movement, synchronization, and boundary-wait overhead total is 15.82\,ms per cycle, or 11.62\% of the 136.10\,ms mean learner cycle. Data movement is the largest counted component at 10.07\,ms per cycle, weight synchronization contributes 4.79\,ms, and residual boundary waiting contributes 0.96\,ms. The signal-ready interval is larger, but it is reported outside the headline total because it describes readiness and backpressure context rather than a direct data-copy or learner-wait cost.

% Panel B 是同配置下的辅助 replay-placement benchmark，不属于 Panel A 的 retained-cycle overhead 汇总。该 benchmark 中 current placement 由 incremental H2D 和 device-side random sampling 组成，为 2.05ms/learner tick；CPU pre-sample plus sampled-batch H2D placement 为 4.81ms/learner tick，即 current placement 的 2.34x。这个结果说明 placement cost 需要和 overlap/scheduling 一起解释，而不能只看孤立的数据移动时间。
Panel B provides an auxiliary replay-placement benchmark under the same configuration, separate from the retained-cycle accounting in Panel~A. In this benchmark, the current placement combines incremental H2D with device-side random sampling and costs 2.05\,ms per learner tick. A CPU pre-sample plus sampled-batch H2D placement costs 4.81\,ms per learner tick, or 2.34$\times$ the current placement cost. This comparison is not part of the counted timeline overhead; instead, it shows why replay placement must be interpreted together with the overlap and scheduling structure of the full pipeline.

\begin{table*}[!t]
\centering
\small
\captionsetup{hypcap=false}

\setlength{\emergencystretch}{2em}
\hyphenpenalty=10000
\exhyphenpenalty=10000
\newcolumntype{L}[1]{>{\raggedright\arraybackslash\hyphenpenalty=10000\exhyphenpenalty=10000}p{#1}}

\caption{Trace-based attribution summary for the SAC replay path. The table reports what can be supported directly by the A100 timeline traces and where additional evidence is needed.}
\label{tab:sac_trace_attribution}

\begin{tabular}{@{}L{0.20\textwidth}L{0.34\textwidth}L{0.13\textwidth}L{0.25\textwidth}@{}}
    \toprule
    Mechanism & Evidence from traces & Strength & Safe interpretation \\
    \midrule
    End-to-end cycle reduction &
    Traced window decreases from 107.50\,s to 70.58\,s; post-warmup cycle decreases from 211.31\,ms to 136.10\,ms. &
    Strong &
    The double-buffer path is 1.52$\times$ faster over the traced window and 1.55$\times$ faster per post-warmup cycle. \\
    \midrule
    Learner replay hot path &
    \texttt{learner/replay\_sample} decreases from 3.64\,ms to 0.23\,ms on average. &
    Strong &
    Replay sampling no longer dominates the learner-side handoff before SAC updates. \\
    \midrule
    Collector-side CPU packing &
    Optimized trace records CPU-side replay packing with 32768 sampled transitions per batch. &
    Strong &
    Random replay packing is performed on the CPU side before transfer. \\
    \midrule
    Asynchronous H2D preparation &
    CPU pack takes 6.30\,ms and GPU H2D takes 3.13\,ms; 99.50\% of collector-active time overlaps with learner updates. &
    Strong &
    Replay preparation is still present, but it is largely hidden behind GPU learner computation. \\
    \midrule
    Hot/cold GPU batch slots &
    Optimized trace records alternating hot/cold batch-slot swaps between the two device slots. &
    Strong &
    The learner consumes one device batch while the next batch is prepared in the cold slot. \\
    \midrule
    Pinned shared pack slots &
    Trace metadata reports registered pinned shared host memory, with pinned and direct-pinned flags enabled. &
    Medium--strong &
    The trace supports pinned H2D source slots; the implementation should be cited for the \texttt{cudaHostRegister} detail. \\
    \midrule
    Actor-weight publication &
    \texttt{learner/weight\_sync\_write} decreases from 1.71\,ms to 0.94\,ms; weight-copy events remain visible. &
    Strong &
    Actor-weight publication remains a synchronous boundary, although it is small in this trace. \\
    \midrule
    GPU replay memory footprint &
    The new trace transfers 56.36\,MB for 32768 samples; two sampled batch slots are about 112.7\,MB under this layout. &
    Estimate &
    This supports a memory-footprint estimate, not a measured peak-memory claim. \\
    \bottomrule
\end{tabular}

\vspace{0.4\baselineskip}
\end{table*}

\subsection{What the Traces Do and Do Not Establish}
\label{app:trace_scope}

% traces 支持 execution-path change 及其 timing consequences，但不能单独支持 peak memory、exact H2D volume 或 cross-algorithm generality 等更强归因。
The traces establish the execution-path change and its timing consequences: replay preparation moves from learner-side GPU-cache sampling to collector-side CPU packing plus asynchronous H2D staging, new-batch preparation is almost fully overlapped with learner computation, and actor-weight publication remains an explicit synchronization boundary. They do not, by themselves, establish stronger claims about peak GPU memory, exact H2D volume reduction, or cross-algorithm generality; those claims require memory counters, byte counters for the baseline lazy-sync path, or corresponding TD3 / FlashSAC measurements.

\section{Domain Randomization Backends and Lifecycle}
\label{app:domain_randomization}

% \method{} 中的域随机化是任务和后端之间的契约，而不是算法层的新机制。
% 任务侧 provider 负责采样 workload 相关的随机变量，仿真后端声明自己能应用哪些物理参数覆盖。
% 运行时的 DomainRandomizationManager 负责校验契约、在 materialize 前应用 cold-start 模型变体、在 sparse reset 中注入 reset payload，并在物理步进前调度 interval 扰动。
% 这样，随机化就和状态 reset 与批量仿真的生命周期绑定在一起。
Domain randomization in \method{} is implemented as a task/backend contract rather
than as an algorithm-level feature.  A task-owned
\texttt{DomainRandomizationProvider} samples the quantities that are meaningful
for the workload, while the simulator backend advertises which physical
overrides it can apply.  The runtime mediator,
\texttt{DomainRandomizationManager}, validates this contract, applies
cold-start model variants before backend materialization, injects reset
payloads into sparse environment resets, and schedules interval perturbations
before physics stepping.  This keeps randomization tied to the same lifecycle
that already controls state reset and batched simulation.

\subsection{Runtime Lifecycle}
\label{app:dr_runtime_lifecycle}

% 表格~\ref{tab:app_dr_lifecycle} 区分当前实现中的生命周期阶段。
% 关键系统细节是 reset-time randomization 是 sparse 的：只有 \texttt{env\_ids} 中的环境会收到新的状态和新的随机化 payload。
% interval randomization 则不同，它在每个 vectorized env step 前检查一次，并发生在后端推进物理之前。
% observation noise 和 command sampling 属于任务侧逻辑，不需要后端物理参数覆盖。
Table~\ref{tab:app_dr_lifecycle} separates the lifecycle stages used by the
current implementation.  The important systems detail is that reset-time
randomization is sparse: only the environments listed in \texttt{env\_ids}
receive a new state and a new randomization payload.  Interval randomization is
different: it is checked once per vectorized environment step, before the
backend advances physics.  Per-observation noise and command sampling are
task-side operations and do not require backend-specific physical overrides,
although they may depend on backend sensor reads that must complete first.

\begin{table*}[t]
\centering
\small
\captionsetup{hypcap=false}

\setlength{\tabcolsep}{3pt}
\begin{tabular}{@{}
>{\raggedright\hyphenpenalty=10000\exhyphenpenalty=10000\arraybackslash}p{0.13\textwidth}
>{\raggedright\hyphenpenalty=10000\exhyphenpenalty=10000\arraybackslash}p{0.21\textwidth}
>{\raggedright\hyphenpenalty=10000\exhyphenpenalty=10000\arraybackslash}p{0.21\textwidth}
>{\raggedright\hyphenpenalty=10000\exhyphenpenalty=10000\arraybackslash}p{0.30\textwidth}@{}}
\toprule
\textbf{Lifecycle} & \textbf{Trigger} & \textbf{Owner} & \textbf{Randomized state} \\
\midrule
Backend initialization & DR init hook before backend
\texttt{materialize()} & Task provider builds an init plan; backend
materializes variants & Persistent
model or geometry variants assigned per environment, such as object-scale
variants expressed through \texttt{GeomSizeOverride}. \\
\midrule
Sparse reset & Environment creation and any later reset of terminated or
truncated \texttt{env\_ids} & Task provider samples reset state and optional
reset payload; backend applies supported fields & Initial
pose, velocity, commands, cached object/grasp state, mass, COM, gravity,
friction, actuator gains, and other supported physical fields. \\
\midrule
Scheduled interval & Each vectorized \texttt{step}; active at the configured
interval or when an equivalent task plan is non-empty & Task provider builds an
interval plan; backend
stages the perturbation for the upcoming physics step & Push forces and
body-force perturbations.  The current capability contract includes body
velocity deltas, but neither backend advertises support for them. \\
\midrule
Observation construction & Every task observation update & Task code & Actor
observation noise, history/bias terms, and task-specific observation
perturbations.  These are backend-independent unless they require backend
sensors to be read first. \\
\midrule
Evaluation and playback & Same environment contract as training unless the
configuration is changed & Training/evaluation entrypoint and task config &
The backend does not reinterpret randomization for evaluation; training and
evaluation share the same environment contract to avoid implicit behavioral
differences between the two modes.  Deterministic runs should disable the
relevant task switches or set degenerate ranges and fixed seeds. \\
\bottomrule
\end{tabular}
\caption{Domain-randomization lifecycle used by the current \method{} runtime.}
\label{tab:app_dr_lifecycle}
\end{table*}

\subsection{Backend Implementation}
\label{app:dr_backend_implementation}

\noindent\textbf{MuJoCoUni.}
% MuJoCoUni 遵循 MuJoCoUni 参考文稿中的 reset-lifecycle 设计：
% \texttt{BatchEnvPool.reset(env\_ids, initial\_state, randomization=None)} 同时接收新的 physics state 和可选的 model-field patch 字典。
% 每个 payload 的首维都是 \texttt{len(env\_ids)}，因此 reset 成本和随机化工作量随实际终止环境数缩放。
% 影响 MuJoCo 派生常量的字段会先 patch 再通过 \texttt{mj\_setConst} 刷新，其他字段直接写入并进入 reset/forward 路径。
% 几何级变化在 runtime execution 前通过编译兼容模型变体并给每个 vectorized environment 分配变体来表达。
MuJoCoUni implements reset-time randomization through
\texttt{BatchEnvPool.reset(env\_ids, initial\_state, randomization=None)}
which receives both the new physics state and an optional dictionary of model-field
patches.  Each payload has leading dimension \texttt{len(env\_ids)}, so reset
cost and randomization work scale with the number of environments that actually
terminate.  Fields that affect MuJoCo derived constants are patched before the
reset/forward path and refreshed with \texttt{mj\_setConst}; other fields are
written directly.  Geometry-level changes are handled before runtime execution by
compiling compatible model variants and assigning each vectorized environment
to one variant before the pool is materialized.

\noindent\textbf{MotrixSim.}
% MotrixSim 通过 MotrixSim 原生 override API 实现同一个 task/backend contract。
% 在 \texttt{set\_state} 中，后端 reset 被选中的 data slice，清除这些环境上暂存的 body force，应用 init-time geometry-size override，再应用支持的 reset randomization，随后写入新的 DOF state 并执行 forward kinematics。
% mass 和 COM 随机化使用 link mass 与 center-of-mass override。
% friction、gravity 和 actuator-gain randomization 是条件能力：只有加载的 MotrixSim model 暴露对应 override method 时才启用，并且 gain randomization 要求所有 actuator 都是 position actuator。
% object 或 geom-size 变体通过每环境 size override 表达，而不是通过独立的 MuJoCo model binary。
MotrixSim implements the same task/backend contract with MotrixSim-native
override APIs.  During \texttt{set\_state}, the backend resets the selected data
slice, clears staged body forces for those environments, applies init-time
geometry-size overrides, applies supported reset randomization, writes the new
DOF state, and runs forward kinematics.  Mass and COM randomization use link
mass and center-of-mass overrides.  Friction, gravity, and actuator-gain
randomization are conditional capabilities: they are enabled only when the
loaded MotrixSim model exposes the corresponding override methods, and
gain randomization requires all actuators to be position actuators.  Object or
geom-size variants are represented as per-environment size overrides rather
than separate MuJoCo model binaries.

\subsection{Supported Randomization Families}
\label{app:dr_supported_families}

% 表格~\ref{tab:app_dr_backend_capabilities} 汇总后端能力和当前任务侧覆盖范围。
% 表格刻意区分“后端能否应用某个字段”和“某个任务配置是否启用了该字段”。
% 当任务请求后端不支持的 reset term 时，manager 会过滤不支持的 reset payload entry 并记录日志；部分任务 provider 如果认为该 term 对 workload 必需，也会在 validate 阶段直接失败。
Table~\ref{tab:app_dr_backend_capabilities} lists backend capabilities and
current task-side coverage.  The table distinguishes a backend's ability to
apply a field from whether a particular task configuration enables that field.
When a task requests reset terms that a backend does not support, the manager
filters unsupported reset payload entries and logs the skipped terms; some task
providers additionally fail validation when the term is required for that
workload.

\begin{table*}[t]
\centering
\scriptsize
\captionsetup{hypcap=false}

\setlength{\tabcolsep}{3pt}
\begin{tabular}{@{}
>{\raggedright\hyphenpenalty=10000\exhyphenpenalty=10000\arraybackslash}p{0.13\textwidth}
>{\raggedright\hyphenpenalty=10000\exhyphenpenalty=10000\arraybackslash}p{0.08\textwidth}
>{\raggedright\hyphenpenalty=10000\exhyphenpenalty=10000\arraybackslash}p{0.18\textwidth}
>{\raggedright\hyphenpenalty=10000\exhyphenpenalty=10000\arraybackslash}p{0.18\textwidth}
>{\raggedright\hyphenpenalty=10000\exhyphenpenalty=10000\arraybackslash}p{0.31\textwidth}@{}}
\toprule
\textbf{Family} & \textbf{Lifecycle} & \textbf{MuJoCoUni} & \textbf{MotrixSim} & \textbf{Current task coverage} \\
\midrule
Model or geometry variants & Init & Precompiled \texttt{MjModel} variants
with per-env assignments. & Per-env geometry-size overrides applied to the
MotrixSim data/model path. & Sharpa in-hand object-scale variants. \\
\midrule
Initial state and task conditions & Reset & Backend receives the sampled
\texttt{qpos}/\texttt{qvel}; task provider owns pose, velocity, command, grasp,
motion-frame, and terrain-spawn sampling. & Same task-level reset contract
after conversion to MotrixSim DOF layout. & Locomotion commands and spawn pose;
motion-tracking reference frames; in-hand grasp/object resets. \\
\midrule
Base/body mass & Reset & \texttt{base\_mass\_delta} and full
\texttt{body\_mass}. & Base-link mass delta and full link-mass override. &
Locomotion, manipulation-locomotion, motion tracking, and dexterous-hand tasks
where config enables mass DR. \\
\midrule
Base/body COM & Reset & \texttt{base\_com\_offset} and full
\texttt{body\_ipos}. & Base-link COM offset and full link COM override. &
Locomotion, motion tracking, and hand/object tasks where config enables COM
DR. \\
\midrule
Gravity & Reset & \texttt{gravity} payload. & Conditional gravity override
support. & Motion-tracking and dexterous-hand
configs that enable gravity or gravity-direction DR. \\
\midrule
Contact friction & Reset & Full \texttt{geom\_friction} payload. &
Conditional collision-geom friction overrides; non-collision geoms must remain
at defaults because the MotrixSim friction override API is only exposed on
geoms with nonzero collision group or affinity. & Ground friction in manipulation-locomotion; foot friction in G1
tracking; object friction in dexterous-hand tasks. \\
\midrule
Actuator gains & Reset & \texttt{kp} and \texttt{kd} payloads for position
actuators. & Conditional per-actuator Kp/damping overrides; available only for
all-position-actuator models. & Go2/G1 locomotion and tracking tasks when
\texttt{randomize\_kp} or \texttt{randomize\_kd} is enabled. \\
\midrule
Inertia and armature & Reset & \texttt{body\_iquat},
\texttt{body\_inertia}, and \texttt{dof\_armature}. & Not advertised in the
current capability set. & Armature randomization is used by
manipulation-locomotion configs when enabled; body inertial tensors are backend
capability rather than broad task coverage. \\
\midrule
External perturbations & Interval & Push and arbitrary body-force payloads are
staged through \texttt{xfrc\_applied}. & Push forces are supported through link
external force; arbitrary body force is conditional on link
\texttt{add\_external\_force}. & Locomotion push perturbations; Sharpa object
force perturbations. \\
\midrule
Observation noise and biases & Observation step or reset & Task-side NumPy
noise after backend sensor reads. & Same task-side path. & Locomotion actor
noise; G1 tracking actor noise and reset biases; hand joint/contact observation
noise where configured. \\
\bottomrule
\end{tabular}
\caption{Supported domain-randomization families and backend-specific limits.}
\label{tab:app_dr_backend_capabilities}
\end{table*}

\subsection{Implications for Cross-Backend Experiments}
\label{app:dr_cross_backend_implications}

% 共享契约让任务可以用同一套接口表达随机化，但实际生效的随机化集合仍然依赖后端。
% 因此在跨后端实验中，我们需要把 resolved task configuration 和 backend capabilities 分开报告。
% 只有当任务配置启用某个随机化项，并且所选后端声明支持对应字段时，该随机化项才应被解释为 active。
% 这一区分对公平比较很重要：例如 MuJoCoUni 暴露更宽的 inertial reset-field surface，而 MotrixSim 在加载模型支持对应 override API 时，可以通过 link、geom、gravity、actuator 和 external-force override 匹配许多常见 locomotion 与 manipulation 设置。
The shared contract lets a task express randomization once, but the effective
randomization set is still backend-dependent.  For cross-backend experiments,
we therefore report the resolved task configuration separately from backend
capabilities.  A randomization item should be interpreted as active only when
the task configuration enables it and the selected backend advertises support
for the corresponding field.  This distinction matters for fair comparison:
for example, MuJoCoUni exposes a wider reset-field surface for inertial fields,
whereas MotrixSim can match many common locomotion and manipulation settings
through link, geom, gravity, actuator, and external-force override APIs when
the loaded model supports them.

\section{Task and Algorithm Details}
\label{app:training_curves}

\subsection{Training Curves}
\label{app:training_curves_figures}

This subsection collects per-task training curves for the three on-policy and off-policy algorithm families used in the main paper. Each panel plots episode reward against environment steps; the curves are aggregated over seeds and smoothed with a fixed-width moving average. Rewards use the same task-side scales as in Section~\ref{app:training_curves_tasks}, so absolute values are comparable across seeds for the same task but not across tasks. The task subsets shown for each algorithm match the per-task override tables in Section~\ref{app:training_curves_algorithms}: PPO is reported on all sixteen benchmark tasks, APPO on the six tasks with a registered APPO configuration, and SAC / FlashSAC on the five tasks with a replay configuration.

\begin{figure}[H]
    \centering
    \includegraphics[width=0.95\textwidth]{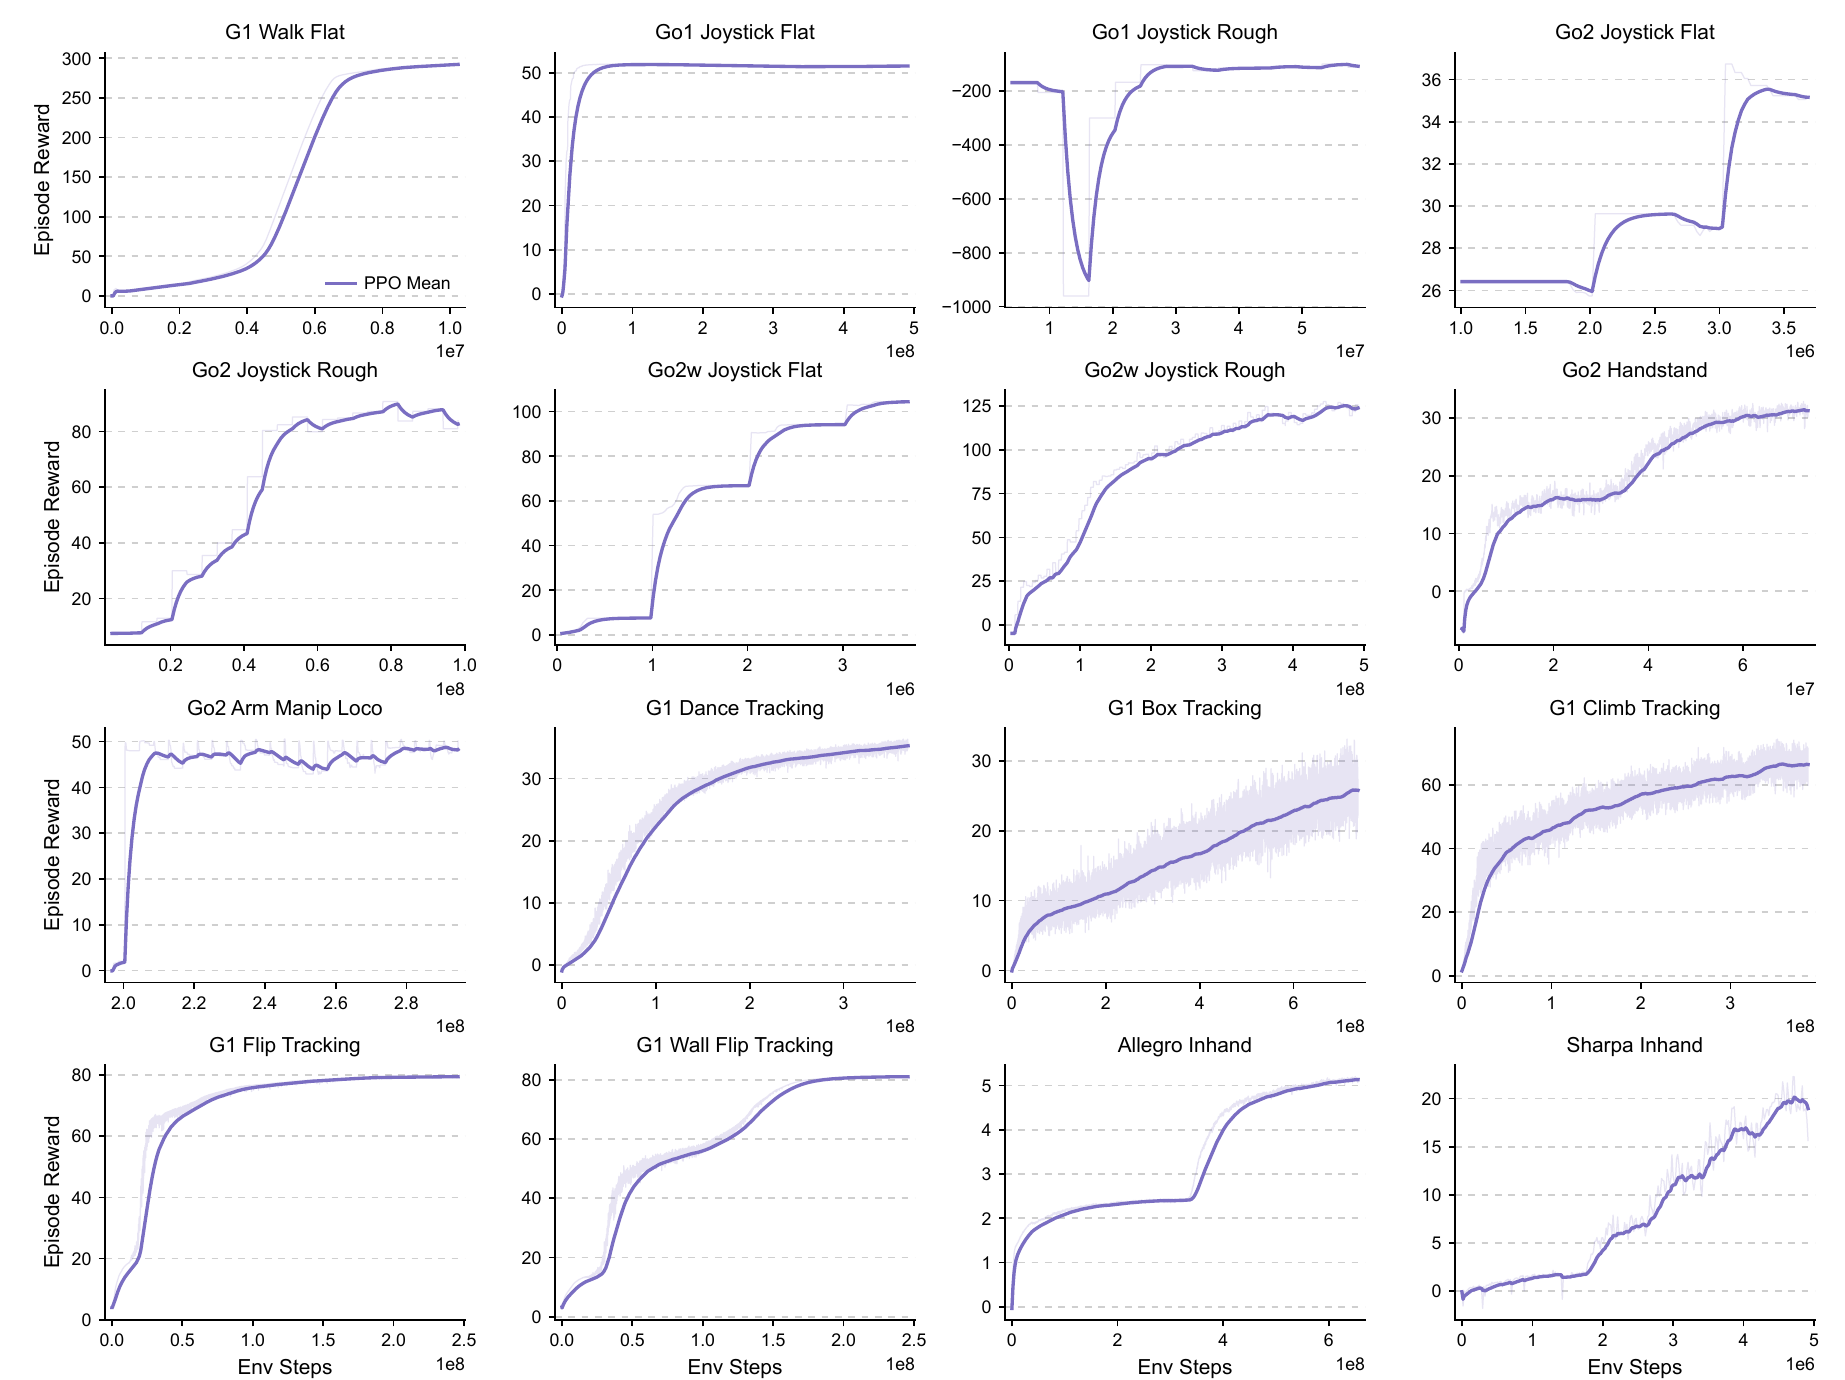}
    \caption{PPO training curves across the sixteen benchmark tasks. Each panel reports episode reward against environment steps; the $x$-axis units differ per panel because environment-step budgets are task-dependent (see Section~\ref{app:training_curves_algorithms}).}
    \label{fig:app_ppo_task_grid}
\end{figure}

\begin{figure}[H]
    \centering
    \includegraphics[width=0.95\textwidth]{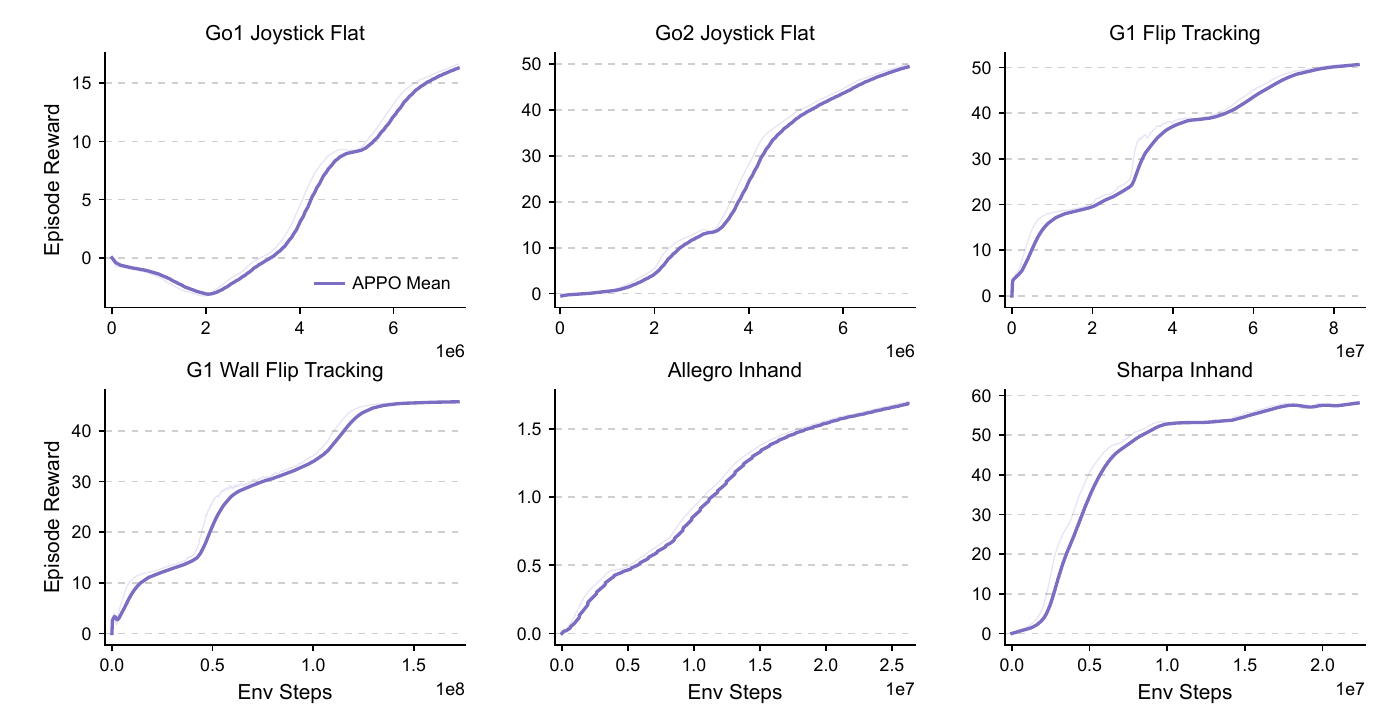}
    \caption{APPO training curves for the six tasks with a registered APPO configuration: Go1 / Go2 Joystick Flat, G1 Flip and Wall Flip Tracking, Allegro Inhand, and Sharpa Inhand (HORA teacher).}
    \label{fig:app_appo_task_grid}
\end{figure}

\begin{figure}[H]
    \centering
    \includegraphics[width=0.95\textwidth]{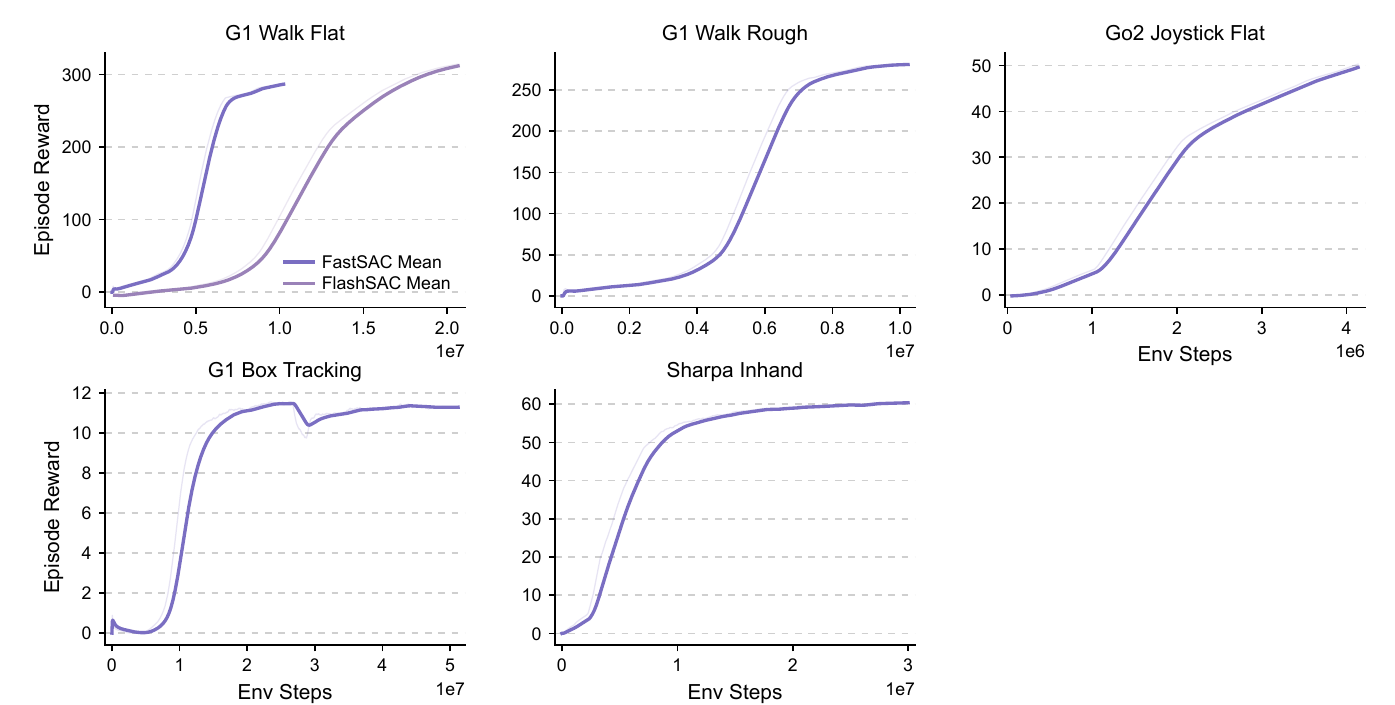}
    \caption{FastSAC and FlashSAC training curves for the five tasks with a replay configuration. G1 Walk Flat reports both FastSAC and FlashSAC; the remaining four tasks (G1 Walk Rough, Go2 Joystick Flat, G1 Box Tracking, Sharpa Inhand) report FastSAC only.}
    \label{fig:app_sac_task_grid}
\end{figure}

\subsection{Bidirectional Sim2Sim Cross-Backend Validation}
\label{app:sim2sim_cross_validation}

\paragraph{Objective.}
This subsection evaluates whether a policy trained against one simulation backend transfers to the other without retraining. We rollout each checkpoint on both MuJoCoUni and MotrixSim and compare its behaviour. Because each task uses backend-specific reward shaping at training time, the absolute reward values from different training backends are not directly comparable; what is meaningful is the change of each metric when the same policy is moved between backends, since this isolates the gap introduced by the simulator rather than by the policy.

\paragraph{Metrics.}
We report three quantities per (policy, evaluation-backend) pair:
\begin{itemize}
    \item \textbf{Mean episodic return:} the mean cumulative reward over 100 evaluation episodes, computed with the reward scale stored with the checkpoint at training time.
    \item \textbf{Success rate:} the fraction of the 100 episodes that finish without early termination.
    \item \textbf{MPJPE (m):} the mean per-joint position error against the reference trajectory, averaged over time and joints. MPJPE is only defined for motion-tracking tasks; locomotion rows report a dash.
\end{itemize}

\paragraph{Protocol.}
All numbers come from zero-shot rollouts of a single trained checkpoint per policy: no fine-tuning, no retraining, and no per-backend adaptation. For each task we evaluate two checkpoints---one trained on MuJoCoUni and one trained on MotrixSim---and run each checkpoint on both backends, yielding four rows per task. The native rows (train backend $=$ test backend) act as the reference; the cross rows (train backend $\ne$ test backend) measure the sim2sim gap. Each cell aggregates 100 episodes. Cross-backend evaluation uses the reward weights and normalization constants associated with the policy's training backend, ensuring that changes reflect simulator transfer rather than reward-definition changes.

\begin{table}[!htbp]
    \centering
    \small
    \caption{Bidirectional sim2sim cross-backend evaluation. For each task, the four rows correspond to: native MotrixSim (train$=$test$=$MotrixSim), forward transfer (MotrixSim$\to$MuJoCoUni), native MuJoCoUni (train$=$test$=$MuJoCoUni), and reverse transfer (MuJoCoUni$\to$MotrixSim). Mean return is comparable only within the four rows of a single task: reward scales are task- and training-backend-specific. A dash in the MPJPE column marks locomotion rows, where no reference trajectory exists.}
    \label{tab:app_sim2sim_cross}
    \resizebox{\textwidth}{!}{%
    \begin{tabular}{@{}llllcccc@{}}
        \toprule
        Test type & Task & Train backend & Test backend & Mean return & Success & MPJPE\,(m) & Episodes \\
        \midrule
        \multicolumn{8}{l}{\emph{G1 Walk Flat (SAC)}} \\
        Native      & G1 Walk Flat       & MotrixSim & MotrixSim & 408.38 & 1.00 & --- & 100 \\
        Forward     & G1 Walk Flat       & MotrixSim & MuJoCoUni & 405.46 & 1.00 & --- & 100 \\
        Native      & G1 Walk Flat       & MuJoCoUni & MuJoCoUni & 354.41 & 1.00 & --- & 100 \\
        Reverse     & G1 Walk Flat       & MuJoCoUni & MotrixSim & 354.00 & 1.00 & --- & 100 \\
        \midrule
        \multicolumn{8}{l}{\emph{G1 Motion Tracking, dance reference (SAC)}} \\
        Native      & G1 Motion Tracking & MotrixSim & MotrixSim & 45.26 & 1.00 & 0.0217 & 100 \\
        Forward     & G1 Motion Tracking & MotrixSim & MuJoCoUni & 45.17 & 1.00 & 0.0219 & 100 \\
        Native      & G1 Motion Tracking & MuJoCoUni & MuJoCoUni & 45.36 & 1.00 & 0.0197 & 100 \\
        Reverse     & G1 Motion Tracking & MuJoCoUni & MotrixSim & 45.34 & 1.00 & 0.0204 & 100 \\
        \midrule
        \multicolumn{8}{l}{\emph{G1 Shuttle-Run Tracking (PPO)}} \\
        Native      & G1 Shuttle-Run     & MotrixSim & MotrixSim & 45.80 & 1.00 & 0.0515 & 100 \\
        Forward     & G1 Shuttle-Run     & MotrixSim & MuJoCoUni & 42.28 & 0.92 & 0.0568 & 100 \\
        Native      & G1 Shuttle-Run     & MuJoCoUni & MuJoCoUni & 32.64 & 0.97 & 0.0519 & 100 \\
        Reverse     & G1 Shuttle-Run     & MuJoCoUni & MotrixSim & 31.95 & 0.91 & 0.0532 & 100 \\
        \midrule
        \multicolumn{8}{l}{\emph{G1 Wall Flip Tracking (PPO)}} \\
        Native      & G1 Wall Flip       & MotrixSim & MotrixSim & 84.46 & 1.00 & 0.0447 & 100 \\
        Forward     & G1 Wall Flip       & MotrixSim & MuJoCoUni & 79.46 & 1.00 & 0.0596 & 100 \\
        Native      & G1 Wall Flip       & MuJoCoUni & MuJoCoUni & 80.61 & 1.00 & 0.0431 & 100 \\
        Reverse     & G1 Wall Flip       & MuJoCoUni & MotrixSim & 77.44 & 1.00 & 0.0620 & 100 \\
        \bottomrule
    \end{tabular}}
\end{table}

Across the four tasks, success rate stays at 1.00 for both locomotion and the two acyclic tracking tasks (dance and wall flip); only the shuttle-run policies drop noticeably (0.97/1.00 native vs.\ 0.92/0.91 cross), and MPJPE remains within $0.0030$\,m of the native baseline for the dance clip, within $0.0053$\,m for the shuttle run, and within $0.0189$\,m for the wall flip. These margins are small relative to the per-joint reference scale and indicate that the policies generalize across the two backends without backend-specific adaptation.

\subsection{Task Specifications}
\label{app:training_curves_tasks}

This subsection lists the per-task observation space, action space, command and termination logic, domain randomization, and reward weights for every task evaluated in the main paper. Tasks are grouped by family: locomotion, motion tracking, manipulation-locomotion, and dexterous-hand in-hand manipulation. When MuJoCoUni and MotrixSim share a value it is reported once; backend-specific differences are called out explicitly.

\subsubsection{Locomotion}
\label{app:task_locomotion}

\paragraph{Go1 Joystick Flat.}
\texttt{Go1JoystickFlat} runs on the flat Go1 scene with simulation step $\Delta t_{\mathrm{sim}}=0.01$\,s, control step $\Delta t_{\mathrm{ctrl}}=0.02$\,s, maximum episode 20\,s, and initial base position $(0,0,0.34)$.

\noindent\textbf{Observation space.}
The actor observation is 49-dimensional:
\begin{equation}
    o_t = [\omega_t,\,-g_t,\,q_t-q_{\mathrm{default}},\,\dot q_t,\,a_{t-1},\,c_t,\,\phi_t],
\end{equation}
where $\omega_t\in\mathbb{R}^3$ is the body-frame gyro, $g_t\in\mathbb{R}^3$ is the up-vector sensor, $q_t-q_{\mathrm{default}}\in\mathbb{R}^{12}$ is the joint-position offset, $\dot q_t\in\mathbb{R}^{12}$ is joint velocity, $a_{t-1}\in\mathbb{R}^{12}$ is the previous action, $c_t\in\mathbb{R}^3$ is the velocity command, and $\phi_t\in\mathbb{R}^4$ is the four-leg gait phase. The critic observation appends local linear velocity, giving 52 dimensions.

\noindent\textbf{Action space.}
The action is a 12-dimensional joint-position offset. The environment maps policy output $a_t$ to actuator targets by $q^{\mathrm{cmd}}_t = q_{\mathrm{default}} + 0.25\,a_t$, using PD gains $K_p=35.0$, $K_d=0.5$.

\noindent\textbf{Commands and termination.}
The velocity-command range is $[(-0.6,-0.4,-0.8),(1.0,0.4,0.8)]$. An episode terminates early when the up-vector $z$ component satisfies $g^z_t \le 0.5$. Gait frequency is 2\,Hz.

\noindent\textbf{Domain randomization.}
Reset-time domain randomization is applied as listed in Table~\ref{tab:app_go1flat_backend_task_values}.

\begin{table}[!htbp]
    \centering
    \caption{Domain randomization for \texttt{go1\_joystick\_flat}.}
    \label{tab:app_go1flat_backend_task_values}
    \begin{tabular}{@{}lc@{}}
        \toprule
        Item & MuJoCoUni \\
        \midrule
        Velocity-command range & $[(-0.6,-0.4,-0.8),(1.0,0.4,0.8)]$ \\
        \texttt{randomize\_kp} & true (default) \\
        \texttt{randomize\_kd} & true (default) \\
        Kp/Kd multiplier range & $[0.9,1.1]$ \\
        \bottomrule
    \end{tabular}
\end{table}

\noindent\textbf{Reward design.}
The reward is $\Delta t_{\mathrm{ctrl}}\sum_i w_i r_i$. Table~\ref{tab:app_go1flat_reward} lists the active reward scales.

\begin{table}[!htbp]
    \centering
    \caption{Reward terms for \texttt{go1\_joystick\_flat}.}
    \label{tab:app_go1flat_reward}
    \begin{tabular}{@{}lc@{}}
        \toprule
        Term & MuJoCoUni \\
        \midrule
        Linear velocity tracking & 1.0 \\
        Yaw angular velocity tracking & 0.2 \\
        Vertical linear velocity & -5.0 \\
        Roll/pitch angular velocity & -0.1 \\
        Base height & -100.0 \\
        Action rate & -0.005 \\
        Joint deviation from default & -0.1 \\
        Contact phase agreement & 0.24 \\
        Swing-foot height & 4.0 \\
        \bottomrule
    \end{tabular}
\end{table}

The velocity-tracking terms use $\exp(-e^2/\sigma^2)$ with $\sigma=0.25$; the base-height penalty uses a target of $0.3$\,m; the swing-foot term uses $\exp(-e_z^2/0.01)$ gated by the swing phase ($\phi_i \ge 0.6$).

\paragraph{Go1 Joystick Rough.}
\texttt{Go1JoystickRough} adds procedurally generated terrain to the Go1 quadruped. The configuration is identical across the two backends. Simulation step $\Delta t_{\mathrm{sim}}=0.01$\,s, control step $\Delta t_{\mathrm{ctrl}}=0.02$\,s, maximum episode 20\,s.

\noindent\textbf{Observation space.}
The actor observation is 45-dimensional (policy group):
\begin{equation}
    o_t = [0.25\omega_t,\,-g_t,\,c_t,\,q_t-q_{\mathrm{default}},\,0.05\dot q_t,\,a_{t-1}],
\end{equation}
where gyro and joint velocity are pre-scaled. The critic observation is 48-dimensional (adds base linear velocity) plus a height-scan vector (default 187 points from an $11\times17$ grid around the robot base).

\noindent\textbf{Action space.}
The action is 12-dimensional with per-joint scaling: hip joints use \texttt{hip\_action\_scale}$=0.125$, non-hip joints use \texttt{non\_hip\_action\_scale}$=0.25$. PD gains $K_p=35.0$, $K_d=0.5$. Actions are clipped to $[-100, 100]$.

\noindent\textbf{Commands and termination.}
The velocity-command range is $[(-1,-1,-1),(1,1,1)]$ with heading command enabled and resampling every 10\,s. Terrain is procedurally generated on an $8\times8$\,m cell grid ($6\times6$ cells, border width 20\,m). Termination occurs when the robot moves more than 3\,m beyond its terrain cell boundary. No gravity-based termination is used.

\noindent\textbf{Domain randomization.}
Reset-time domain randomization is listed in Table~\ref{tab:app_go1rough_dr}.

\begin{table}[!htbp]
    \centering
    \caption{Domain randomization for \texttt{go1\_joystick\_rough}.}
    \label{tab:app_go1rough_dr}
    \begin{tabular}{@{}lcc@{}}
        \toprule
        Item & MuJoCoUni & MotrixSim \\
        \midrule
        \texttt{randomize\_base\_mass} & true & true \\
        Added mass range & $[-1.0, 3.0]$ & $[-1.0, 3.0]$ \\
        \texttt{random\_com} & true & true \\
        \texttt{randomize\_kp} & true & true \\
        Kp multiplier range & $[0.5, 2.0]$ & $[0.5, 2.0]$ \\
        \texttt{randomize\_kd} & true & true \\
        Kd multiplier range & $[0.5, 2.0]$ & $[0.5, 2.0]$ \\
        \texttt{push\_robots} & true & true \\
        Push interval (steps) & 625 & 625 \\
        Max push force & $[1.0, 1.0, 0.5]$ & $[1.0, 1.0, 0.5]$ \\
        \bottomrule
    \end{tabular}
\end{table}

\noindent\textbf{Reward design.}
Table~\ref{tab:app_go1rough_reward} lists the active reward scales.

\begin{table}[!htbp]
    \centering
    \caption{Reward terms for \texttt{go1\_joystick\_rough}.}
    \label{tab:app_go1rough_reward}
    \small
    \begin{tabular}{@{}lcc@{}}
        \toprule
        Term & MuJoCoUni & MotrixSim \\
        \midrule
        Linear velocity tracking & 3.0 & 3.0 \\
        Yaw angular velocity tracking & 1.5 & 1.5 \\
        Vertical linear velocity & -2.0 & -2.0 \\
        Roll/pitch angular velocity & -0.05 & -0.05 \\
        Joint torques L2 & $-2.5{\times}10^{-5}$ & $-2.5{\times}10^{-5}$ \\
        Joint acceleration L2 & $-2.5{\times}10^{-7}$ & $-2.5{\times}10^{-7}$ \\
        Joint position limits & -5.0 & -5.0 \\
        Joint power & $-2.0{\times}10^{-5}$ & $-2.0{\times}10^{-5}$ \\
        Stand still & -2.0 & -2.0 \\
        Hip position & -0.5 & -0.5 \\
        Joint position penalty & -1.0 & -1.0 \\
        Joint mirror & -0.05 & -0.05 \\
        Action rate & -0.01 & -0.01 \\
        Undesired contacts & -1.0 & -1.0 \\
        Contact forces & $-1.5{\times}10^{-4}$ & $-1.5{\times}10^{-4}$ \\
        Feet air time & 0.5 & 0.5 \\
        Feet air time variance & -1.0 & -1.0 \\
        Feet contact without cmd & 0.1 & 0.1 \\
        Feet slide & -0.1 & -0.1 \\
        Feet height body & -5.0 & -5.0 \\
        Feet gait & 0.5 & 0.5 \\
        Upward & 1.0 & 1.0 \\
        \bottomrule
    \end{tabular}
\end{table}

Tracking-style terms use $\sigma=0.25$ and the base-height penalty uses a target of $0.33$\,m on both backends.

\paragraph{Go2 Joystick Flat.}
\texttt{Go2JoystickFlat} runs on the flat Go2 scene with simulation step $\Delta t_{\mathrm{sim}}=0.01$\,s, control step $\Delta t_{\mathrm{ctrl}}=0.02$\,s, maximum episode 20\,s, and initial base position $(0,0,0.42)$.

\noindent\textbf{Observation space.}
The actor observation is 49-dimensional:
\begin{equation}
    o_t = [\omega_t,\,-g_t,\,q_t-q_{\mathrm{default}},\,\dot q_t,\,a_{t-1},\,c_t,\,\phi_t],
\end{equation}
where $\omega_t\in\mathbb{R}^3$ is the body-frame gyro reading, $g_t\in\mathbb{R}^3$ is the up-vector sensor value, $q_t-q_{\mathrm{default}}\in\mathbb{R}^{12}$ is the joint-position offset from the default pose, $\dot q_t\in\mathbb{R}^{12}$ is joint velocity, $a_{t-1}\in\mathbb{R}^{12}$ is the previous action, $c_t\in\mathbb{R}^3$ is the velocity command, and $\phi_t\in\mathbb{R}^4$ is the foot phase. The critic observation appends local linear velocity, giving a 52-dimensional privileged observation. Observation noise uses the default level.

\noindent\textbf{Action space.}
The action is a 12-dimensional joint-position command offset. The environment maps policy output $a_t$ to actuator targets by
\begin{equation}
    q^{\mathrm{cmd}}_t = q_{\mathrm{default}} + 0.25 a_t,
\end{equation}
using the shared Go2 PD gains $K_p=35.0$ and $K_d=0.5$.

\noindent\textbf{Commands and termination.}
The velocity-command range is $[(-0.6,-0.4,-0.8),(1.0,0.4,0.8)]$. An episode terminates early when the up-vector $z$ component satisfies $g^z_t \le 0.5$.

\noindent\textbf{Domain randomization.}
Reset-time domain randomization is applied as listed in Table~\ref{tab:app_go2_backend_task_values}.

\begin{table}[!htbp]
    \centering
    \caption{Domain randomization for \texttt{go2\_joystick\_flat}.}
    \label{tab:app_go2_backend_task_values}
    \begin{tabular}{@{}lc@{}}
        \toprule
        Item & MuJoCoUni \\
        \midrule
        Velocity-command range & $[(-0.6,-0.4,-0.8),(1.0,0.4,0.8)]$ \\
        \texttt{randomize\_kp} & true \\
        \texttt{randomize\_kd} & true \\
        Kp/Kd multiplier range & $[0.9,1.1]$ \\
        \bottomrule
    \end{tabular}
\end{table}

\noindent\textbf{Reward design.}
The reward is the control-step-scaled sum $\Delta t_{\mathrm{ctrl}}\sum_i w_i r_i$. Table~\ref{tab:app_go2_backend_reward} lists the active reward scales.

\begin{table}[!htbp]
    \centering
    \caption{Reward terms for \texttt{go2\_joystick\_flat}.}
    \label{tab:app_go2_backend_reward}
    \begin{tabular}{@{}lc@{}}
        \toprule
        Term & MuJoCoUni \\
        \midrule
        Linear velocity tracking & 1.0 \\
        Yaw angular velocity tracking & 0.2 \\
        Vertical linear velocity & -5.0 \\
        Roll/pitch angular velocity & -0.1 \\
        Base height & -100.0 \\
        Action rate & -0.005 \\
        Joint deviation from default pose & -0.1 \\
        Contact phase agreement & 0.24 \\
        Swing-foot height & 4.0 \\
        \bottomrule
    \end{tabular}
\end{table}

Tracking-style terms use $\sigma=0.25$ and the base-height penalty uses a target of $0.3$\,m. The swing-foot term rewards swing feet near 0.1\,m height; the contact term compares measured foot contact with the gait phase.

\paragraph{Go2 Joystick Rough.}
\texttt{Go2JoystickRough} shares the same architecture as Go1 Joystick Rough (procedural terrain, height scan, heading command) but uses the Go2 robot model. The configuration is identical across the two backends. Simulation step $\Delta t_{\mathrm{sim}}=0.01$\,s, control step $\Delta t_{\mathrm{ctrl}}=0.02$\,s, maximum episode 20\,s.

\noindent\textbf{Observation space.}
Same structure as Go1 Joystick Rough: actor 45-dimensional (pre-scaled gyro, gravity, command, joint offset, joint velocity, last action), critic 48-dimensional plus height-scan (187 points).

\noindent\textbf{Action space.}
12-dimensional with \texttt{hip\_action\_scale}$=0.125$, \texttt{non\_hip\_action\_scale}$=0.25$. PD gains $K_p=35.0$, $K_d=0.5$. Clip to $[-100, 100]$.

\noindent\textbf{Commands and termination.}
Velocity-command range $[(-1,-1,-1),(1,1,1)]$, heading command enabled, resampling every 10\,s. Terrain: $8\times8$\,m cells, $6\times6$ grid, border 20\,m. Termination: terrain out-of-bounds (3\,m buffer). No gravity-based termination.

\noindent\textbf{Domain randomization.}
Identical to Go1 Joystick Rough (Table~\ref{tab:app_go1rough_dr}): base mass $[-1,3]$\,kg, COM offset, Kp/Kd $[0.5,2.0]$, push robots every 625 steps with force $[1,1,0.5]$.

\noindent\textbf{Reward design.}
Same reward terms and weights as Go1 Joystick Rough (Table~\ref{tab:app_go1rough_reward}), with base-height target $0.33$\,m and tracking sigma $0.25$.

\paragraph{Go2W Joystick Flat.}
\texttt{Go2WJoystickFlat} is a wheeled-legged quadruped with 12 leg joints and 2 wheel joints. The configuration is identical across the two backends. Simulation step $\Delta t_{\mathrm{sim}}=0.01$\,s, control step $\Delta t_{\mathrm{ctrl}}=0.02$\,s, maximum episode 20\,s.

\noindent\textbf{Observation space.}
The actor observation is 53-dimensional:
\begin{equation}
    o_t = [\omega_t,\,-g_t,\,q^{leg}_t{-}q^{leg}_{\mathrm{def}},\,\dot q^{leg}_t,\,\dot q^{wheel}_t,\,a_{t-1},\,c_t],
\end{equation}
where the leg joint offset and velocity are 12-dimensional each, wheel velocity is 2-dimensional, and actions include both leg (12) and wheel (2) outputs. The critic observation is 72-dimensional (adds linear velocity, motor control targets, and wheel control targets).

\noindent\textbf{Action space.}
14-dimensional: 12 leg joints with \texttt{action\_scale}$=0.5$ and 2 wheel joints with \texttt{wheel\_action\_scale}$=10.0$. Leg PD gains $K_p=50.0$, $K_d=1.5$; wheel uses velocity control with $K_d^{wheel}=0.5$.

\noindent\textbf{Commands and termination.}
Velocity-command range $[(0,0,-1),(1,0,1)]$ (forward and yaw only). An episode terminates early when $g^z_t \le 0.5$.

\noindent\textbf{Domain randomization.}
Kp/Kd randomization is disabled. No other domain randomization is enabled in the flat variant.

\noindent\textbf{Reward design.}
Table~\ref{tab:app_go2wflat_reward} lists the active reward scales.

\begin{table}[!htbp]
    \centering
    \caption{Reward terms for \texttt{go2w\_joystick\_flat}.}
    \label{tab:app_go2wflat_reward}
    \begin{tabular}{@{}lcc@{}}
        \toprule
        Term & MuJoCoUni & MotrixSim \\
        \midrule
        Linear velocity tracking & 1.0 & 1.0 \\
        Yaw angular velocity tracking & 0.75 & 0.75 \\
        Vertical linear velocity & -5.0 & -5.0 \\
        Roll/pitch angular velocity & -0.1 & -0.1 \\
        Base height & -100.0 & -100.0 \\
        Orientation & -2.0 & -2.0 \\
        Action rate & -0.005 & -0.005 \\
        Joint deviation from default & -0.5 & -0.5 \\
        Torques & $-2.0{\times}10^{-4}$ & $-2.0{\times}10^{-4}$ \\
        Alive & 0.5 & 0.5 \\
        Upward & 1.0 & 1.0 \\
        \bottomrule
    \end{tabular}
\end{table}

Tracking-style terms use $\sigma=0.25$ and the base-height penalty uses a target of $0.4$\,m on both backends.

\paragraph{Go2W Joystick Rough.}
\texttt{Go2WJoystickRough} adds procedural terrain to the wheeled-legged Go2W. Simulation step $\Delta t_{\mathrm{sim}}=0.01$\,s, control step $\Delta t_{\mathrm{ctrl}}=0.02$\,s, maximum episode 20\,s.

\noindent\textbf{Observation space.}
The actor observation is 53-dimensional (pre-scaled gyro $0.25\omega$, gravity, command, leg joint offset, leg velocity $0.05\dot q$, last action including wheel). The critic observation is 56-dimensional (adds linear velocity) plus height-scan (187 points).

\noindent\textbf{Action space.}
14-dimensional: 12 leg joints with \texttt{action\_scale}$=0.5$ and 2 wheel joints with \texttt{wheel\_action\_scale}$=10.0$. Leg PD gains $K_p=35.0$, $K_d=0.5$; wheel $K_d^{wheel}=0.5$. Clip to $[-100, 100]$.

\noindent\textbf{Commands and termination.}
Velocity-command range $[(-1,-1,-1),(1,1,1)]$, heading command enabled, resampling every 10\,s. Terrain: $8\times8$\,m cells, $6\times6$ grid, border 20\,m. Termination: terrain out-of-bounds (3\,m buffer).

\noindent\textbf{Domain randomization.}
Table~\ref{tab:app_go2wrough_dr} lists the domain-randomization settings. Kp/Kd randomization is enabled under MotrixSim and disabled under MuJoCoUni.

\begin{table}[!htbp]
    \centering
    \caption{Domain randomization for \texttt{go2w\_joystick\_rough}.}
    \label{tab:app_go2wrough_dr}
    \begin{tabular}{@{}lcc@{}}
        \toprule
        Item & MuJoCoUni & MotrixSim \\
        \midrule
        \texttt{randomize\_base\_mass} & true & true \\
        Added mass range & $[-1.0, 3.0]$ & $[-1.0, 3.0]$ \\
        \texttt{random\_com} & true & true \\
        COM offset x & $[-0.05, 0.05]$ & $[-0.05, 0.05]$ \\
        \texttt{randomize\_kp} & false & true \\
        Kp multiplier range & $[0.5, 1.0]$ & $[0.5, 1.0]$ \\
        \texttt{randomize\_kd} & false & true \\
        Kd multiplier range & $[0.5, 1.0]$ & $[0.5, 1.0]$ \\
        \texttt{push\_robots} & true & true \\
        Push interval (steps) & 500 & 625 \\
        Max push force & $[0.5, 0.5, 0.0]$ & $[1.0, 1.0, 0.5]$ \\
        Push body & \texttt{base\_link} & \texttt{base\_link} \\
        \bottomrule
    \end{tabular}
\end{table}

\noindent\textbf{Reward design.}
Table~\ref{tab:app_go2wrough_reward} lists the active reward scales. MotrixSim adds an orientation penalty that MuJoCoUni does not use, and the two backends differ on the hip-position penalty weight.

\begin{table}[!htbp]
    \centering
    \caption{Reward terms for \texttt{go2w\_joystick\_rough}.}
    \label{tab:app_go2wrough_reward}
    \small
    \begin{tabular}{@{}lcc@{}}
        \toprule
        Term & MuJoCoUni & MotrixSim \\
        \midrule
        Linear velocity tracking & 3.0 & 3.0 \\
        Yaw angular velocity tracking & 1.5 & 1.5 \\
        Vertical linear velocity & -2.0 & -2.0 \\
        Roll/pitch angular velocity & -0.05 & -0.05 \\
        Orientation & / & -2.0 \\
        Joint torques L2 & $-2.5{\times}10^{-5}$ & $-2.5{\times}10^{-5}$ \\
        Joint acceleration L2 & $-2.5{\times}10^{-7}$ & $-2.5{\times}10^{-7}$ \\
        Wheel-joint acceleration L2 & $-2.5{\times}10^{-9}$ & $-2.5{\times}10^{-9}$ \\
        Joint position limits & -5.0 & -5.0 \\
        Joint power & $-2.0{\times}10^{-5}$ & $-2.0{\times}10^{-5}$ \\
        Action rate & -0.01 & -0.01 \\
        Stand still & -2.0 & -2.0 \\
        Hip position & -2.0 & -0.5 \\
        Joint position penalty & -1.0 & -1.0 \\
        Joint mirror & -0.05 & -0.05 \\
        Upward & 1.0 & 1.0 \\
        \bottomrule
    \end{tabular}
\end{table}

Tracking-style terms use $\sigma=0.25$ and the base-height penalty uses a target of $0.4$\,m on both backends.

\paragraph{G1 Walk Flat.}
\texttt{G1WalkFlat} is a 29-DOF humanoid locomotion task on the flat G1 scene. Simulation step $\Delta t_{\mathrm{sim}}=0.01$\,s, control step $\Delta t_{\mathrm{ctrl}}=0.02$\,s, maximum episode 20\,s, initial base position $(0,0,0.754)$.

\noindent\textbf{Observation space.}
The actor observation is 98-dimensional:
\begin{equation}
    o_t = [\omega_t,\,-g_t,\,q_t-q_{\mathrm{default}},\,\dot q_t,\,a_{t-1},\,c_t,\,\phi_t],
\end{equation}
where joint offset, joint velocity, and last action are 29-dimensional each, and $\phi_t\in\mathbb{R}^2$ is the bipedal gait phase (left, right). The critic observation is 101-dimensional (adds base linear velocity).

\noindent\textbf{Action space.}
29-dimensional joint-position offset. Action mapping $q^{\mathrm{cmd}}_t = q_{\mathrm{default}} + s\,a_t$ with backend-dependent scale: MuJoCoUni uses $s=0.25$, MotrixSim uses $s=0.5$. PD gains $K_p=50.0$, $K_d=1.0$ (from G1 base config).

\noindent\textbf{Commands and termination.}
Under MuJoCoUni the velocity-command range follows the task default; under MotrixSim it is fixed to $[(0.4,0,0),(0.7,0,0)]$ (forward walking only) with the gait phase initialized at the configured offset and the reset base-velocity limited to $0.05$\,m/s. Termination occurs when body tilt exceeds the configured maximum or the base height drops below the configured minimum: MuJoCoUni uses $25^\circ$ and $0.55$\,m, MotrixSim uses $35^\circ$ and $0.5$\,m.

\noindent\textbf{Domain randomization.}
The velocity curriculum is disabled. Under MotrixSim Kp/Kd randomization is additionally disabled. Observation noise is configured identically on both backends: noise level $1.0$, joint-angle scale $0.01$, joint-velocity scale $1.5$, gyro scale $0.2$.

\noindent\textbf{Reward design.}
Table~\ref{tab:app_g1walkflat_reward} lists the active reward scales. MotrixSim introduces several gait-shaping terms (feet phase contrast, feet phase contact, double-stance penalty, under-speed penalty, upper-body pose) that are not used under MuJoCoUni.

\begin{table}[!htbp]
    \centering
    \caption{Reward terms for \texttt{g1\_walk\_flat}.}
    \label{tab:app_g1walkflat_reward}
    \small
    \begin{tabular}{@{}lcc@{}}
        \toprule
        Term & MuJoCoUni & MotrixSim \\
        \midrule
        Linear velocity tracking & 2.0 & 2.0 \\
        Yaw angular velocity tracking & 0.2 & 0.25 \\
        Feet phase & 1.0 & 1.2 \\
        Feet phase contrast & / & 1.5 \\
        Feet phase contact & / & 1.0 \\
        Feet double stance & / & -1.0 \\
        Under speed & / & -0.2 \\
        Upper body pose & / & -0.05 \\
        Vertical linear velocity & -1.0 & -1.0 \\
        Roll/pitch angular velocity & -0.25 & -0.2 \\
        Base height & -500.0 & -120.0 \\
        Orientation & -5.0 & -2.5 \\
        Action rate & -0.01 & -0.005 \\
        Pose (weighted) & -0.1 & -0.05 \\
        \bottomrule
    \end{tabular}
\end{table}

Shaping parameters used by the table above: velocity-tracking $\sigma=0.25$, gait frequency $1.5$\,Hz, feet-phase swing height $0.09$\,m, feet-phase tracking $\sigma=0.008$, base-height target $0.754$\,m (MuJoCoUni) / $0.765$\,m (MotrixSim). The 29-entry pose-weight vector is identical on both backends. Under MotrixSim, the gait reward is gated by a minimum forward speed of $0.05$\,m/s.

\paragraph{G1 Walk Rough.}
\texttt{G1WalkRough} is the rough-terrain variant trained with SAC on both backends. The environment shares the same 29-DOF humanoid structure as G1 Walk Flat with terrain-aware reset behaviour.

\noindent\textbf{Observation space.}
Same structure as G1 Walk Flat: actor 98-dimensional, critic 101-dimensional. Refer to the G1 Walk Flat paragraph for the layout.

\noindent\textbf{Action space.}
29-dimensional joint-position offset with action scale $s=1.0$ (raised from the task default $0.25$). PD gains $K_p=50.0$, $K_d=1.0$.

\noindent\textbf{Commands and termination.}
The gait phase is initialized at the configured offset and the reset base-velocity is limited to $0.5$\,m/s. A base-velocity curriculum is enabled with initial scale $0.5$, maximum scale $1.0$, level-down threshold $150$, level-up threshold $750$, and degree $0.001$. Under MotrixSim, Kp/Kd randomization is disabled and the simulation step is set to $0.01$\,s. Termination uses a maximum tilt of $65^\circ$ and a minimum base height of $0.3$\,m.

\noindent\textbf{Domain randomization.}
Under MuJoCoUni, observation noise uses level $1.0$ with joint-angle scale $0.01$ and joint-velocity scale $0.1$ (other channels zero). Under MotrixSim, the default noise level is used. MuJoCoUni enables policy symmetry at the algorithm level; MotrixSim does not. Mass, COM, and push randomization are not enabled on either backend.

\noindent\textbf{Reward design.}
Table~\ref{tab:app_g1walkrough_reward} lists the active reward scales. MotrixSim uses a tighter feet-phase tracking sigma than MuJoCoUni.

\begin{table}[!htbp]
    \centering
    \caption{Reward terms for \texttt{g1\_walk\_rough}.}
    \label{tab:app_g1walkrough_reward}
    \begin{tabular}{@{}lcc@{}}
        \toprule
        Term & MuJoCoUni & MotrixSim \\
        \midrule
        Linear velocity tracking & 2.0 & 2.2 \\
        Yaw angular velocity tracking & 1.5 & 1.8 \\
        Penalty ang vel xy & -1.0 & -1.2 \\
        Penalty orientation & -10.0 & -12.0 \\
        Penalty action rate & -4.0 & -2.5 \\
        Pose (weighted) & -0.5 & -0.6 \\
        Penalty feet orientation & -20.0 & -5.0 \\
        Feet phase & 5.0 & 6.0 \\
        Alive & 10.0 & 12.0 \\
        \bottomrule
    \end{tabular}
\end{table}

Shaping parameters used by the table above: velocity-tracking $\sigma=0.25$, gait frequency $1.5$\,Hz, feet-phase swing height $0.09$\,m, feet-phase tracking $\sigma=0.04$ (MuJoCoUni) / $0.008$ (MotrixSim), close-feet threshold $0.15$\,m, base-height target $0.754$\,m. Termination thresholds (maximum tilt $65^\circ$, minimum base height $0.3$\,m) are repeated here from the Commands and termination paragraph for reference.

\subsubsection{Motion Tracking}
\label{app:task_motion_tracking}

The motion-tracking family imitates a reference motion clip on the 29-DOF G1 humanoid. All five tasks (\texttt{g1\_motion\_tracking}, \texttt{g1\_climb\_tracking}, \texttt{g1\_flip\_tracking}, \texttt{g1\_wall\_flip\_tracking}, \texttt{g1\_box\_tracking}) share the same observation/action layout and reward-term library; they differ in reference motion clip, scene, sampling mode, and termination thresholds. The shared structure is described once under G1 Motion Tracking; per-variant deltas follow.

\paragraph{G1 Motion Tracking.}
\texttt{G1MotionTracking} runs on the flat G1 scene with a dance reference clip. The configuration is identical across the two backends. Simulation step from the G1 base config, control step $\Delta t_{\mathrm{ctrl}}=0.02$\,s, maximum episode 10\,s.

\noindent\textbf{Observation space.}
The actor observation is 176-dimensional:
\begin{equation}
    o^{actor}_t = [m^{joint}_t,\,p^{ref}_{b,t},\,R^{ref}_{b,t},\,v^{base}_t,\,\omega_t,\,q_t-q_{\mathrm{default}},\,\dot q_t,\,a_{t-1}],
\end{equation}
where $m^{joint}_t\in\mathbb{R}^{58}$ is the reference joint position and velocity (29+29), $p^{ref}_{b,t}\in\mathbb{R}^3$ is the reference anchor position in body frame, $R^{ref}_{b,t}\in\mathbb{R}^6$ is the reference anchor orientation (6D rotation representation), and the remaining channels mirror the locomotion observation layout for 29 joints. The critic observation appends per-body privileged transforms for all 14 tracked bodies (3D position + 6D orientation each, $14\times9=126$ extra dims), giving a 302-dimensional critic.

The 14 tracked bodies are: \texttt{pelvis}, left/right \{\texttt{hip\_roll\_link}, \texttt{knee\_link}, \texttt{ankle\_roll\_link}\}, \texttt{torso\_link} (anchor body), left/right \{\texttt{shoulder\_roll\_link}, \texttt{elbow\_link}, \texttt{wrist\_yaw\_link}\}.

\noindent\textbf{Action space.}
29-dimensional joint-position offset with a per-joint 29-element action scale (not a single scalar). PD gains from the G1 base config ($K_p=50.0$, $K_d=1.0$).

\noindent\textbf{Commands and termination.}
There is no joystick command channel; the reference motion plays the role of command. Termination occurs when any of the following holds: anchor-position $z$-error exceeds $0.25$\,m, end-effector $z$-error exceeds $0.25$\,m, or a non-EE body falls below $0.05$\,m when undesired-contact termination is enabled. Anchor-orientation termination is disabled.

\noindent\textbf{Reference-clip sampling.}
The per-environment start frame is chosen at reset by one of four modes: always frame zero, random clip start, uniform over all frames, or failure-weighted adaptive bin sampling. G1 Motion Tracking uses the adaptive mode.

\noindent\textbf{Domain randomization.}
Under MuJoCoUni, observation noise uses the environment defaults. Under MotrixSim, noise level $1.0$ is enabled with joint-angle scale $0.01$, joint-velocity scale $1.5$, and gyro scale $0.2$. Base-mass, COM, gravity, push, and Kp/Kd randomization are not enabled.

\noindent\textbf{Reward design.}
Each motion-tracking term has the form $\exp(-e^2/\sigma^2)$ where $e$ is the reference-tracking error in the corresponding channel; non-tracking penalties use squared / L2 forms identical to the locomotion library. Table~\ref{tab:app_g1mt_reward} lists the active scales.

\begin{table}[!htbp]
    \centering
    \caption{Reward terms for \texttt{g1\_motion\_tracking}.}
    \label{tab:app_g1mt_reward}
    \begin{tabular}{@{}lcc@{}}
        \toprule
        Term & MuJoCoUni & MotrixSim \\
        \midrule
        motion\_global\_root\_pos & 0.5 & 1.0 \\
        motion\_global\_root\_ori & 0.5 & 0.5 \\
        motion\_body\_pos & 1.0 & 1.0 \\
        motion\_body\_ori & 1.0 & 1.0 \\
        motion\_body\_lin\_vel & 1.0 & 1.0 \\
        motion\_body\_ang\_vel & 1.0 & 1.0 \\
        action\_rate\_l2 & -0.1 & -0.05 \\
        joint\_limit & -10.0 & -10.0 \\
        undesired\_contacts & / & -0.1 \\
        \bottomrule
    \end{tabular}
\end{table}

Shaping parameters (per-channel tracking $\sigma$ used inside the $\exp(-e^2/\sigma^2)$ form) are identical on the two backends: $\sigma_{\mathrm{root\_pos}}=0.3$, $\sigma_{\mathrm{root\_ori}}=0.4$, $\sigma_{\mathrm{body\_pos}}=0.3$, $\sigma_{\mathrm{body\_ori}}=0.4$, $\sigma_{\mathrm{body\_lin\_vel}}=1.0$, $\sigma_{\mathrm{body\_ang\_vel}}=3.14$, $\sigma_{\mathrm{joint\_pos}}=0.2$, $\sigma_{\mathrm{joint\_vel}}=1.0$. The joint-position and joint-velocity tracking terms are not used in this configuration.

\paragraph{G1 Climb Tracking.}
The climb variant uses a scene with a 20-rung wall and a matched climbing reference clip. Maximum episode is $15$\,s, sampling is adaptive, simulation step is $0.005$\,s, undesired-contact termination is enabled, and anchor/end-effector $z$-error thresholds are both $0.3$\,m. The episode is not truncated when the clip ends.

The per-joint action scale is roughly $0.55$ for hip and ankle joints, $0.35$ for the knee, $0.44$ for waist and shoulder joints, and $0.07$ for wrist joints. Observation, action, and termination structure match G1 Motion Tracking.

\noindent\textbf{Reward design.}
Reward scales are identical across the two backends (Table~\ref{tab:app_g1ct_reward}). Compared to G1 Motion Tracking, the climb variant additionally weights end-effector vertical tracking, joint-position tracking, and joint-velocity tracking to encourage limb coordination with the reference clip.

\begin{table}[!htbp]
    \centering
    \caption{Reward terms for \texttt{g1\_climb\_tracking} (mj/mx identical).}
    \label{tab:app_g1ct_reward}
    \begin{tabular}{@{}lc@{}}
        \toprule
        Term & Weight \\
        \midrule
        motion\_global\_root\_pos & 0.5 \\
        motion\_global\_root\_ori & 0.5 \\
        motion\_body\_pos & 2.0 \\
        motion\_body\_ori & 1.5 \\
        motion\_body\_lin\_vel & 1.0 \\
        motion\_body\_ang\_vel & 1.0 \\
        motion\_ee\_body\_pos\_z & 2.0 \\
        motion\_joint\_pos & 0.5 \\
        motion\_joint\_vel & 0.25 \\
        action\_rate\_l2 & -0.005 \\
        joint\_limit & -10.0 \\
        undesired\_contacts & -0.1 \\
        \bottomrule
    \end{tabular}
\end{table}

The sigma values match the G1 Motion Tracking defaults (Table~\ref{tab:app_g1mt_reward}).

\paragraph{G1 Flip Tracking.}
The flip variant uses the flat G1 scene with a 360-degree flip reference clip. Sampling always starts from frame zero, the episode is not truncated when the clip ends, and the simulation step is $0.005$\,s.

Under MuJoCoUni, the anchor and end-effector $z$-error thresholds are both $0.5$\,m, undesired-contact termination is enabled, and the per-joint action scale matches G1 Climb Tracking. Under MotrixSim, the corresponding thresholds and action scale use the baseline environment settings.

\begin{table}[!htbp]
    \centering
    \caption{Reward terms for \texttt{g1\_flip\_tracking}.}
    \label{tab:app_g1ft_reward}
    \begin{tabular}{@{}lcc@{}}
        \toprule
        Term & MuJoCoUni & MotrixSim \\
        \midrule
        motion\_global\_root\_pos & 0.5 & 1.0 \\
        motion\_global\_root\_ori & 0.5 & 0.5 \\
        motion\_body\_pos & 2.0 & 1.0 \\
        motion\_body\_ori & 1.5 & 1.0 \\
        motion\_body\_lin\_vel & 1.0 & 1.0 \\
        motion\_body\_ang\_vel & 1.0 & 1.0 \\
        motion\_ee\_body\_pos\_z & 2.0 & / \\
        action\_rate\_l2 & -0.005 & -0.05 \\
        joint\_limit & -10.0 & -10.0 \\
        undesired\_contacts & -0.1 & / \\
        \bottomrule
    \end{tabular}
\end{table}

\paragraph{G1 Wall Flip Tracking.}
The wall-flip variant uses a flat scene with a wall and a wall-flip reference clip. Sampling always starts from frame zero, the episode is not truncated when the clip ends, the simulation step is $0.005$\,s, anchor and end-effector $z$-error thresholds are both $0.5$\,m, undesired-contact termination is enabled, and the per-joint action scale matches G1 Climb Tracking. Under MotrixSim, the solver runs three substep iterations per control step.

Reward scales are identical across the two backends and match the climb-tracking weights (Table~\ref{tab:app_g1ct_reward}); only the reference clip and the wall-scene termination geometry change.

\paragraph{G1 Box Tracking.}
The box variant uses a flat scene with a large box and a box-manipulation reference clip. It extends G1 Motion Tracking with explicit object-state tracking: the critic observation appends 12 extra dimensions (object position, object 6D orientation, object linear velocity, all in body frame) for a 314-dimensional critic. The actor observation remains 176-dimensional. Under MuJoCoUni, the simulation step is $0.005$\,s; under MotrixSim, the base step is used.

Under MotrixSim, empirical normalization is enabled, an asymmetric critic observation group is declared, and observation noise uses level $1.0$ with joint-angle scale $0.01$, joint-velocity scale $1.5$, and gyro scale $0.2$.

\begin{table}[!htbp]
    \centering
    \caption{Reward terms for \texttt{g1\_box\_tracking}.}
    \label{tab:app_g1bt_reward}
    \small
    \begin{tabular}{@{}lcc@{}}
        \toprule
        Term & MuJoCoUni & MotrixSim \\
        \midrule
        motion\_global\_root\_pos & 0.5 & 1.0 \\
        motion\_global\_root\_ori & 0.5 & 0.5 \\
        motion\_body\_pos & 1.0 & 1.0 \\
        motion\_body\_ori & 1.0 & 1.5 \\
        motion\_body\_lin\_vel & 1.0 & 1.0 \\
        motion\_body\_ang\_vel & 1.0 & 1.5 \\
        action\_rate\_l2 & -0.1 & -0.1 \\
        joint\_limit & -10.0 & -10.0 \\
        undesired\_contacts & -0.1 & -0.1 \\
        object\_global\_ref\_position\_error\_exp & 2.0 & 4.0 \\
        object\_global\_ref\_orientation\_error\_exp & 2.0 & 3.0 \\
        \bottomrule
    \end{tabular}
\end{table}

Body-tracking sigmas inherit the G1 Motion Tracking defaults; the object-tracking sigmas used inside $\exp(-e^2/\sigma^2)$ differ between backends: $\sigma_{\mathrm{object\_pos}}=0.2$ (MuJoCoUni) / $0.12$ (MotrixSim), $\sigma_{\mathrm{object\_ori}}=0.3$ (MuJoCoUni) / $0.2$ (MotrixSim).

\subsubsection{Manipulation-Locomotion}
\label{app:task_manipulation_locomotion}

This subsection covers tasks where locomotion is coupled with an upper-body manipulation or posture objective. Two tasks are included: Go2 Hand Stand (rear-leg balance) and Go2 Arm Manip Loco (locomotion with a 6-DOF arm tracking an end-effector goal).

\paragraph{Go2 Hand Stand.}
\texttt{Go2HandStand} rewards the robot for inverting onto its front legs while maintaining a target torso height. Under MuJoCoUni the simulation step is $0.005$\,s; under MotrixSim it is $0.01$\,s. Control step $\Delta t_{\mathrm{ctrl}}=0.02$\,s, maximum episode 20\,s.

\noindent\textbf{Observation space.}
The actor observation is 42-dimensional:
\begin{equation}
    o_t = [\omega_t,\,-g_t,\,q_t-q_{\mathrm{default}},\,\dot q_t,\,a_{t-1}],
\end{equation}
where joint offset, joint velocity, and last action are 12-dimensional each. No velocity command channel; the task is a fixed posture-tracking objective. The critic observation is 46-dimensional (adds base linear velocity 3 and torso height 1).

\noindent\textbf{Action space.}
12-dimensional joint-position offset with default \texttt{action\_scale}. PD gains $K_p=35.0$, $K_d=0.5$.

\noindent\textbf{Commands and termination.}
The target pose is inverted handstand: target torso height $z_{des}=0.55$\,m, desired gravity $g_{des}=(-1,0,0)$ (body $x$-axis aligned with world gravity). Termination occurs when the up-vector $z$-component satisfies $g^z_t \le -0.25$ (robot fully inverted past the target) or when undesired contacts on front legs/hips/thighs occur. A rear-leg gait at 2\,Hz (RL phase 0, RR phase 0.5) provides a phase signal for the gait-aware reward terms.

\noindent\textbf{Domain randomization.}
Under MotrixSim, Kp/Kd randomization is disabled. No additional domain randomization is enabled on top of the environment defaults.

\noindent\textbf{Reward design.}
Table~\ref{tab:app_go2hs_reward} lists the active reward scales. The two backends differ only in the front-leg contact weight.

\begin{table}[!htbp]
    \centering
    \caption{Reward terms for \texttt{go2\_handstand}.}
    \label{tab:app_go2hs_reward}
    \begin{tabular}{@{}lcc@{}}
        \toprule
        Term & MuJoCoUni & MotrixSim \\
        \midrule
        Contact (front-leg) & -1.0 & -0.5 \\
        Height & 1.0 & 1.0 \\
        Orientation (alignment to target gravity) & 1.0 & 1.0 \\
        Pose (deviation from default) & -0.3 & -0.3 \\
        Penalty contact (penalty bodies) & -0.2 & -0.2 \\
        Action rate & -0.01 & -0.01 \\
        Target pose (\texttt{tar}) & 0.3 & 0.3 \\
        Feet air time (rear legs) & 1.0 & 1.0 \\
        World $z$-velocity penalty & -1.0 & -1.0 \\
        \bottomrule
    \end{tabular}
\end{table}

Shaping parameters: velocity-tracking $\sigma=0.25$ and base-height target $0.3$\,m on both backends. The \texttt{height} term uses $\exp(-|z_{des}-h|/0.1)$, the \texttt{orientation} term uses $[0.5\cos\angle(g,g_{des})+0.5]^2$, and the \texttt{tar} reward is gated by $h \ge 0.8\,z_{des}$.

\paragraph{Go2 Arm Manip Loco.}
\texttt{Go2ArmManipLoco} is available only on the MuJoCoUni backend. Simulation step $\Delta t_{\mathrm{sim}}=0.01$\,s, control step $\Delta t_{\mathrm{ctrl}}=0.02$\,s, maximum episode 20\,s.

\noindent\textbf{Observation space.}
The per-step observation is 79-dimensional:
\begin{equation}
    o_t = [v^{base}_t,\,\omega_t,\,-g_t,\,c_t,\,\phi_t,\,q_t-q_{\mathrm{default}},\,\dot q_t,\,p^{ee}_t,\,p^{goal}_t,\,e^{ee}_t,\,a_{t-1}],
\end{equation}
where $\phi_t\in\mathbb{R}^4$ is the four-foot gait phase, joint offset/velocity are 18-dimensional each (12 leg + 6 arm), $p^{ee}_t,\,p^{goal}_t,\,e^{ee}_t\in\mathbb{R}^3$ are end-effector position, goal, and error in body frame, and the action history is 18-dimensional. The actor observation drops base linear velocity (to avoid bypassing the on-board estimator) and uses a per-step history of $H_a$ frames; the critic observation keeps linear velocity and uses $H_c$ frames. Default history length is $H_a=H_c=1$.

\noindent\textbf{Action space.}
18-dimensional: 12 leg-joint offsets with action scale $0.25$ (hip-joint scale $0.125$) and 6 arm-joint offsets with arm action scale zero. Leg PD gains $K_p=35.0$, $K_d=0.5$. With the arm scale set to zero, the policy controls only the legs; the arm follows the IK-derived target from the end-effector goal.

\noindent\textbf{End-effector goal sampling.}
The end-effector goal is sampled in spherical coordinates around the body: radius $\in[0.3,0.6]$\,m, azimuth $\in[-1.26,1.05]$\,rad, polar angle $\in[-2.36,2.36]$\,rad. Trajectory time $\in[1.0,3.0]$\,s, hold time $\in[0.5,2.0]$\,s. Collision bounds: upper $[0.3,0.15,-0.115]$, lower $[-0.2,-0.15,-0.515]$, underground limit $z=-0.57$. The IK uses damping $0.05$, gain $1.0$, $\Delta q$-clip $0.2$, with target-orientation tracking.

\noindent\textbf{Commands and termination.}
Velocity-command range $[(-0.6,-0.4,-0.8),(1.0,0.4,0.8)]$, zero-command probability $0.15$ (for stable standing), command resampling every $4.0$\,s. The velocity curriculum is disabled. Termination: $g^z_t \le 0.5$.

\noindent\textbf{Domain randomization.}
The following terms are enabled: body-mass multiplier $[0.9, 1.1]$, random COM offset $x\in[-0.03,0.03]$, ground-friction multiplier $[0.8,1.2]$, DOF-armature multiplier $[0.8,1.2]$, base pushes every 500 steps with maximum force $[1.2,1.2,0.6]$, and Kp/Kd multipliers $[0.9,1.1]$. Base-mass and gravity randomization are not enabled.

\noindent\textbf{Reward design.}
Table~\ref{tab:app_go2arml_reward} lists the active reward scales.

\begin{table}[!htbp]
    \centering
    \caption{Reward terms for \texttt{go2\_arm\_manip\_loco}.}
    \label{tab:app_go2arml_reward}
    \begin{tabular}{@{}lc@{}}
        \toprule
        Term & MuJoCoUni \\
        \midrule
        Linear velocity tracking & 2.0 \\
        Yaw angular velocity tracking & 0.5 \\
        Vertical linear velocity & -5.0 \\
        Roll/pitch angular velocity & -0.1 \\
        Roll & -5.0 \\
        Base height & -100.0 \\
        Leg pose & -0.1 \\
        Action rate & -0.005 \\
        Stand still & -0.5 \\
        Contact phase agreement & 0.24 \\
        Swing-foot height & 4.0 \\
        Foot drag & -0.1 \\
        Object distance (to EE goal) & 2.0 \\
        Object distance L2 & -0.5 \\
        Arm collision & -1.0 \\
        \bottomrule
    \end{tabular}
\end{table}

Shaping parameters: velocity-tracking $\sigma=0.25$, base-height target $0.3$\,m, object-distance kernel $\sigma=0.1$.

\subsubsection{Dexterous-Hand and In-Hand Manipulation}
\label{app:task_dexterous_hand}

This subsection covers in-hand manipulation tasks where a multi-finger hand rotates a free object about a specified axis. Two tasks are included: Allegro Inhand Rotation (16-DOF hand, ball) and Sharpa Inhand Rotation (22-DOF hand with tactile sensing).

\paragraph{Allegro Inhand Rotation.}
\texttt{AllegroInhandRotation} rotates a free ball about a fixed world-axis using the 16-DOF Allegro hand. The configuration is identical across the two backends. Simulation step $\Delta t_{\mathrm{sim}}=0.005$\,s, control step $\Delta t_{\mathrm{ctrl}}=0.05$\,s (10 simulator steps per control step), maximum episode 20\,s.

\noindent\textbf{Observation space.}
The observation is 105-dimensional, organized as a lag-history of 3 steps of a 35-dimensional per-step frame:
\begin{equation}
    f_t = [\widetilde q^{hand}_t,\,q^{target}_t,\,p^{ball}_t],
\end{equation}
where $\widetilde q^{hand}_t\in\mathbb{R}^{16}$ is the normalized hand joint position (mapped from joint limits to $[-2,2]$), $q^{target}_t\in\mathbb{R}^{16}$ is the current incremental joint target, and $p^{ball}_t\in\mathbb{R}^3$ is the ball position. Actor and critic share a single observation group; the critic has no privileged channel.

\noindent\textbf{Action space.}
16-dimensional in $[-1,1]$. The environment maps actions to actuator targets incrementally: $q^{target}_t = q^{target}_{t-1} + s\,\mathrm{clip}(a_t)$ with $s = 1/24 \approx 0.0417$, then clipped to the actuator-range limits. PD gains $K_p=1.0$, $K_d=0.1$. Torque is clipped to $[-0.5, 0.5]$.

\noindent\textbf{Commands and termination.}
The rotation axis is the world $z$-axis, $\hat n=(0,0,1)$. The episode terminates when the ball height drops below $0.125$\,m.

\noindent\textbf{Domain randomization.}
All online domain randomization is disabled (base-mass, COM, gravity, push, joint noise, ball-velocity noise, ball-$z$ offset). Reset-time grasp variation is the only source of initialization diversity.

\noindent\textbf{Reward design.}
Reward scales are identical across the two backends (Table~\ref{tab:app_allegro_reward}).

\begin{table}[!htbp]
    \centering
    \caption{Reward terms for \texttt{allegro\_inhand} (mj/mx identical).}
    \label{tab:app_allegro_reward}
    \begin{tabular}{@{}lc@{}}
        \toprule
        Term & Weight \\
        \midrule
        rotate (\texttt{clip}$(\boldsymbol\omega^{ball}\cdot\hat n,-0.5,0.5)$) & 1.25 \\
        obj\_linvel ($\sum_i |v^{ball}_i|$) & -0.3 \\
        pose\_diff ($\sum_j(q_j-q_j^{init})^2$) & -0.3 \\
        torque ($\sum_j \tau_j^2$) & -0.1 \\
        work ($(\sum_j \tau_j \dot q_j)^2$) & -2.0 \\
        \bottomrule
    \end{tabular}
\end{table}

Shaping parameters: angular-velocity clip range $[-0.5, 0.5]$\,rad/s inside the rotate term, and ball-height reset threshold $0.125$\,m used by the termination check. The reward is $\Delta t_{\mathrm{ctrl}}\sum_i w_i r_i$.

\paragraph{Sharpa Inhand Rotation.}
\texttt{SharpaInhandRotation} rotates a cylinder using the 22-DOF Sharpa hand with tactile sensing. The numbers reported here correspond to the MuJoCoUni HORA teacher configuration, which is shared by the APPO, SAC, and PPO HORA comparisons. Simulation step $1/240$\,s, control step $\Delta t_{\mathrm{ctrl}}=12/240=0.05$\,s, maximum episode 20\,s.

\noindent\textbf{Observation space.}
The per-step policy frame is 49-dimensional:
\begin{equation}
    f_t = [\widetilde q^{hand}_t,\,q^{target}_t,\,F^{tactile}_t],
\end{equation}
with $\widetilde q^{hand}_t\in\mathbb{R}^{22}$, $q^{target}_t\in\mathbb{R}^{22}$, and tactile forces $F^{tactile}_t\in\mathbb{R}^5$ (one per fingertip). The frame is stacked over a 3-step lag history, giving a 147-dimensional policy observation. The privileged tail is 9-dimensional: object position delta (3), friction scale (1), mass (1), COM offset (3), and object scale (1). In flattened mode the single observation group is $147+9=156$-dimensional. In separated mode the actor receives the 147-dimensional policy observation, while the critic receives the 156-dimensional concatenation.

\noindent\textbf{Action space.}
22-dimensional in $[-1,1]$. Incremental position control: $q^{target}_t = q^{target}_{t-1} + s\,\mathrm{clip}(a_t)$, $s=1/24$, with joint limits scaled by $0.9$. PD gains are set per actuator and randomized at reset within $[0.5, 2.0]$ around their nominal values.

\noindent\textbf{Commands and termination.}
Rotation axis $\hat n = (0,0,1)$. Termination uses object world-$z$ height bounds $[p^{obj}_z - 0.5\Delta h, p^{obj}_z + 0.5\Delta h]$ with $\Delta h = 0.04$\,m centered on the reset object position; the fallback bounds are $[0.59906, 0.63906]$\,m. The rotation rollout does not use angular-violation termination; angular deviation is used only during offline grasp-state filtering.

\noindent\textbf{Domain randomization.}
A rich randomization stack is enabled on both backends (Table~\ref{tab:app_sharpa_dr}). The reported Sharpa teacher runs use eight cylinder scales $\{0.8\ldots1.5\}$, excluding 1.6 to align with the external baseline setup. The active gravity setting is fixed-magnitude direction randomization; full-vector gravity randomization is disabled.

\begin{table}[!htbp]
    \centering
    \caption{Domain randomization for \texttt{sharpa\_inhand}.}
    \label{tab:app_sharpa_dr}
    \begin{tabular}{@{}lcc@{}}
        \toprule
        Item & MuJoCoUni & MotrixSim \\
        \midrule
        Scale list (cylinder sizes) & $\{0.8\ldots1.5\}$ & $\{0.8\ldots1.5\}$ \\
        \texttt{randomize\_gravity\_direction} & true & true \\
        Gravity magnitude & 9.81 & 9.81 \\
        \texttt{randomize\_gravity} (full vector) & false & false \\
        \texttt{randomize\_pd\_gains} & true & true \\
        $K_p$ scale range & $[0.5, 2.0]$ & $[0.5, 2.0]$ \\
        $K_d$ scale range & $[0.5, 2.0]$ & $[0.5, 2.0]$ \\
        \texttt{randomize\_friction} & true & true \\
        Friction scale range & $[0.75, 1.25]$ & $[0.75, 1.25]$ \\
        Elastomer/metal/object base friction & $2.0, 1.0, 2.0$ & $2.0, 1.0, 2.0$ \\
        \texttt{randomize\_com} & true & true \\
        COM offset range & $[-0.01, 0.01]$ & $[-0.01, 0.01]$ \\
        \texttt{randomize\_mass} & true & true \\
        Mass range & $[0.01, 0.25]$ & $[0.01, 0.25]$ \\
        Force perturbation scale & 2.0 & 2.0 \\
        Force probability per step & 0.25 & 0.25 \\
        Force decay / interval & $0.9 / 0.08$ & $0.9 / 0.08$ \\
        Joint observation noise scale & 0.02 & 0.02 \\
        Contact latency & 0.005 & 0.005 \\
        Contact sensor noise & 0.01 & 0.01 \\
        \bottomrule
    \end{tabular}
\end{table}

\noindent\textbf{Reward design.}
Reward scales are identical across the two backends (Table~\ref{tab:app_sharpa_reward}).

\begin{table}[!htbp]
    \centering
    \caption{Reward terms for \texttt{sharpa\_inhand} (mj/mx identical).}
    \label{tab:app_sharpa_reward}
    \begin{tabular}{@{}lc@{}}
        \toprule
        Term & Weight \\
        \midrule
        rotate (\texttt{clip}$(\boldsymbol\omega^{obj}\cdot\hat n,-0.5,0.5)$) & 2.5 \\
        obj\_linvel ($\sum_i |v^{obj}_i|$) & -0.3 \\
        pose\_diff ($\sum_j(q_j-q_j^{def})^2$) & -0.4 \\
        torque (squared virtual torque) & -0.1 \\
        work ($(\sum_j \tau_j \dot q_j)^2$) & -0.5 \\
        object\_pos ($1/(\|p^{obj}-p^{anchor}\|+10^{-3})$) & 0.003 \\
        \bottomrule
    \end{tabular}
\end{table}

The rotate term clips its angular-velocity argument to $[-0.5, 0.5]$\,rad/s before applying the weight.

\subsection{Algorithm Hyperparameters}
\label{app:training_curves_algorithms}

This subsection lists the per-algorithm global defaults and the per-task overrides applied on top of them. Reward weights and environment-side hyperparameters are documented in Section~\ref{app:training_curves_tasks}; only algorithm-side training hyperparameters appear here.

\subsubsection{PPO}
\label{app:algorithm_ppo}

We report PPO hyperparameters as global defaults followed by per-task overrides.

\paragraph{PPO global defaults.}
Table~\ref{tab:app_ppo_default} lists the global defaults inherited by every PPO task before any per-task override.

\begin{table}[!htbp]
    \centering
    \small
    \caption{PPO global default hyperparameters.}
    \label{tab:app_ppo_default}
    \begin{tabular}{@{}ll@{}}
        \toprule
        Field & Default Value \\
        \midrule
        \multicolumn{2}{l}{\emph{Runner / Environment}} \\
        \texttt{algo} & ppo \\
        \texttt{algo\_log\_name} & rsl\_rl\_ppo \\
        \texttt{seed} & $1$ \\
        \texttt{num\_envs} & $4096$ \\
        \texttt{num\_steps\_per\_env} & $24$ \\
        \texttt{max\_iterations} & $101$ \\
        \texttt{save\_interval} & $100$ \\
        \texttt{empirical\_normalization} & false \\
        \texttt{runner\_class\_name} & \texttt{OnPolicyRunner} \\
        \texttt{obs\_groups.default} & \texttt{[policy]} \\
        \midrule
        \multicolumn{2}{l}{\emph{Policy network}} \\
        \texttt{policy.class\_name} & \texttt{ActorCritic} \\
        \texttt{policy.actor\_hidden\_dims} & $[512, 256, 128]$ \\
        \texttt{policy.critic\_hidden\_dims} & $[512, 256, 128]$ \\
        \texttt{policy.activation} & elu \\
        \texttt{policy.init\_noise\_std} & $1.0$ \\
        \midrule
        \multicolumn{2}{l}{\emph{Algorithm}} \\
        \texttt{algorithm.class\_name} & \texttt{FinalObservationAwarePPO} \\
        \texttt{algorithm.value\_loss\_coef} & $1.0$ \\
        \texttt{algorithm.use\_clipped\_value\_loss} & true \\
        \texttt{algorithm.clip\_param} & $0.2$ \\
        \texttt{algorithm.entropy\_coef} & $0.01$ \\
        \texttt{algorithm.num\_learning\_epochs} & $5$ \\
        \texttt{algorithm.num\_mini\_batches} & $4$ \\
        \texttt{algorithm.learning\_rate} & $1.0\times10^{-3}$ \\
        \texttt{algorithm.schedule} & adaptive \\
        \texttt{algorithm.gamma} & $0.99$ \\
        \texttt{algorithm.lam} & $0.95$ \\
        \texttt{algorithm.desired\_kl} & $0.01$ \\
        \texttt{algorithm.max\_grad\_norm} & $1.0$ \\
        \texttt{algorithm.adaptive\_kl\_beta} & $0.9$ \\
        \texttt{algorithm.adaptive\_lr\_growth} & $1.1$ \\
        \texttt{algorithm.adaptive\_lr\_decay} & $1.2$ \\
        \texttt{algorithm.adaptive\_lr\_update\_interval} & $5$ \\
        \bottomrule
    \end{tabular}
\end{table}

\paragraph{PPO overrides across tasks.}
Tables~\ref{tab:app_ppo_loco_overrides}--\ref{tab:app_ppo_hand_overrides} summarize the PPO-side overrides for each task. Fields not listed are inherited from Table~\ref{tab:app_ppo_default}. When the two backends differ, the value is written as ``mj / mx''; identical values are written once.

\begin{table}[!htbp]
    \centering
    \caption{PPO overrides for locomotion tasks (Go1, Go2, Go2W families). Cells with a slash report ``mj~/~mx'' values; single values are shared between the two backends.}
    \label{tab:app_ppo_loco_overrides}
    \resizebox{\textwidth}{!}{%
    \begin{tabular}{@{}lcccccc@{}}
        \toprule
        Field & Go1 Flat & Go1 Rough & Go2 Flat & Go2 Rough & Go2W Flat & Go2W Rough \\
        \midrule
        \texttt{num\_envs}              & $4096$               & $4096$       & $1024$       & $4096$       & $1024$       & $2048$ \\
        \texttt{num\_steps\_per\_env}   & $24$                 & $24$         & $24$         & $24$         & $24$         & $48 / 24$ \\
        \texttt{max\_iterations}        & $151$                & $600$        & $151$        & $1000$       & $151$        & $5000 / 2000$ \\
        \texttt{empirical\_normalization} & false / true       & false        & true         & false        & true         & false \\
        \texttt{init\_noise\_std}       & inherited / $0.5$    & $1.0$        & $0.5$        & $1.0$        & $0.5$        & inherited \\
        \texttt{learning\_rate}         & $10^{-3} / 3{\times}10^{-4}$ & $10^{-3}$ & $3{\times}10^{-4}$ & $10^{-3}$ & $3{\times}10^{-4}$ & inherited \\
        \texttt{entropy\_coef}          & $0.01 / 10^{-3}$     & $0.01$       & $10^{-3}$    & $0.01$       & $10^{-3}$    & inherited \\
        \bottomrule
    \end{tabular}}
\end{table}

For Go1 Joystick Flat, empirical normalization, the lower action-noise std, and the lower learning rate / entropy coefficient are applied only under MotrixSim. Go2 Joystick Flat uses the same lowered values on both backends. Go1 / Go2 Joystick Rough share a single hyperparameter set between the two backends with action-noise std $1.0$ and entropy coefficient $0.01$. Go2W Joystick Flat and Rough use the same hyperparameters on both backends apart from rollout length and iteration count in the Rough case.

\begin{table}[!htbp]
    \centering
    \caption{PPO overrides for humanoid locomotion and tracking tasks. Cells with a slash report ``mj~/~mx'' values; single values are shared between the two backends.}
    \label{tab:app_ppo_g1_overrides}
    \resizebox{\textwidth}{!}{%
    \begin{tabular}{@{}lccccc@{}}
        \toprule
        Field & G1 Walk Flat & G1 Motion & G1 Climb & G1 Flip & G1 Wall Flip \\
        \midrule
        \texttt{num\_envs}              & $2048$                       & $1024$       & $1024$       & $1024$              & $1024$ \\
        \texttt{num\_steps\_per\_env}   & $24$                         & $24$         & $24$         & $24$                & $24$ \\
        \texttt{max\_iterations}        & $2200$                       & $15000$      & $20000$      & $20000 / 30000$     & $20000 / 12000$ \\
        \texttt{empirical\_normalization} & false / true               & false        & true         & true / false        & true \\
        \texttt{init\_noise\_std}       & inherited / $0.5$            & inherited    & inherited    & inherited           & inherited \\
        \texttt{learning\_rate}         & $10^{-3} / 3{\times}10^{-4}$ & $10^{-3}$    & $10^{-3}$    & $10^{-3}$           & $10^{-3}$ \\
        \texttt{entropy\_coef}          & $0.01 / 5{\times}10^{-3}$    & $0.005$      & $0.005$      & $0.005$             & $0.005$ \\
        \texttt{desired\_kl}            & inherited                    & inherited    & $0.01$       & $0.01 / $ inh.      & $0.01$ \\
        \texttt{save\_interval}         & $100$                        & $500$        & $500$        & $500$               & $500$ \\
        \texttt{obs\_groups}            & symmetric / asymmetric       & symmetric    & asymmetric   & asymmetric          & asymmetric \\
        \bottomrule
    \end{tabular}}
\end{table}

Asymmetric observation groups means the actor and critic see different channels, enabling privileged critic observations. G1 Walk Flat enables this only under MotrixSim. G1 Box Tracking uses \texttt{num\_envs}$=1024$, \texttt{max\_iterations}$=30000 / 40000$, empirical normalization false / true, entropy coefficient $0.005 / 0.002$, save interval $500$, and asymmetric observation groups under MotrixSim.

\begin{table}[!htbp]
    \centering
    \caption{PPO overrides for handstand, arm-loco, and dexterous tasks.}
    \label{tab:app_ppo_hand_overrides}
    \begingroup
    \small
    \setlength{\tabcolsep}{3pt}
    \resizebox{\textwidth}{!}{%
    \begin{tabular}{@{}lcccc@{}}
        \toprule
        Field & Go2 HandStand & Go2 Arm Loco & Allegro & Sharpa HORA PPO \\
        \midrule
        \texttt{num\_envs}              & $1024$       & $4096$               & $16384$      & $2048$ \\
        \texttt{num\_steps\_per\_env}   & $24$         & $24$                 & $8$          & $24$ \\
        \texttt{max\_iterations}        & $3000$       & $151$                & $201$        & $301$ \\
        \texttt{empirical\_normalization} & inherited & true                  & true         & true \\
        \texttt{init\_noise\_std}       & $0.5$        & $0.5$                & inherited    & inherited \\
        \texttt{learning\_rate}         & inherited    & $3{\times}10^{-4}$   & inherited    & $10^{-3}$ \\
        \texttt{entropy\_coef}          & $0.005$      & $10^{-3}$            & $0.01$       & $0.01$ \\
        \texttt{value\_loss\_coef}      & inherited    & inherited            & $4.0$        & $4.0$ \\
        \texttt{desired\_kl}            & inherited    & inherited            & $0.02$       & $0.02$ \\
        \texttt{save\_interval}         & inherited    & inherited            & inherited    & $50$ \\
        \texttt{obs\_groups}            & asymmetric   & symmetric            & symmetric    & actor/critic both [actor] \\
        \bottomrule
    \end{tabular}}
    \endgroup
\end{table}

Go2 Arm Manip Loco is available only under MuJoCoUni; the MotrixSim column does not apply. Allegro Inhand and generic Sharpa Inhand use identical hyperparameters on both backends. The Sharpa column reports the HORA PPO setting used for the main Sharpa PPO comparison.

\subsubsection{APPO}
\label{app:algorithm_appo}

APPO is the asynchronous on-policy variant used in UniLab; it shares PPO's clipped-surrogate objective but allows the learner to consume rollouts produced with a slightly stale policy. Only APPO training hyperparameters appear here; task-side values (rewards, observation/action spaces, domain randomization) are documented in the task specifications above.

\paragraph{APPO global defaults.}
Table~\ref{tab:app_appo_default} lists the global defaults inherited by every APPO task before any per-task override.

\begin{table}[!htbp]
    \centering
    \small
    \caption{APPO global default hyperparameters.}
    \label{tab:app_appo_default}
    \begin{tabular}{@{}ll@{}}
        \toprule
        Field & Default Value \\
        \midrule
        \multicolumn{2}{l}{\emph{Runner / Environment}} \\
        \texttt{algo} & appo \\
        \texttt{algo\_log\_name} & appo \\
        \texttt{seed} & $1$ \\
        \texttt{num\_envs} & $2048$ \\
        \texttt{steps\_per\_env} & $24$ \\
        \texttt{max\_iterations} & $150$ \\
        \texttt{save\_interval} & $50$ \\
        \texttt{obs\_groups.actor} & \texttt{\{policy: 0\}} \\
        \midrule
        \multicolumn{2}{l}{\emph{Actor / Critic networks}} \\
        \texttt{actor.class\_name} & \texttt{rsl\_rl.models.MLPModel} \\
        \texttt{actor.hidden\_dims} & $[512, 256, 128]$ \\
        \texttt{actor.activation} & elu \\
        \texttt{actor.obs\_normalization} & false \\
        \texttt{actor.distribution\_cfg.class\_name} & \texttt{GaussianDistribution} \\
        \texttt{actor.distribution\_cfg.init\_std} & $1.0$ \\
        \texttt{actor.distribution\_cfg.std\_type} & scalar \\
        \texttt{critic.class\_name} & \texttt{rsl\_rl.models.MLPModel} \\
        \texttt{critic.hidden\_dims} & $[512, 256, 128]$ \\
        \texttt{critic.activation} & elu \\
        \texttt{critic.obs\_normalization} & false \\
        \midrule
        \multicolumn{2}{l}{\emph{Algorithm}} \\
        \texttt{algorithm.num\_learning\_epochs} & $5$ \\
        \texttt{algorithm.num\_mini\_batches} & $4$ \\
        \texttt{algorithm.clip\_param} & $0.2$ \\
        \texttt{algorithm.gamma} & $0.99$ \\
        \texttt{algorithm.lam} & $0.95$ \\
        \texttt{algorithm.value\_loss\_coef} & $1.0$ \\
        \texttt{algorithm.entropy\_coef} & $0.01$ \\
        \texttt{algorithm.learning\_rate} & $1.0\times10^{-3}$ \\
        \texttt{algorithm.max\_grad\_norm} & $1.0$ \\
        \texttt{algorithm.use\_clipped\_value\_loss} & true \\
        \texttt{algorithm.schedule} & adaptive \\
        \texttt{algorithm.desired\_kl} & $0.01$ \\
        \texttt{algorithm.adaptive\_kl\_factor} & $1.2$ \\
        \texttt{algorithm.adaptive\_lr\_factor} & $1.1$ \\
        \texttt{algorithm.optimizer} & adam \\
        \texttt{algorithm.tau} (target update) & $1.0$ \\
        \texttt{algorithm.target\_update\_freq} & $1$ \\
        \texttt{algorithm.vtrace\_clip\_rho} & $1.0$ \\
        \texttt{algorithm.vtrace\_clip\_c} & $1.0$ \\
        \bottomrule
    \end{tabular}
\end{table}

\paragraph{APPO overrides across tasks.}
Tables~\ref{tab:app_appo_loco_overrides} and ~\ref{tab:app_appo_tracking_overrides} list the per-task overrides. Fields not listed are inherited from Table~\ref{tab:app_appo_default}. When the two backends differ, the value is written as ``mj / mx''; identical values appear once.

\begin{table}[!htbp]
    \centering
    \small
    \caption{APPO overrides for locomotion and dexterous tasks.}
    \label{tab:app_appo_loco_overrides}
    \begin{tabular}{@{}lcccc@{}}
        \toprule
        Field & Go1 Flat & Go2 Flat & Allegro MuJoCo & Sharpa HORA \\
        \midrule
        \texttt{num\_envs} & inherited & inherited & $1024$ & $2048$ \\
        \texttt{steps\_per\_env} & inherited & inherited & $8$ & $8$ \\
        \texttt{max\_iterations} & $150$ & $150$ & $3000$ & $1360$ \\
        \texttt{save\_interval} & inherited & inherited & $5000$ & $170$ \\
        \texttt{training.replay\_queue\_size} & inherited & inherited & $4$ & $8$ \\
        \texttt{actor.obs\_normalization} & inherited & inherited & true & true \\
        \texttt{critic.obs\_normalization} & inherited & inherited & true & true \\
        \texttt{algorithm.value\_loss\_coef} & inherited & inherited & $4.0$ & $4.0$ \\
        \texttt{algorithm.desired\_kl} & inherited & inherited & $0.025$ & $0.04$ \\
        \bottomrule
    \end{tabular}
\end{table}

Go1/Go2 Joystick Flat run under MuJoCoUni only. The Sharpa HORA setting uses \texttt{runtime\_impl=hora\_appo}, separated actor/critic observations, a 9-dimensional privileged embedding, and HORA actor/critic model classes. The generic non-HORA Sharpa APPO setting is not the teacher recipe reported for the Sharpa HORA curves.

\begin{table}[!htbp]
    \centering
    \small
    \caption{APPO overrides for motion-tracking tasks (mj/mx identical for all four).}
    \label{tab:app_appo_tracking_overrides}
    \begin{tabular}{@{}lcccc@{}}
        \toprule
        Field & G1 Motion & G1 Climb & G1 Flip & G1 Wall Flip \\
        \midrule
        \texttt{num\_envs} & $1024$ & $1024$ & $1024$ & $1024$ \\
        \texttt{steps\_per\_env} & inherited & inherited & inherited & inherited \\
        \texttt{max\_iterations} & $5000$ & $20000$ & $5000$ & $5000$ \\
        \texttt{save\_interval} & $500$ & $500$ & $500$ & $500$ \\
        \bottomrule
    \end{tabular}
\end{table}

All four motion-tracking tasks use the same APPO configuration on both backends. G1 Box Tracking is not available under APPO.

\subsubsection{SAC}
\label{app:algorithm_sac}

SAC is the entropy-regularized off-policy actor-critic used in UniLab for replay-buffer experiments. The shared family contains two implementation variants: the standard SAC trainer (\texttt{algo: sac}) and the FlashSAC accelerated variant (\texttt{algo: flashsac}). Both consume rollouts via a replay buffer and respect the off-policy producer/consumer protocol described in the main text.

\paragraph{SAC global defaults.}
Table~\ref{tab:app_sac_default} lists the global defaults inherited by every SAC task before any per-task override.

\begin{table}[!htbp]
    \centering
    \small
    \caption{SAC global default hyperparameters.}
    \label{tab:app_sac_default}
    \begin{tabular}{@{}ll@{}}
        \toprule
        Field & Default Value \\
        \midrule
        \multicolumn{2}{l}{\emph{Runner / Replay}} \\
        \texttt{algo} & sac \\
        \texttt{algo\_log\_name} & fast\_sac \\
        \texttt{seed} & $1$ \\
        \texttt{num\_envs} & $4096$ \\
        \texttt{batch\_size} & $8192$ \\
        \texttt{replay\_buffer\_n} & $512$ \\
        \texttt{updates\_per\_step} & $4$ \\
        \texttt{learning\_starts} & $1$ \\
        \texttt{policy\_frequency} & $4$ \\
        \texttt{env\_steps\_per\_sync} & $1$ \\
        \texttt{max\_iterations} & $500$ \\
        \texttt{save\_interval} & $500$ \\
        \midrule
        \multicolumn{2}{l}{\emph{Network}} \\
        \texttt{actor\_hidden\_dim} & $512$ \\
        \texttt{critic\_hidden\_dim} & $768$ \\
        \texttt{num\_atoms} & $101$ \\
        \texttt{obs\_normalization} & true \\
        \texttt{use\_layer\_norm} & true \\
        \texttt{use\_symmetry} & false \\
        \midrule
        \multicolumn{2}{l}{\emph{Algorithm}} \\
        \texttt{gamma} & $0.97$ \\
        \texttt{tau} & $0.125$ \\
        \texttt{actor\_lr} & $3.0\times10^{-4}$ \\
        \texttt{critic\_lr} & $3.0\times10^{-4}$ \\
        \texttt{algo\_params.alpha\_lr} & $3.0\times10^{-4}$ \\
        \texttt{algo\_params.alpha\_init} & $0.01$ \\
        \texttt{algo\_params.target\_entropy\_ratio} & $0.0$ \\
        \texttt{algo\_params.max\_grad\_norm} & $0.0$ \\
        \texttt{algo\_params.amp\_dtype} & auto \\
        \texttt{algo\_params.use\_compile} & true \\
        \bottomrule
    \end{tabular}
\end{table}

\paragraph{FlashSAC global defaults.}
Table~\ref{tab:app_flashsac_default} gives the resolved FlashSAC defaults. The two recipes differ in actor/critic capacity, replay-buffer warmup length, and the addition of FlashSAC-specific reward / temperature parameters.

\begin{table}[!htbp]
    \centering
    \small
    \caption{FlashSAC global default hyperparameters.}
    \label{tab:app_flashsac_default}
    \begin{tabular}{@{}ll@{}}
        \toprule
        Field & Default Value \\
        \midrule
        \multicolumn{2}{l}{\emph{Runner / Replay}} \\
        \texttt{algo} & flashsac \\
        \texttt{algo\_log\_name} & flash\_sac \\
        \texttt{num\_envs} & $1024$ \\
        \texttt{batch\_size} & $2048$ \\
        \texttt{replay\_buffer\_n} & $512$ \\
        \texttt{updates\_per\_step} & $2$ \\
        \texttt{learning\_starts} & $98$ \\
        \texttt{policy\_frequency} & $2$ \\
        \texttt{max\_iterations} & $5000$ \\
        \texttt{save\_interval} & $1000$ \\
        \midrule
        \multicolumn{2}{l}{\emph{Network}} \\
        \texttt{actor\_hidden\_dim} & $128$ \\
        \texttt{critic\_hidden\_dim} & $256$ \\
        \texttt{num\_atoms} & $101$ \\
        \texttt{obs\_normalization} & false \\
        \texttt{use\_layer\_norm} & false \\
        \texttt{algo\_params.actor\_num\_blocks} & $2$ \\
        \texttt{algo\_params.critic\_num\_blocks} & $2$ \\
        \midrule
        \multicolumn{2}{l}{\emph{Algorithm}} \\
        \texttt{gamma} & $0.97$ \\
        \texttt{tau} & $0.01$ \\
        \texttt{actor\_lr} & $3.0\times10^{-4}$ \\
        \texttt{critic\_lr} & $3.0\times10^{-4}$ \\
        \texttt{algo\_params.normalize\_reward} & true \\
        \texttt{algo\_params.normalized\_g\_max} & $5.0$ \\
        \texttt{algo\_params.actor\_bc\_alpha} & $0.0$ \\
        \texttt{algo\_params.actor\_noise\_zeta\_mu} & $2.0$ \\
        \texttt{algo\_params.actor\_noise\_zeta\_max} & $16$ \\
        \texttt{algo\_params.critic\_min\_v} / \texttt{critic\_max\_v} & $-5.0 / 5.0$ \\
        \texttt{algo\_params.temp\_initial\_value} & $0.01$ \\
        \texttt{algo\_params.temp\_target\_sigma} & $0.15$ \\
        \texttt{algo\_params.temp\_target\_entropy} & null \\
        \texttt{algo\_params.learning\_rate\_init / peak / end} & $3{\times}10^{-4} / 3{\times}10^{-4} / 1.5{\times}10^{-4}$ \\
        \texttt{algo\_params.learning\_rate\_warmup\_steps} & $0$ \\
        \texttt{algo\_params.learning\_rate\_decay\_steps} & $500{,}000$ \\
        \texttt{algo\_params.n\_step} & $1$ \\
        \bottomrule
    \end{tabular}
\end{table}

\paragraph{SAC and FlashSAC overrides across tasks.}
Tables~\ref{tab:app_sac_overrides} and ~\ref{tab:app_flashsac_overrides} summarize the per-task overrides. Fields not listed are inherited from the corresponding default tables. When the two backends differ, the value is written as ``mj / mx''; identical values appear once.

\begin{table}[!htbp]
    \centering
    \small
    \caption{SAC overrides for G1 walk and motion-tracking tasks.}
    \label{tab:app_sac_overrides}
    \begin{tabular}{@{}lccc@{}}
        \toprule
        Field & G1 Walk Flat & G1 Walk Rough & G1 Motion Tracking \\
        \midrule
        \texttt{num\_envs} & $2048$ & $2048$ & $2048$ \\
        \texttt{learning\_starts} & $10 / 1$ & $10 / 1$ & inherited \\
        \texttt{max\_iterations} & $5000$ & $5000$ & $25000$ \\
        \texttt{save\_interval} & $1000$ & $1000$ & $1000$ \\
        \texttt{updates\_per\_step} & $8$ & $8$ & $4$ \\
        \texttt{policy\_frequency} & inherited & inherited & $2$ \\
        \texttt{use\_symmetry} & true / false & true / false & false \\
        \texttt{gamma} & inherited & inherited & $0.99$ \\
        \texttt{tau} & inherited & inherited & $0.05$ \\
        \texttt{num\_atoms} & inherited & inherited & $501$ \\
        \texttt{algo\_params.alpha\_init} & $0.001$ & $0.001$ & $0.1$ \\
        \texttt{algo\_params.target\_entropy\_ratio} & $0.0$ & $0.0$ & $0.5$ \\
        \texttt{algo\_params.max\_grad\_norm} & inherited & inherited & $10.0$ \\
        \bottomrule
    \end{tabular}
\end{table}

G1 Motion Tracking under SAC shares the same environment as the PPO/APPO version; under MotrixSim only the backend identity and the Kp/Kd randomization switches differ from MuJoCoUni.

\begin{table}[!htbp]
    \centering
    \small
    \caption{HORA SAC overrides for Sharpa Inhand Rotation.}
    \label{tab:app_sac_sharpa_hora_overrides}
    \begin{tabular}{@{}ll@{}}
        \toprule
        Field & Sharpa HORA SAC \\
        \midrule
        \texttt{runtime\_impl} & \texttt{hora\_sac} \\
        \texttt{num\_envs} & $1024$ \\
        \texttt{batch\_size} & $2048$ \\
        \texttt{replay\_buffer\_n} & $1280$ \\
        \texttt{training.env\_steps\_per\_sync} & $2$ \\
        \texttt{updates\_per\_step} & $14$ \\
        \texttt{policy\_frequency} & $2$ \\
        \texttt{learning\_starts} & $1$ \\
        \texttt{max\_iterations} & $39063$ \\
        \texttt{save\_interval} & $1000$ \\
        \texttt{actor\_lr}, \texttt{critic\_lr}, \texttt{alpha\_lr} & $4.5{\times}10^{-4}$ \\
        \texttt{training.use\_amp} & true \\
        \texttt{algo\_params.use\_compile} & true \\
        \texttt{actor.priv\_info\_embed\_dim} & $9$ \\
        \texttt{actor.priv\_mlp\_hidden\_dims} & $[256,128,9]$ \\
        \bottomrule
    \end{tabular}
\end{table}

The Sharpa HORA SAC setting keeps the standard SAC replay objective and uses a HORA-style SAC actor that consumes the 9-dimensional privileged tail described in Section~\ref{app:task_dexterous_hand}. Task-side reward, observation, action, and domain-randomization values are therefore documented once in the Sharpa task subsection rather than repeated here.

\begin{table}[!htbp]
    \centering
    \small
    \caption{FlashSAC overrides for G1 Walk Flat and Go2 Joystick Flat.}
    \label{tab:app_flashsac_overrides}
    \begin{tabular}{@{}lcc@{}}
        \toprule
        Field & G1 Walk Flat & Go2 Joystick Flat \\
        \midrule
        \texttt{num\_envs} & $4096$ & $1024$ \\
        \texttt{batch\_size} & inherited & inherited \\
        \texttt{replay\_buffer\_n} & $256$ & $4096$ \\
        \texttt{learning\_starts} & $49$ & $50$ \\
        \texttt{updates\_per\_step} & $8$ & $2$ \\
        \texttt{max\_iterations} & $5000$ & $4000$ \\
        \texttt{save\_interval} & $1000$ & $1000$ \\
        \texttt{tau} & $0.05$ & $0.05$ \\
        \bottomrule
    \end{tabular}
\end{table}

Both FlashSAC tasks are available only under MuJoCoUni.
