# Supplementary material for: UniLab: A Heterogeneous Architecture for Robot RL Beyond GPU-Dominant Paradigms
Source: arXiv:2605.30313 source file (2026-06-02)
Supplement: Supplementary file 2 [file 1_OffPolicyReplayCaseStudy.tex]

\section{Off-Policy Replay Path Case Study}
\label{app:offpolicy_replay_case_study}

% 本节补充主文的 System Attribution 小节，给出 SAC replay-based execution path 的系统归因案例研究。
This section complements the system-attribution analysis in Section~\ref{subsec:end_to_end_training} with a detailed case study of the SAC replay-based execution path.

% 除非另有说明，本节（Appendix~\ref{app:offpolicy_replay_case_study}）所有 timeline statistics 都来自同一台 A100 机器上的 Perfetto traces。该机器使用单张 NVIDIA A100 80GB PCIe GPU、driver 560.35.05、CUDA 12.6、双路 Intel Xeon Gold 5320 CPU 和 188GiB system memory。learner cycle 从一次 learner/weight_sync_write 结束到下一次结束；丢弃前五个 warmup cycles；每个 retained cycle 对应 2048 environment steps；per-cycle 数值报告 retained cycles 的均值。
Unless otherwise stated, all timeline statistics in this section (Appendix~\ref{app:offpolicy_replay_case_study}) are computed from Perfetto traces collected on the same A100 machine: one NVIDIA A100 80\,GB PCIe GPU with driver 560.35.05 and CUDA~12.6, two Intel Xeon Gold 5320 CPUs with 104 logical CPU threads, and 188\,GiB system memory. A learner cycle is measured from the end of one \texttt{learner/weight\_sync\_write} event to the end of the next such event; the first five cycles are discarded as warmup, and each retained cycle corresponds to 2048 environment steps. Reported per-cycle values are means over the retained cycles.

\subsection{Baseline GPU-Cache SAC Path}
\label{app:baseline_gpu_cache_sac}

% 这里先定义 SAC-A：本文中 SAC-A 指用于对比的 straightforward baseline，不是新的 SAC 算法；它对应 sample-before-transfer pipeline 之前的 GPU-cache replay path。这个 baseline 仍然是 heterogeneous design：CPU collector 用 learner 同步来的 actor 权重推进 batched environment 并写入 CPU shared replay storage；learner 在 accelerator 上持有 SAC actor/critic 并周期性把更新后的 actor 权重发回 collector。
We use SAC-A to denote the straightforward SAC baseline used for comparison in this case study, not a separate SAC algorithm. It corresponds to the GPU-cache replay path before the sample-before-transfer pipeline. This baseline is already a heterogeneous design: a CPU collector process runs a CPU actor synchronized from learner weights, advances the batched environment, and writes transitions into shared CPU replay storage. The learner process holds the SAC actor and critic networks on the accelerator and periodically publishes updated actor weights back to the collector. This organization already separates CPU simulation from GPU learning.

% 剩余成本在 replay boundary：CUDA 路径由 learner 维护 device-side replay cache；采样时新增 replay rows 会 lazy sync 到 GPU cache，random indices 被移到 device，然后从 cached replay tensors gather sampled batch，因此 replay-cache maintenance 和 random replay access 进入 learner hot update path。
The remaining cost lies in the replay boundary. In the CUDA path, the learner maintains a device-side replay cache. When the learner samples, newly appended replay rows are lazily synchronized into this GPU cache, random indices are moved to the device, and the sampled batch is gathered from the cached replay tensors before SAC updates are performed. Thus, replay-cache maintenance and random replay access are part of the learner's hot update path. This increases GPU-resident replay storage and inserts replay-management work before the critic, actor, and target-network updates.

\subsection{Sample-Before-Transfer Replay Pipeline}
\label{app:sample_before_transfer}

% \method{} 将 replay boundary 从 replay buffer 移到 sampled batch。collector 继续做 CPU actor inference、environment stepping 和 replay insertion；当 learner 请求下一批训练数据时，collector 在 CPU replay snapshot 上采样并 pack 到两个 shared pack slots 之一，CUDA 下这些 slots 作为 pinned H2D 源，由 learner-side background H2D submit thread 异步传入 cold GPU batch slot，同时 learner 使用当前 hot slot。
\method{} moves the replay boundary from the replay buffer to the sampled batch. The collector still performs CPU actor inference, environment stepping, and replay insertion. Once the learner requests the next training batch, the collector samples rows from a replay snapshot on the CPU and packs them into one of two shared pack slots. On CUDA, these pack slots are registered as pinned host-memory sources for asynchronous H2D transfer. A learner-side background H2D submit thread then transfers the packed batch into the cold GPU batch slot while the learner consumes the current hot slot.

% 这个 distinction 对理解 memory path 很重要：main replay storage 仍然是 CPU shared replay storage；CUDA-specific pinned-memory path 只作用在作为 H2D 源的 shared pack slots。learner 从 hot GPU batch slot 的 device-resident views 读取数据，执行 SAC 更新，并在下一次 batch handoff 交换 hot/cold slots。
This distinction matters for interpreting the memory path. The main replay storage remains CPU shared replay storage; the CUDA-specific pinned-memory path applies to the shared pack slots used as H2D sources. The learner consumes device-resident views from the hot GPU batch slot, executes SAC critic, actor, entropy-temperature, and target-network updates, and swaps the hot and cold slots at the next batch handoff.

% 图~\ref{fig:app_sac_old_new_timeline} 把 baseline 和 double-buffer path 放在同一个 retained learner cycle 时间轴上。图中的 env/replay/H2D/sync/stall/gap 分别表示 environment stepping、replay insertion、host-to-device transfer、actor-weight publication/consumption、等待，以及从 learner weight publication 结束到下一次 learner update 开始之间的 resume gap。关键比较是 replay ownership 和 timing 的变化：baseline 把 replay sampling 和 lazy synchronization 留在 learner hot path，double-buffer path 则提前准备下一批 sampled batch，使 CPU packing 和 H2D transfer 与 GPU learner updates 重叠。
Figure~\ref{fig:app_sac_old_new_timeline} places the baseline and double-buffer paths on the same retained learner-cycle time axis. In the figure, \emph{env}, \emph{replay}, \emph{H2D}, \emph{sync}, \emph{stall}, and \emph{gap} denote environment stepping, replay-buffer insertion, host-to-device transfer, actor-weight publication or consumption, waiting, and the delay from learner weight publication to the next first learner update, respectively. The key comparison is the change in replay ownership and timing: the baseline keeps replay sampling and lazy synchronization on the learner-side critical path, whereas the double-buffer path prepares the next sampled batch early enough to overlap CPU packing and H2D transfer with GPU learner updates.

\begin{figure}[!htbp]
    \centering
    \includegraphics[width=0.85\columnwidth]{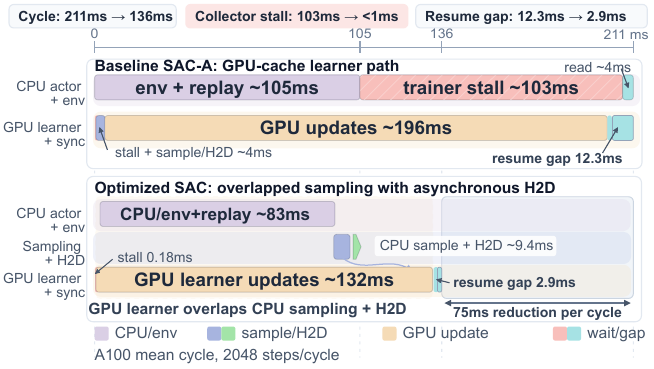}
    \caption{Baseline SAC-A and optimized SAC learner-cycle timelines on A100. Durations are means per retained learner cycle using the cycle definition above; each cycle corresponds to 2048 environment steps. The optimized double-buffer path reduces cycle time from 211\,ms to 136\,ms, collector stall from 103\,ms to below 1\,ms, and resume gap from 12.3\,ms to 2.9\,ms.}
    \label{fig:app_sac_old_new_timeline}
\end{figure}

\subsection{Trace-Based Attribution}
\label{app:trace_based_attribution}

% 本节分析 baseline GPU-cache SAC path 和 \method{} double-buffer path 的 A100 Perfetto traces。这些 traces 提供机制和时序证据，说明 replay sampling、H2D transfer、learner updates 和 weight publication 发生在哪里；由于两个 traces 中 learner update kernels 的时长也不同，归因需要和后续 ablation 一起解释。
We analyze A100 Perfetto traces for the baseline GPU-cache SAC path and the \method{} double-buffer path. These traces provide mechanism and timing evidence: they show where replay sampling, H2D transfer, learner updates, and weight publication occur. Because learner-update kernels also differ in duration across traces, the attribution is interpreted together with the ablation below.

\begin{figure}[!htbp]
    \centering
    \includegraphics[width=\linewidth]{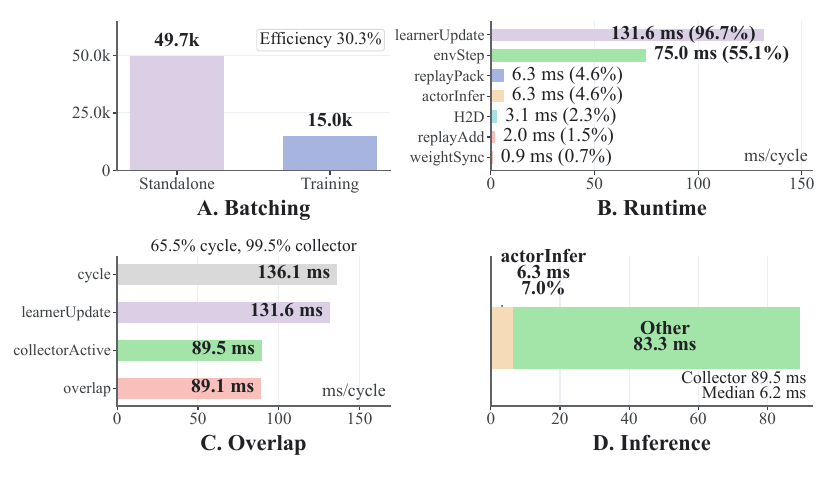}
    % 图注只保留 panel 级读法，详细缩写和统计口径在正文中说明。
    \caption{System-attribution summary for the optimized SAC trace. Panel A reports batching efficiency, with \emph{Eff.} defined as training-pipeline throughput divided by standalone simulator throughput. Panels B--D summarize runtime components, simulation-learning overlap, and collector-side CPU actor-inference cost.}
    \label{fig:app_sac_system_attribution}
\end{figure}

% 图~\ref{fig:app_sac_system_attribution} 从四个互补视角总结 optimized trace：A 面板比较 standalone simulator throughput 和 SAC training pipeline 内的 throughput，Eff. 是两者比值；B--D 面板使用前述 retained learner-cycle 定义并报告 per-cycle means。B 面板中的 Lrn/Env/Pack/Inf/H2D/Add/Sync 分别对应 learner update、environment stepping、CPU replay sampling and batch packing、collector CPU actor inference、host-to-device batch transfer、replay-buffer insertion 和 actor-weight publication/consumption。C 面板把 cycle-level timing terms 汇总为 Cyc/Lrn/Col/Ovl，分别表示 learner-cycle duration、learner-update time、collector-active time 及二者 overlap。D 面板进一步把 collector-active time 与 CPU actor-inference share 分离出来。
Figure~\ref{fig:app_sac_system_attribution} summarizes the optimized trace from four complementary views. Panel A compares standalone simulator throughput with throughput inside the SAC training pipeline; the reported efficiency is their ratio. Panels B--D use the retained learner-cycle definition above and report per-cycle means. In Panel B, \emph{Lrn}, \emph{Env}, \emph{Pack}, \emph{Inf}, \emph{H2D}, \emph{Add}, and \emph{Sync} denote learner update, environment stepping, CPU replay sampling and batch packing, collector CPU actor inference, host-to-device batch transfer, replay-buffer insertion, and actor-weight publication or consumption. Panel C groups the cycle-level timing terms: \emph{Cyc}, \emph{Lrn}, \emph{Col}, and \emph{Ovl} denote learner-cycle duration, learner-update time, collector-active time, and their overlap. Panel D isolates collector-side actor inference by comparing it with total collector-active time.

% 在 traced 500-iteration window 中，double-buffer path 将训练时间从 107.50s 降到 70.58s；丢弃前五个 cycles 后，mean learner cycle 从 211.31ms 降到 136.10ms。每个 cycle 对应 2048 environment steps，因此 throughput 从 9.69k 提升到 15.05k environment steps per second。
In the traced 500-iteration window, the double-buffer path reduces training time from 107.50\,s to 70.58\,s, a 34.34\% reduction in wall-clock time. After dropping the first five cycles, the mean learner cycle decreases from 211.31\,ms to 136.10\,ms. With 2048 environment steps per learner cycle, this corresponds to an increase from 9.69k to 15.05k environment steps per second.

% 最清晰的变化在 replay hot path：baseline 中 learner/replay_sample 平均 3.64ms，并包含 lazy replay synchronization；\method{} 中 learner-side replay consumption 降到 0.23ms。replay preparation 仍然存在，但被移出 learner hot path：CPU packing 为 6.30ms，GPU H2D transfer 为 3.13ms，且 collector-active time 的 99.50% 与 learner updates 重叠；剩余 H2D handoff wait 约为 0.055ms/cycle。
The clearest change is on the replay hot path. In the baseline trace, \texttt{learner/replay\_sample} takes 3.64\,ms on average and includes lazy replay synchronization, with \texttt{replay/h2d\_lazy\_sync} taking 1.88\,ms on the CPU wrapper path and \texttt{gpu/replay\_h2d\_lazy\_sync} taking 1.84\,ms on the GPU event path. In the \method{} trace, learner-side replay consumption is reduced to 0.23\,ms on average. Replay preparation still exists, but it is moved out of the learner hot path: CPU packing takes 6.30\,ms, and GPU H2D transfer takes 3.13\,ms, while 99.50\% of collector-active time overlaps with learner updates. The remaining H2D handoff wait is about 0.055\,ms per cycle.

\subsection{Ablating the Path from GPU-Cache SAC to Sample-Before-Transfer}
\label{app:sac_replay_ablation_c_to_baseline}

% trace-based attribution 给出了 replay path 变化的时序证据，但还需要消融来区分 GPU-cache residency、sampled-batch transfer 和 transfer orchestration。本小节在同一 A100 机器上比较四个 SAC replay path 变体；这些变体保持 SAC objective 和 update equations 不变，只移动 replay boundary。
The trace-based attribution gives timing evidence for the replay-path change, but it does not by itself separate replay-data residency from transfer orchestration. We run a SAC replay-path ablation on the same A100 machine. The four variants preserve SAC's objective and update equations; only the replay boundary changes, moving from learner-side GPU-cache replay to sampled-batch transfer and then to the CPU-pinned double-buffer path.

% 四个变体构成一条受控迁移链。C 是 old-SAC-like GPU-cache compatibility control，保留 learner-side GPU replay cache、lazy sync newly appended replay rows 和 GPU-cache random gather；B 保留 GPU-cache replay，但使用现代 ablation framework，因此主要体现 GPU-cache 路径中的调度改善；A 移除 GPU-cache residency，转为 sampled-batch transfer，但没有完整 pinned/asynchronous overlap；baseline 在 A 的 CPU-resident sampled-batch 边界上加入 pinned pack slots、one-tick async H2D 和 hot/cold GPU batch slots。
The variants form a controlled migration chain. C is the old-SAC-like GPU-cache compatibility control: replay samples are still served through a learner-side GPU replay cache with lazy synchronization of newly appended rows and random gather from cached replay tensors. B keeps the same GPU-cache replay organization, but uses the modern ablation framework; its improvement over C therefore primarily reflects scheduling and runner-level overlap rather than a change in replay residency. A removes the GPU-cache resident replay component and moves the boundary to sampled-batch transfer, but it uses a synchronous/pageable transfer path rather than the full pinned asynchronous pipeline. The baseline keeps A's CPU-resident sampled-batch boundary and adds registered pinned pack slots, one-tick asynchronous H2D, and hot/cold GPU batch slots.

% 图中的统计口径也需要明确。Panel A 的 E2E 结果报告三次 seed 的均值和 sample standard deviation；Panel B 报告 learner-cycle median 和 p95；Panel C 区分 learner/replay_sample 事件和 learner-side boundary wait，其中 GPU wait 不是 kernel-level GPU idle；Panel D 报告 peak CUDA reserved memory，并把 learner-side GPU replay cache 贡献的部分单独列为 GPU-cache component。
The figure reports four complementary measurements. Panel A reports wall-clock E2E time as means over three seeds, with sample-standard-deviation error bars. Panel B reports learner-cycle medians, with diamonds marking p95 cycle time. Panel C focuses on the learner-side replay boundary. We report \emph{Replay sample mean} using the learner-side \texttt{learner/replay\_sample} event: in GPU-cache variants, this event includes learner-side sampling, gather, and lazy replay-cache synchronization; in sampled-batch variants, it measures the learner-side batch handoff and consumption path, not the CPU packing work that is scheduled earlier. \emph{GPU wait mean} reports learner-side boundary waiting before update computation, including waiting for data or replay-batch readiness, and should not be read as total kernel-level GPU idle time. The black marks indicate the corresponding medians. Panel D reports the mean peak CUDA reserved memory and separates the replay-cache portion as the GPU-cache component. This component is present in C and B because the learner maintains a full GPU replay cache, and absent in A and the baseline because they keep replay CPU-resident and retain only sampled GPU batch slots.

\begin{figure}[!htbp]
    \centering
    \includegraphics[width=\linewidth]{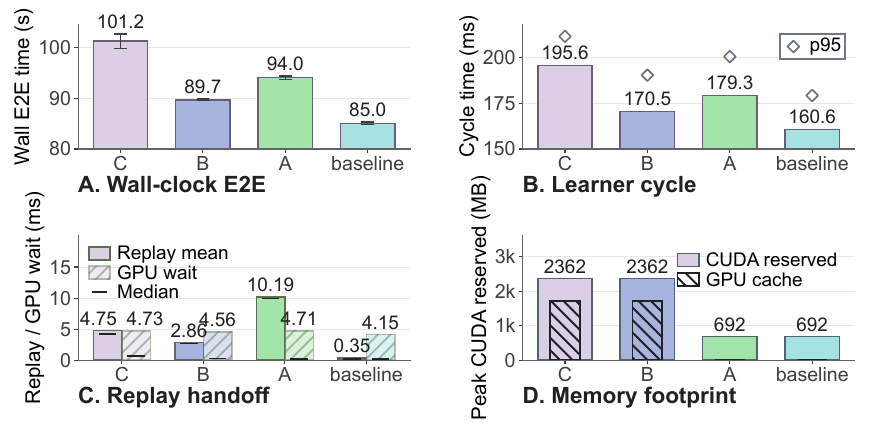}
    \caption{C-to-baseline ablation for the SAC replay path. Wall-clock E2E bars are three-seed means with sample-standard-deviation error bars. Learner-cycle bars are medians, with diamonds marking p95 cycle time. Panel C reports learner-side replay-sample and boundary-wait statistics; Panel D reports peak CUDA reserved memory and the measured GPU-cache component.}
    \label{fig:app_sac_replay_ablation}
\end{figure}

% 结果显示，不同技术差距对应不同指标变化。C 到 B 改善 E2E，主要来自 GPU-cache family 内部的调度改善；B 到 A 移除 GPU-cache component，显著降低 CUDA reserved memory，但同步/pageable sampled-batch handoff 暴露在 learner boundary 上，导致 replay sample time 和 E2E 变差；A 到 baseline 不重新引入 GPU cache，而是优化 transfer orchestration，因此恢复吞吐并保持低显存。
With these definitions, Figure~\ref{fig:app_sac_replay_ablation} shows that the variants affect different metrics for different reasons. Moving from C to B improves wall-clock time within the GPU-cache family, while CUDA reserved memory remains unchanged; this is consistent with a scheduling improvement rather than a memory-residency change. Moving from B to A removes the measured GPU-cache component and reduces peak CUDA reserved memory from 2362\,MB to 692\,MB, but the synchronous/pageable sampled-batch handoff becomes visible on the learner boundary, increasing replay-sample time and hurting E2E time. Moving from A to the baseline keeps the low-memory CPU-resident replay design and changes the transfer mechanism instead: pinned shared pack slots, one-tick asynchronous H2D, and hot/cold GPU slots reduce learner-side replay consumption from 10.19\,ms to 0.35\,ms and reduce wall time from 94.04\,s to 85.04\,s without reintroducing the GPU-cache component. Relative to C, the final baseline reduces wall time from 101.23\,s to 85.04\,s while also removing the measured GPU-cache footprint.

% 因此，消融把 trace-based attribution 与端到端收益连接起来：收益来自 replay runtime boundary 的重放置，而不是 SAC loss 的改变。replay work 仍然存在，但 ownership 和 timing 发生转移，使 learner 消费 ready device batches，而不是在 hot path 中维护和采样 capacity-scaled GPU replay cache。
This ablation connects the trace-based attribution to the end-to-end result. The gain comes from relocating the replay-runtime boundary, not from changing the SAC loss. Replay work remains, but shifts in ownership and timing: the learner consumes ready device batches instead of maintaining and sampling a capacity-scaled GPU replay cache on the hot update path.
\begin{figure}[!htbp]
    \centering
    \includegraphics[width=\columnwidth]{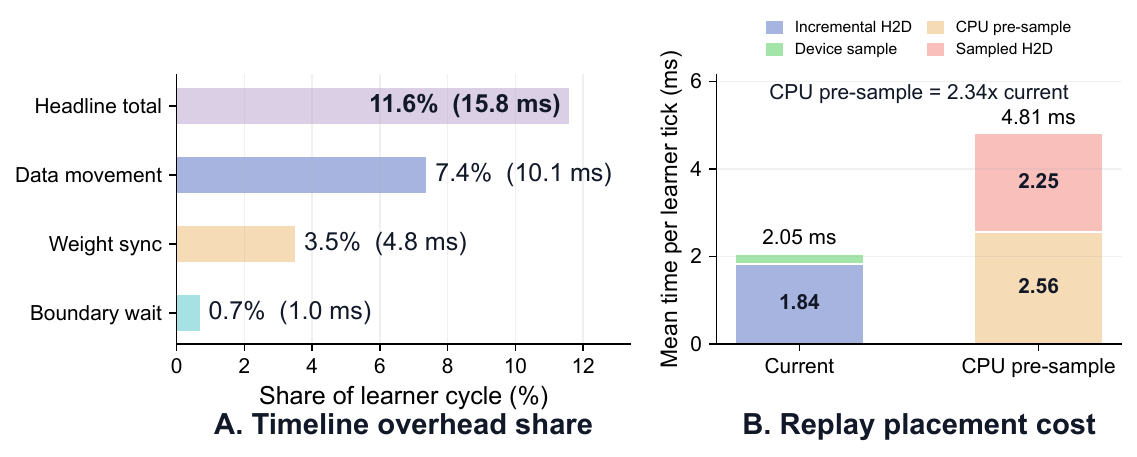}
    \caption{SAC buffer and communication overhead. Values in Panel A are means per retained learner cycle from the optimized SAC timeline; Panel A groups counted data-movement, weight-synchronization, and boundary-wait overhead by share of the mean learner cycle, with signal-ready context shown separately. Panel B reports an auxiliary replay-placement benchmark comparing current incremental-transfer/device-sampling and CPU pre-sample plus sampled-batch H2D schemes.}
    \label{fig:app_sac_buffer_communication}
\end{figure}

\subsection{Buffer and Communication Overhead}
\label{app:buffer_communication_overhead}

% 图~\ref{fig:app_sac_buffer_communication} 分解 optimized SAC timeline 中的数据移动、同步和残余等待，并把计入 headline overhead 的项与只作为调度/背压上下文报告的项分开。Data movement 包括 CPU-side replay sampling and packing、H2D submission、H2D transfer 和 transfer-completion wait；weight sync 包括 learner weight publication、D2H weight copy 和 collector-side weight read/update checking；boundary wait 包括 collector 和 learner 在 cycle boundary 的等待。Signal-ready context 单独报告：collector 已经准备好下一批数据并发出 ready signal，但 learner 尚未到达下一次 batch boundary；它表示 scheduling/backpressure slack，而不是额外 data-copy cost 或 learner-update waiting。
Figure~\ref{fig:app_sac_buffer_communication} combines a timeline overhead breakdown with an auxiliary replay-placement benchmark. Panel~A breaks down the data movement, synchronization, and residual waiting observed inside the optimized SAC timeline. We separate the counted overhead into three groups. \emph{Data movement} covers CPU-side replay sampling and batch packing, H2D submission, H2D transfer, and transfer-completion wait. \emph{Weight sync} covers learner weight publication, device-to-host (D2H) weight copy, and collector-side weight read/update checking. \emph{Boundary wait} covers collector and learner waiting at the cycle boundary. The figure also reports signal-ready context separately: the collector has already prepared the next batch and issued a ready signal, while the learner has not yet reached the next batch boundary. We treat this interval as scheduling and backpressure context rather than data-copy cost or learner-update waiting, so it is excluded from the counted overhead total.

% 在该 trace 中，主要计入的 data-movement、synchronization 和 boundary-wait overhead 合计为 15.82ms/cycle，即 136.10ms mean learner cycle 的 11.62%。其中 data movement 为 10.07ms/cycle，weight synchronization 为 4.79ms，residual boundary waiting 为 0.96ms。Signal-ready interval 较大但不计入 headline total，因为它描述 readiness/backpressure context，而不是直接 data-copy 或 learner-wait cost。
In this trace, the counted data-movement, synchronization, and boundary-wait overhead total is 15.82\,ms per cycle, or 11.62\% of the 136.10\,ms mean learner cycle. Data movement is the largest counted component at 10.07\,ms per cycle, weight synchronization contributes 4.79\,ms, and residual boundary waiting contributes 0.96\,ms. The signal-ready interval is larger, but it is reported outside the headline total because it describes readiness and backpressure context rather than a direct data-copy or learner-wait cost.

% Panel B 是同配置下的辅助 replay-placement benchmark，不属于 Panel A 的 retained-cycle overhead 汇总。该 benchmark 中 current placement 由 incremental H2D 和 device-side random sampling 组成，为 2.05ms/learner tick；CPU pre-sample plus sampled-batch H2D placement 为 4.81ms/learner tick，即 current placement 的 2.34x。这个结果说明 placement cost 需要和 overlap/scheduling 一起解释，而不能只看孤立的数据移动时间。
Panel B provides an auxiliary replay-placement benchmark under the same configuration, separate from the retained-cycle accounting in Panel~A. In this benchmark, the current placement combines incremental H2D with device-side random sampling and costs 2.05\,ms per learner tick. A CPU pre-sample plus sampled-batch H2D placement costs 4.81\,ms per learner tick, or 2.34$\times$ the current placement cost. This comparison is not part of the counted timeline overhead; instead, it shows why replay placement must be interpreted together with the overlap and scheduling structure of the full pipeline.

\begin{table*}[!t]
\centering
\small
\captionsetup{hypcap=false}

\setlength{\emergencystretch}{2em}
\hyphenpenalty=10000
\exhyphenpenalty=10000
\newcolumntype{L}[1]{>{\raggedright\arraybackslash\hyphenpenalty=10000\exhyphenpenalty=10000}p{#1}}

\caption{Trace-based attribution summary for the SAC replay path. The table reports what can be supported directly by the A100 timeline traces and where additional evidence is needed.}
\label{tab:sac_trace_attribution}

\begin{tabular}{@{}L{0.20\textwidth}L{0.34\textwidth}L{0.13\textwidth}L{0.25\textwidth}@{}}
    \toprule
    Mechanism & Evidence from traces & Strength & Safe interpretation \\
    \midrule
    End-to-end cycle reduction &
    Traced window decreases from 107.50\,s to 70.58\,s; post-warmup cycle decreases from 211.31\,ms to 136.10\,ms. &
    Strong &
    The double-buffer path is 1.52$\times$ faster over the traced window and 1.55$\times$ faster per post-warmup cycle. \\
    \midrule
    Learner replay hot path &
    \texttt{learner/replay\_sample} decreases from 3.64\,ms to 0.23\,ms on average. &
    Strong &
    Replay sampling no longer dominates the learner-side handoff before SAC updates. \\
    \midrule
    Collector-side CPU packing &
    Optimized trace records CPU-side replay packing with 32768 sampled transitions per batch. &
    Strong &
    Random replay packing is performed on the CPU side before transfer. \\
    \midrule
    Asynchronous H2D preparation &
    CPU pack takes 6.30\,ms and GPU H2D takes 3.13\,ms; 99.50\% of collector-active time overlaps with learner updates. &
    Strong &
    Replay preparation is still present, but it is largely hidden behind GPU learner computation. \\
    \midrule
    Hot/cold GPU batch slots &
    Optimized trace records alternating hot/cold batch-slot swaps between the two device slots. &
    Strong &
    The learner consumes one device batch while the next batch is prepared in the cold slot. \\
    \midrule
    Pinned shared pack slots &
    Trace metadata reports registered pinned shared host memory, with pinned and direct-pinned flags enabled. &
    Medium--strong &
    The trace supports pinned H2D source slots; the implementation should be cited for the \texttt{cudaHostRegister} detail. \\
    \midrule
    Actor-weight publication &
    \texttt{learner/weight\_sync\_write} decreases from 1.71\,ms to 0.94\,ms; weight-copy events remain visible. &
    Strong &
    Actor-weight publication remains a synchronous boundary, although it is small in this trace. \\
    \midrule
    GPU replay memory footprint &
    The new trace transfers 56.36\,MB for 32768 samples; two sampled batch slots are about 112.7\,MB under this layout. &
    Estimate &
    This supports a memory-footprint estimate, not a measured peak-memory claim. \\
    \bottomrule
\end{tabular}

\vspace{0.4\baselineskip}
\end{table*}

\subsection{What the Traces Do and Do Not Establish}
\label{app:trace_scope}

% traces 支持 execution-path change 及其 timing consequences，但不能单独支持 peak memory、exact H2D volume 或 cross-algorithm generality 等更强归因。
The traces establish the execution-path change and its timing consequences: replay preparation moves from learner-side GPU-cache sampling to collector-side CPU packing plus asynchronous H2D staging, new-batch preparation is almost fully overlapped with learner computation, and actor-weight publication remains an explicit synchronization boundary. They do not, by themselves, establish stronger claims about peak GPU memory, exact H2D volume reduction, or cross-algorithm generality; those claims require memory counters, byte counters for the baseline lazy-sync path, or corresponding TD3 / FlashSAC measurements.
