# Supplementary material for: UniLab: A Heterogeneous Architecture for Robot RL Beyond GPU-Dominant Paradigms
Source: arXiv:2605.30313 source file (2026-06-02)
Supplement: Supplementary file 3 [file 2_DomainRandomization.tex]

\section{Domain Randomization Backends and Lifecycle}
\label{app:domain_randomization}

% \method{} 中的域随机化是任务和后端之间的契约，而不是算法层的新机制。
% 任务侧 provider 负责采样 workload 相关的随机变量，仿真后端声明自己能应用哪些物理参数覆盖。
% 运行时的 DomainRandomizationManager 负责校验契约、在 materialize 前应用 cold-start 模型变体、在 sparse reset 中注入 reset payload，并在物理步进前调度 interval 扰动。
% 这样，随机化就和状态 reset 与批量仿真的生命周期绑定在一起。
Domain randomization in \method{} is implemented as a task/backend contract rather
than as an algorithm-level feature.  A task-owned
\texttt{DomainRandomizationProvider} samples the quantities that are meaningful
for the workload, while the simulator backend advertises which physical
overrides it can apply.  The runtime mediator,
\texttt{DomainRandomizationManager}, validates this contract, applies
cold-start model variants before backend materialization, injects reset
payloads into sparse environment resets, and schedules interval perturbations
before physics stepping.  This keeps randomization tied to the same lifecycle
that already controls state reset and batched simulation.

\subsection{Runtime Lifecycle}
\label{app:dr_runtime_lifecycle}

% 表格~\ref{tab:app_dr_lifecycle} 区分当前实现中的生命周期阶段。
% 关键系统细节是 reset-time randomization 是 sparse 的：只有 \texttt{env\_ids} 中的环境会收到新的状态和新的随机化 payload。
% interval randomization 则不同，它在每个 vectorized env step 前检查一次，并发生在后端推进物理之前。
% observation noise 和 command sampling 属于任务侧逻辑，不需要后端物理参数覆盖。
Table~\ref{tab:app_dr_lifecycle} separates the lifecycle stages used by the
current implementation.  The important systems detail is that reset-time
randomization is sparse: only the environments listed in \texttt{env\_ids}
receive a new state and a new randomization payload.  Interval randomization is
different: it is checked once per vectorized environment step, before the
backend advances physics.  Per-observation noise and command sampling are
task-side operations and do not require backend-specific physical overrides,
although they may depend on backend sensor reads that must complete first.

\begin{table*}[t]
\centering
\small
\captionsetup{hypcap=false}

\setlength{\tabcolsep}{3pt}
\begin{tabular}{@{}
>{\raggedright\hyphenpenalty=10000\exhyphenpenalty=10000\arraybackslash}p{0.13\textwidth}
>{\raggedright\hyphenpenalty=10000\exhyphenpenalty=10000\arraybackslash}p{0.21\textwidth}
>{\raggedright\hyphenpenalty=10000\exhyphenpenalty=10000\arraybackslash}p{0.21\textwidth}
>{\raggedright\hyphenpenalty=10000\exhyphenpenalty=10000\arraybackslash}p{0.30\textwidth}@{}}
\toprule
\textbf{Lifecycle} & \textbf{Trigger} & \textbf{Owner} & \textbf{Randomized state} \\
\midrule
Backend initialization & DR init hook before backend
\texttt{materialize()} & Task provider builds an init plan; backend
materializes variants & Persistent
model or geometry variants assigned per environment, such as object-scale
variants expressed through \texttt{GeomSizeOverride}. \\
\midrule
Sparse reset & Environment creation and any later reset of terminated or
truncated \texttt{env\_ids} & Task provider samples reset state and optional
reset payload; backend applies supported fields & Initial
pose, velocity, commands, cached object/grasp state, mass, COM, gravity,
friction, actuator gains, and other supported physical fields. \\
\midrule
Scheduled interval & Each vectorized \texttt{step}; active at the configured
interval or when an equivalent task plan is non-empty & Task provider builds an
interval plan; backend
stages the perturbation for the upcoming physics step & Push forces and
body-force perturbations.  The current capability contract includes body
velocity deltas, but neither backend advertises support for them. \\
\midrule
Observation construction & Every task observation update & Task code & Actor
observation noise, history/bias terms, and task-specific observation
perturbations.  These are backend-independent unless they require backend
sensors to be read first. \\
\midrule
Evaluation and playback & Same environment contract as training unless the
configuration is changed & Training/evaluation entrypoint and task config &
The backend does not reinterpret randomization for evaluation; training and
evaluation share the same environment contract to avoid implicit behavioral
differences between the two modes.  Deterministic runs should disable the
relevant task switches or set degenerate ranges and fixed seeds. \\
\bottomrule
\end{tabular}
\caption{Domain-randomization lifecycle used by the current \method{} runtime.}
\label{tab:app_dr_lifecycle}
\end{table*}

\subsection{Backend Implementation}
\label{app:dr_backend_implementation}

\noindent\textbf{MuJoCoUni.}
% MuJoCoUni 遵循 MuJoCoUni 参考文稿中的 reset-lifecycle 设计：
% \texttt{BatchEnvPool.reset(env\_ids, initial\_state, randomization=None)} 同时接收新的 physics state 和可选的 model-field patch 字典。
% 每个 payload 的首维都是 \texttt{len(env\_ids)}，因此 reset 成本和随机化工作量随实际终止环境数缩放。
% 影响 MuJoCo 派生常量的字段会先 patch 再通过 \texttt{mj\_setConst} 刷新，其他字段直接写入并进入 reset/forward 路径。
% 几何级变化在 runtime execution 前通过编译兼容模型变体并给每个 vectorized environment 分配变体来表达。
MuJoCoUni implements reset-time randomization through
\texttt{BatchEnvPool.reset(env\_ids, initial\_state, randomization=None)}
which receives both the new physics state and an optional dictionary of model-field
patches.  Each payload has leading dimension \texttt{len(env\_ids)}, so reset
cost and randomization work scale with the number of environments that actually
terminate.  Fields that affect MuJoCo derived constants are patched before the
reset/forward path and refreshed with \texttt{mj\_setConst}; other fields are
written directly.  Geometry-level changes are handled before runtime execution by
compiling compatible model variants and assigning each vectorized environment
to one variant before the pool is materialized.

\noindent\textbf{MotrixSim.}
% MotrixSim 通过 MotrixSim 原生 override API 实现同一个 task/backend contract。
% 在 \texttt{set\_state} 中，后端 reset 被选中的 data slice，清除这些环境上暂存的 body force，应用 init-time geometry-size override，再应用支持的 reset randomization，随后写入新的 DOF state 并执行 forward kinematics。
% mass 和 COM 随机化使用 link mass 与 center-of-mass override。
% friction、gravity 和 actuator-gain randomization 是条件能力：只有加载的 MotrixSim model 暴露对应 override method 时才启用，并且 gain randomization 要求所有 actuator 都是 position actuator。
% object 或 geom-size 变体通过每环境 size override 表达，而不是通过独立的 MuJoCo model binary。
MotrixSim implements the same task/backend contract with MotrixSim-native
override APIs.  During \texttt{set\_state}, the backend resets the selected data
slice, clears staged body forces for those environments, applies init-time
geometry-size overrides, applies supported reset randomization, writes the new
DOF state, and runs forward kinematics.  Mass and COM randomization use link
mass and center-of-mass overrides.  Friction, gravity, and actuator-gain
randomization are conditional capabilities: they are enabled only when the
loaded MotrixSim model exposes the corresponding override methods, and
gain randomization requires all actuators to be position actuators.  Object or
geom-size variants are represented as per-environment size overrides rather
than separate MuJoCo model binaries.

\subsection{Supported Randomization Families}
\label{app:dr_supported_families}

% 表格~\ref{tab:app_dr_backend_capabilities} 汇总后端能力和当前任务侧覆盖范围。
% 表格刻意区分“后端能否应用某个字段”和“某个任务配置是否启用了该字段”。
% 当任务请求后端不支持的 reset term 时，manager 会过滤不支持的 reset payload entry 并记录日志；部分任务 provider 如果认为该 term 对 workload 必需，也会在 validate 阶段直接失败。
Table~\ref{tab:app_dr_backend_capabilities} lists backend capabilities and
current task-side coverage.  The table distinguishes a backend's ability to
apply a field from whether a particular task configuration enables that field.
When a task requests reset terms that a backend does not support, the manager
filters unsupported reset payload entries and logs the skipped terms; some task
providers additionally fail validation when the term is required for that
workload.

\begin{table*}[t]
\centering
\scriptsize
\captionsetup{hypcap=false}

\setlength{\tabcolsep}{3pt}
\begin{tabular}{@{}
>{\raggedright\hyphenpenalty=10000\exhyphenpenalty=10000\arraybackslash}p{0.13\textwidth}
>{\raggedright\hyphenpenalty=10000\exhyphenpenalty=10000\arraybackslash}p{0.08\textwidth}
>{\raggedright\hyphenpenalty=10000\exhyphenpenalty=10000\arraybackslash}p{0.18\textwidth}
>{\raggedright\hyphenpenalty=10000\exhyphenpenalty=10000\arraybackslash}p{0.18\textwidth}
>{\raggedright\hyphenpenalty=10000\exhyphenpenalty=10000\arraybackslash}p{0.31\textwidth}@{}}
\toprule
\textbf{Family} & \textbf{Lifecycle} & \textbf{MuJoCoUni} & \textbf{MotrixSim} & \textbf{Current task coverage} \\
\midrule
Model or geometry variants & Init & Precompiled \texttt{MjModel} variants
with per-env assignments. & Per-env geometry-size overrides applied to the
MotrixSim data/model path. & Sharpa in-hand object-scale variants. \\
\midrule
Initial state and task conditions & Reset & Backend receives the sampled
\texttt{qpos}/\texttt{qvel}; task provider owns pose, velocity, command, grasp,
motion-frame, and terrain-spawn sampling. & Same task-level reset contract
after conversion to MotrixSim DOF layout. & Locomotion commands and spawn pose;
motion-tracking reference frames; in-hand grasp/object resets. \\
\midrule
Base/body mass & Reset & \texttt{base\_mass\_delta} and full
\texttt{body\_mass}. & Base-link mass delta and full link-mass override. &
Locomotion, manipulation-locomotion, motion tracking, and dexterous-hand tasks
where config enables mass DR. \\
\midrule
Base/body COM & Reset & \texttt{base\_com\_offset} and full
\texttt{body\_ipos}. & Base-link COM offset and full link COM override. &
Locomotion, motion tracking, and hand/object tasks where config enables COM
DR. \\
\midrule
Gravity & Reset & \texttt{gravity} payload. & Conditional gravity override
support. & Motion-tracking and dexterous-hand
configs that enable gravity or gravity-direction DR. \\
\midrule
Contact friction & Reset & Full \texttt{geom\_friction} payload. &
Conditional collision-geom friction overrides; non-collision geoms must remain
at defaults because the MotrixSim friction override API is only exposed on
geoms with nonzero collision group or affinity. & Ground friction in manipulation-locomotion; foot friction in G1
tracking; object friction in dexterous-hand tasks. \\
\midrule
Actuator gains & Reset & \texttt{kp} and \texttt{kd} payloads for position
actuators. & Conditional per-actuator Kp/damping overrides; available only for
all-position-actuator models. & Go2/G1 locomotion and tracking tasks when
\texttt{randomize\_kp} or \texttt{randomize\_kd} is enabled. \\
\midrule
Inertia and armature & Reset & \texttt{body\_iquat},
\texttt{body\_inertia}, and \texttt{dof\_armature}. & Not advertised in the
current capability set. & Armature randomization is used by
manipulation-locomotion configs when enabled; body inertial tensors are backend
capability rather than broad task coverage. \\
\midrule
External perturbations & Interval & Push and arbitrary body-force payloads are
staged through \texttt{xfrc\_applied}. & Push forces are supported through link
external force; arbitrary body force is conditional on link
\texttt{add\_external\_force}. & Locomotion push perturbations; Sharpa object
force perturbations. \\
\midrule
Observation noise and biases & Observation step or reset & Task-side NumPy
noise after backend sensor reads. & Same task-side path. & Locomotion actor
noise; G1 tracking actor noise and reset biases; hand joint/contact observation
noise where configured. \\
\bottomrule
\end{tabular}
\caption{Supported domain-randomization families and backend-specific limits.}
\label{tab:app_dr_backend_capabilities}
\end{table*}

\subsection{Implications for Cross-Backend Experiments}
\label{app:dr_cross_backend_implications}

% 共享契约让任务可以用同一套接口表达随机化，但实际生效的随机化集合仍然依赖后端。
% 因此在跨后端实验中，我们需要把 resolved task configuration 和 backend capabilities 分开报告。
% 只有当任务配置启用某个随机化项，并且所选后端声明支持对应字段时，该随机化项才应被解释为 active。
% 这一区分对公平比较很重要：例如 MuJoCoUni 暴露更宽的 inertial reset-field surface，而 MotrixSim 在加载模型支持对应 override API 时，可以通过 link、geom、gravity、actuator 和 external-force override 匹配许多常见 locomotion 与 manipulation 设置。
The shared contract lets a task express randomization once, but the effective
randomization set is still backend-dependent.  For cross-backend experiments,
we therefore report the resolved task configuration separately from backend
capabilities.  A randomization item should be interpreted as active only when
the task configuration enables it and the selected backend advertises support
for the corresponding field.  This distinction matters for fair comparison:
for example, MuJoCoUni exposes a wider reset-field surface for inertial fields,
whereas MotrixSim can match many common locomotion and manipulation settings
through link, geom, gravity, actuator, and external-force override APIs when
the loaded model supports them.
