# Supplementary material for: UniLab: A Heterogeneous Architecture for Robot RL Beyond GPU-Dominant Paradigms
Source: arXiv:2605.30313 source file (2026-06-02)
Supplement: Supplementary file 4 [file 3_TrainingCurves.tex]

\section{Task and Algorithm Details}
\label{app:training_curves}

\subsection{Training Curves}
\label{app:training_curves_figures}

This subsection collects per-task training curves for the three on-policy and off-policy algorithm families used in the main paper. Each panel plots episode reward against environment steps; the curves are aggregated over seeds and smoothed with a fixed-width moving average. Rewards use the same task-side scales as in Section~\ref{app:training_curves_tasks}, so absolute values are comparable across seeds for the same task but not across tasks. The task subsets shown for each algorithm match the per-task override tables in Section~\ref{app:training_curves_algorithms}: PPO is reported on all sixteen benchmark tasks, APPO on the six tasks with a registered APPO configuration, and SAC / FlashSAC on the five tasks with a replay configuration.

\begin{figure}[H]
    \centering
    \includegraphics[width=0.95\textwidth]{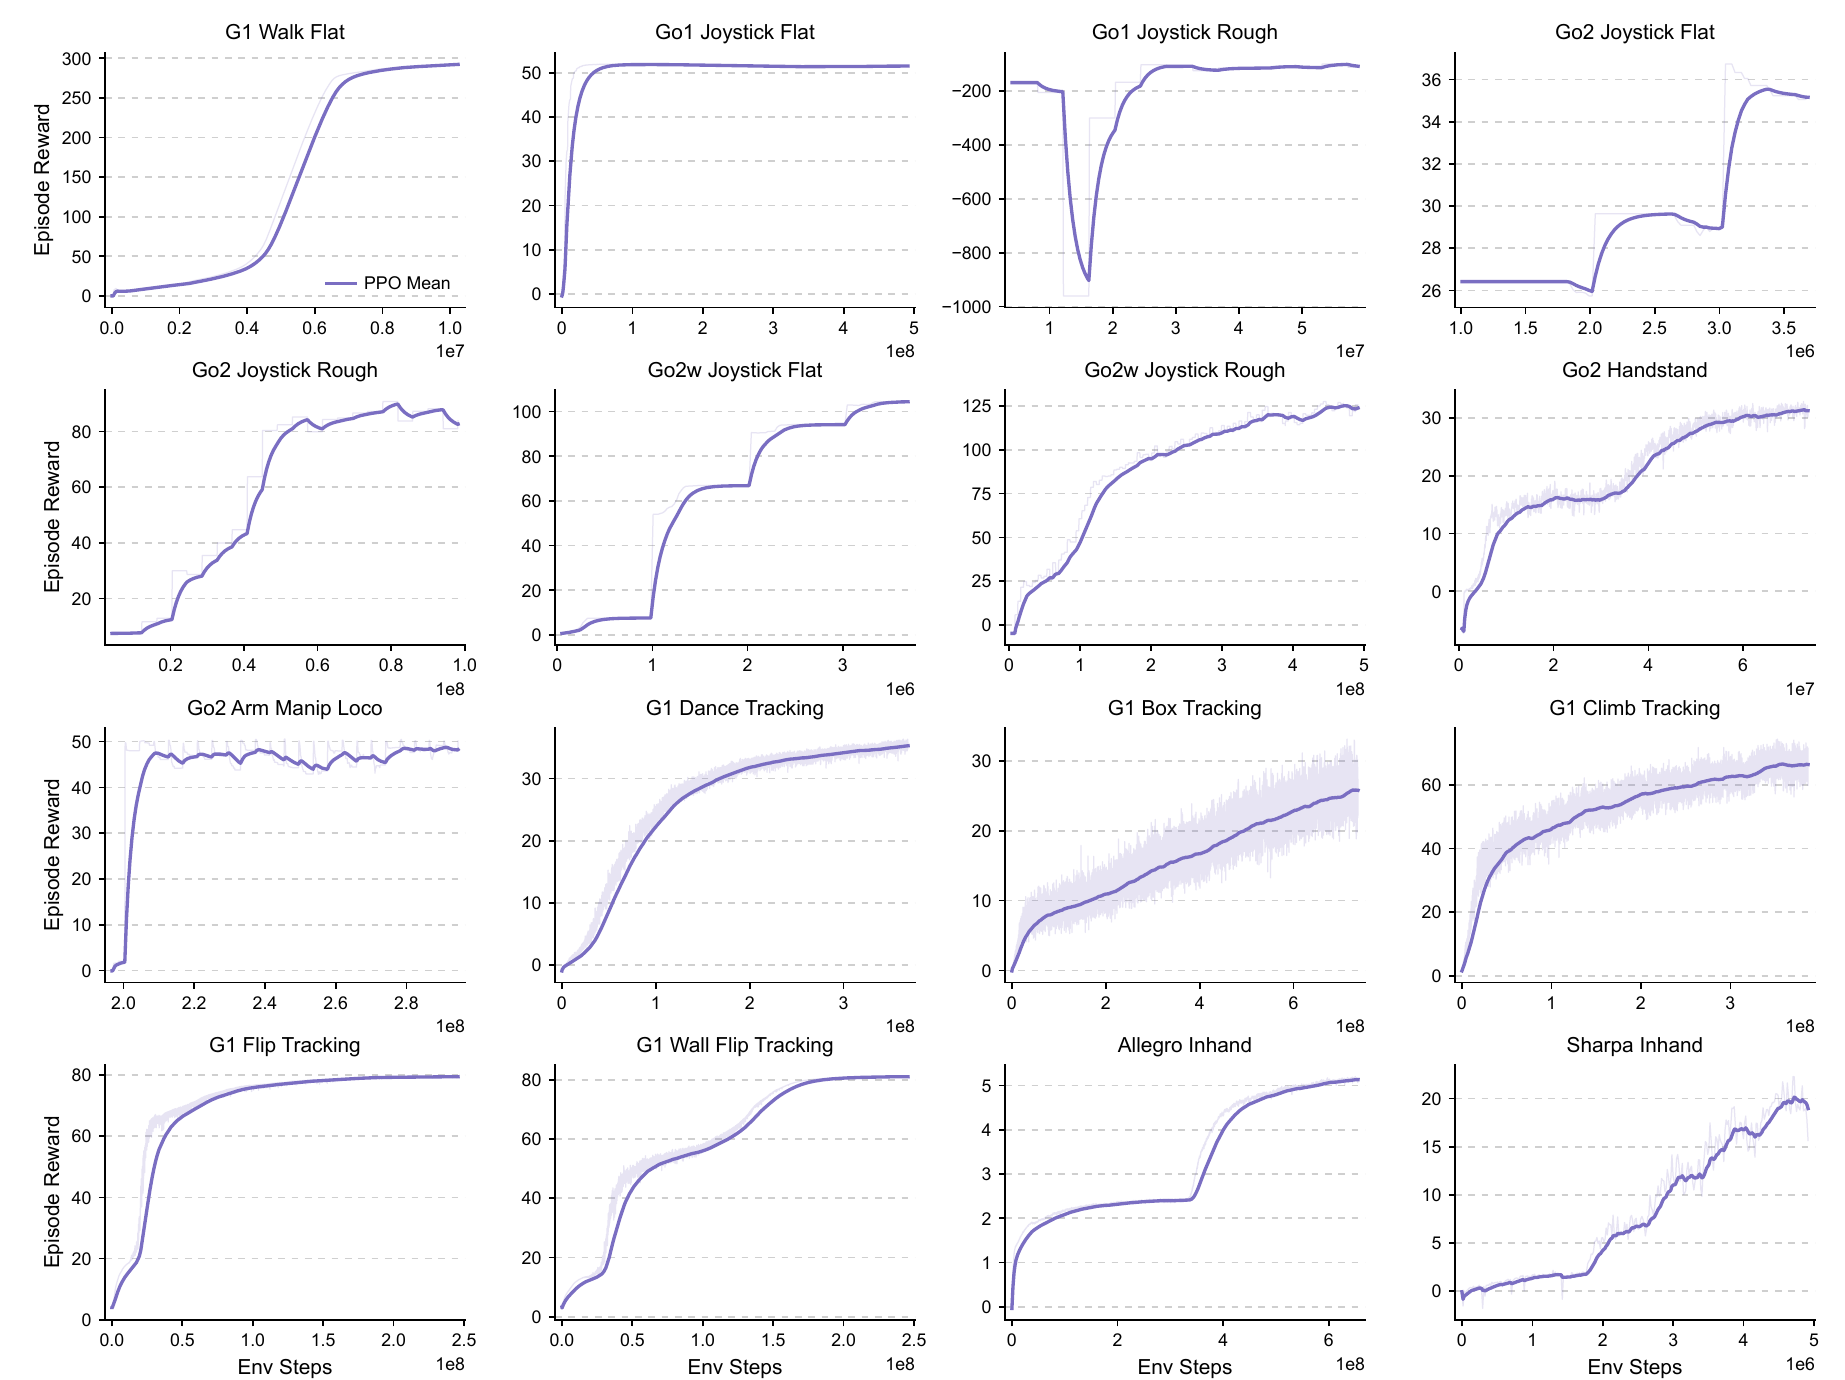}
    \caption{PPO training curves across the sixteen benchmark tasks. Each panel reports episode reward against environment steps; the $x$-axis units differ per panel because environment-step budgets are task-dependent (see Section~\ref{app:training_curves_algorithms}).}
    \label{fig:app_ppo_task_grid}
\end{figure}

\begin{figure}[H]
    \centering
    \includegraphics[width=0.95\textwidth]{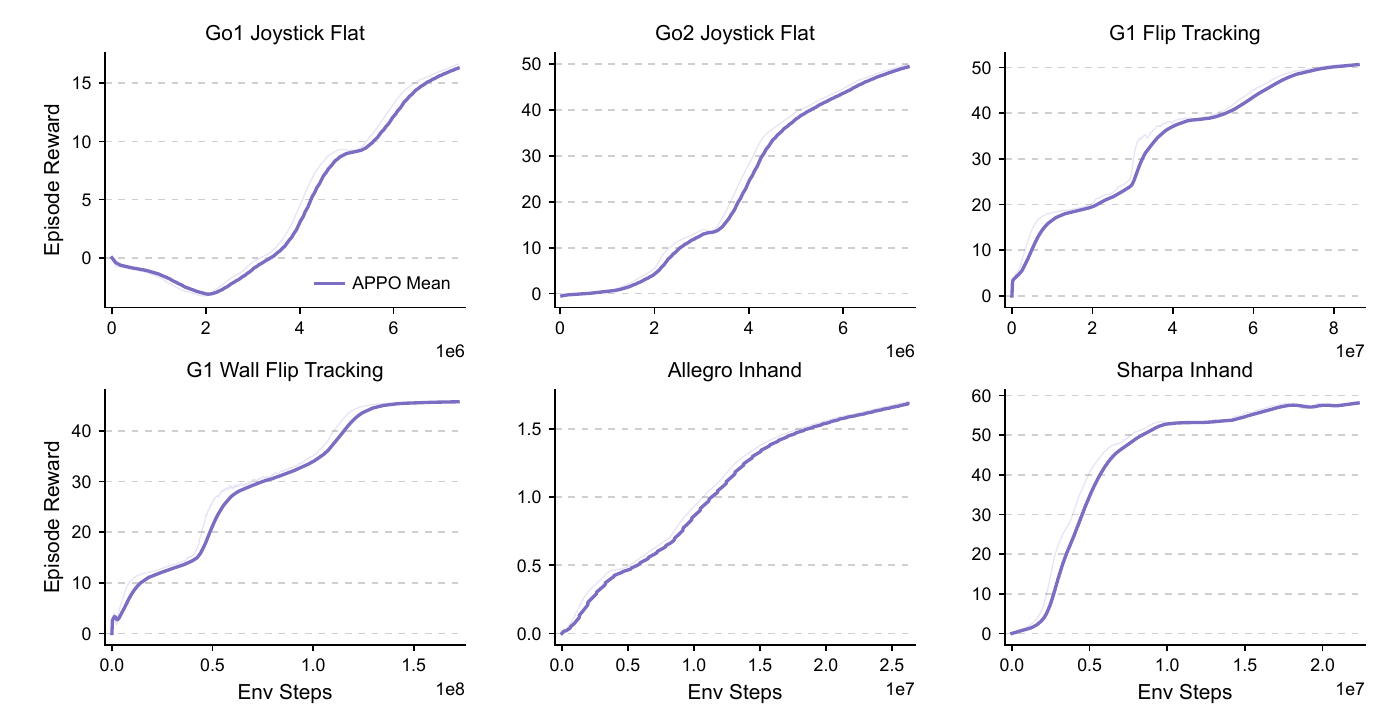}
    \caption{APPO training curves for the six tasks with a registered APPO configuration: Go1 / Go2 Joystick Flat, G1 Flip and Wall Flip Tracking, Allegro Inhand, and Sharpa Inhand (HORA teacher).}
    \label{fig:app_appo_task_grid}
\end{figure}

\begin{figure}[H]
    \centering
    \includegraphics[width=0.95\textwidth]{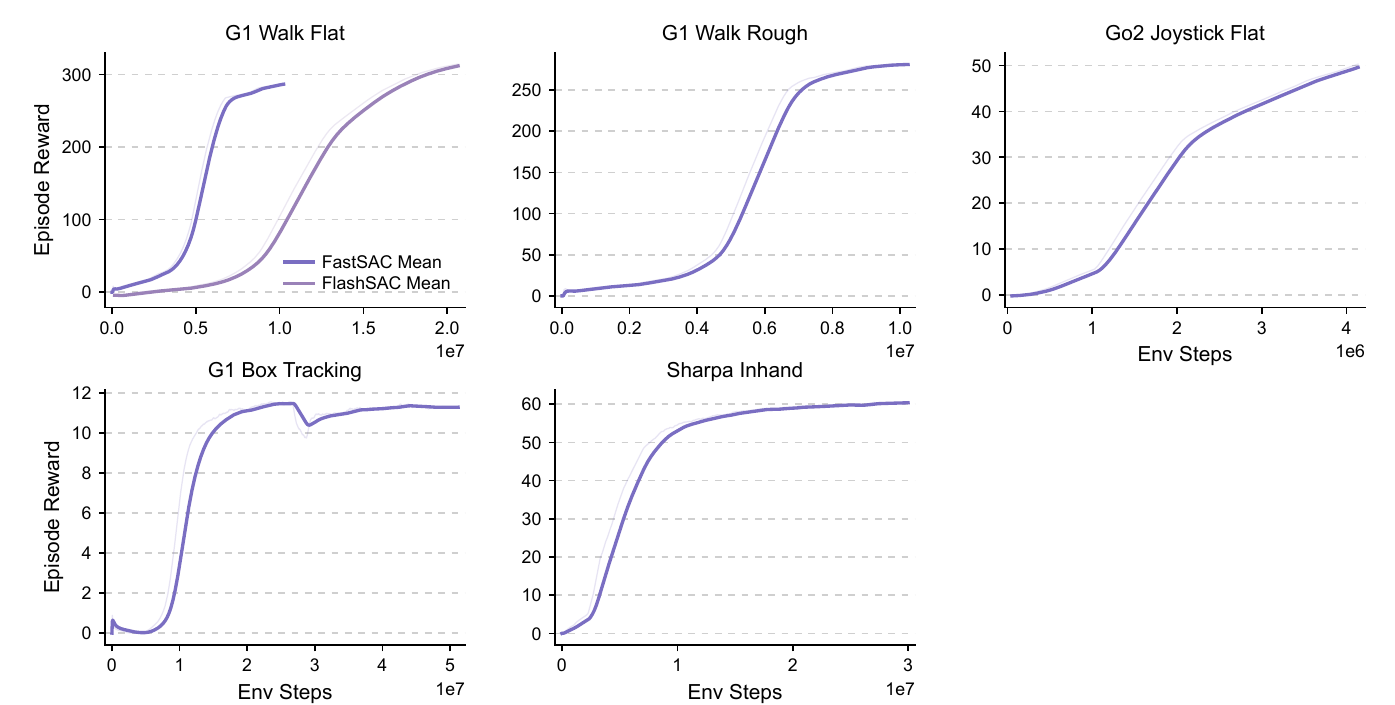}
    \caption{FastSAC and FlashSAC training curves for the five tasks with a replay configuration. G1 Walk Flat reports both FastSAC and FlashSAC; the remaining four tasks (G1 Walk Rough, Go2 Joystick Flat, G1 Box Tracking, Sharpa Inhand) report FastSAC only.}
    \label{fig:app_sac_task_grid}
\end{figure}

\subsection{Bidirectional Sim2Sim Cross-Backend Validation}
\label{app:sim2sim_cross_validation}

\paragraph{Objective.}
This subsection evaluates whether a policy trained against one simulation backend transfers to the other without retraining. We rollout each checkpoint on both MuJoCoUni and MotrixSim and compare its behaviour. Because each task uses backend-specific reward shaping at training time, the absolute reward values from different training backends are not directly comparable; what is meaningful is the change of each metric when the same policy is moved between backends, since this isolates the gap introduced by the simulator rather than by the policy.

\paragraph{Metrics.}
We report three quantities per (policy, evaluation-backend) pair:
\begin{itemize}
    \item \textbf{Mean episodic return:} the mean cumulative reward over 100 evaluation episodes, computed with the reward scale stored with the checkpoint at training time.
    \item \textbf{Success rate:} the fraction of the 100 episodes that finish without early termination.
    \item \textbf{MPJPE (m):} the mean per-joint position error against the reference trajectory, averaged over time and joints. MPJPE is only defined for motion-tracking tasks; locomotion rows report a dash.
\end{itemize}

\paragraph{Protocol.}
All numbers come from zero-shot rollouts of a single trained checkpoint per policy: no fine-tuning, no retraining, and no per-backend adaptation. For each task we evaluate two checkpoints---one trained on MuJoCoUni and one trained on MotrixSim---and run each checkpoint on both backends, yielding four rows per task. The native rows (train backend $=$ test backend) act as the reference; the cross rows (train backend $\ne$ test backend) measure the sim2sim gap. Each cell aggregates 100 episodes. Cross-backend evaluation uses the reward weights and normalization constants associated with the policy's training backend, ensuring that changes reflect simulator transfer rather than reward-definition changes.

\begin{table}[!htbp]
    \centering
    \small
    \caption{Bidirectional sim2sim cross-backend evaluation. For each task, the four rows correspond to: native MotrixSim (train$=$test$=$MotrixSim), forward transfer (MotrixSim$\to$MuJoCoUni), native MuJoCoUni (train$=$test$=$MuJoCoUni), and reverse transfer (MuJoCoUni$\to$MotrixSim). Mean return is comparable only within the four rows of a single task: reward scales are task- and training-backend-specific. A dash in the MPJPE column marks locomotion rows, where no reference trajectory exists.}
    \label{tab:app_sim2sim_cross}
    \resizebox{\textwidth}{!}{%
    \begin{tabular}{@{}llllcccc@{}}
        \toprule
        Test type & Task & Train backend & Test backend & Mean return & Success & MPJPE\,(m) & Episodes \\
        \midrule
        \multicolumn{8}{l}{\emph{G1 Walk Flat (SAC)}} \\
        Native      & G1 Walk Flat       & MotrixSim & MotrixSim & 408.38 & 1.00 & --- & 100 \\
        Forward     & G1 Walk Flat       & MotrixSim & MuJoCoUni & 405.46 & 1.00 & --- & 100 \\
        Native      & G1 Walk Flat       & MuJoCoUni & MuJoCoUni & 354.41 & 1.00 & --- & 100 \\
        Reverse     & G1 Walk Flat       & MuJoCoUni & MotrixSim & 354.00 & 1.00 & --- & 100 \\
        \midrule
        \multicolumn{8}{l}{\emph{G1 Motion Tracking, dance reference (SAC)}} \\
        Native      & G1 Motion Tracking & MotrixSim & MotrixSim & 45.26 & 1.00 & 0.0217 & 100 \\
        Forward     & G1 Motion Tracking & MotrixSim & MuJoCoUni & 45.17 & 1.00 & 0.0219 & 100 \\
        Native      & G1 Motion Tracking & MuJoCoUni & MuJoCoUni & 45.36 & 1.00 & 0.0197 & 100 \\
        Reverse     & G1 Motion Tracking & MuJoCoUni & MotrixSim & 45.34 & 1.00 & 0.0204 & 100 \\
        \midrule
        \multicolumn{8}{l}{\emph{G1 Shuttle-Run Tracking (PPO)}} \\
        Native      & G1 Shuttle-Run     & MotrixSim & MotrixSim & 45.80 & 1.00 & 0.0515 & 100 \\
        Forward     & G1 Shuttle-Run     & MotrixSim & MuJoCoUni & 42.28 & 0.92 & 0.0568 & 100 \\
        Native      & G1 Shuttle-Run     & MuJoCoUni & MuJoCoUni & 32.64 & 0.97 & 0.0519 & 100 \\
        Reverse     & G1 Shuttle-Run     & MuJoCoUni & MotrixSim & 31.95 & 0.91 & 0.0532 & 100 \\
        \midrule
        \multicolumn{8}{l}{\emph{G1 Wall Flip Tracking (PPO)}} \\
        Native      & G1 Wall Flip       & MotrixSim & MotrixSim & 84.46 & 1.00 & 0.0447 & 100 \\
        Forward     & G1 Wall Flip       & MotrixSim & MuJoCoUni & 79.46 & 1.00 & 0.0596 & 100 \\
        Native      & G1 Wall Flip       & MuJoCoUni & MuJoCoUni & 80.61 & 1.00 & 0.0431 & 100 \\
        Reverse     & G1 Wall Flip       & MuJoCoUni & MotrixSim & 77.44 & 1.00 & 0.0620 & 100 \\
        \bottomrule
    \end{tabular}}
\end{table}

Across the four tasks, success rate stays at 1.00 for both locomotion and the two acyclic tracking tasks (dance and wall flip); only the shuttle-run policies drop noticeably (0.97/1.00 native vs.\ 0.92/0.91 cross), and MPJPE remains within $0.0030$\,m of the native baseline for the dance clip, within $0.0053$\,m for the shuttle run, and within $0.0189$\,m for the wall flip. These margins are small relative to the per-joint reference scale and indicate that the policies generalize across the two backends without backend-specific adaptation.

\subsection{Task Specifications}
\label{app:training_curves_tasks}

This subsection lists the per-task observation space, action space, command and termination logic, domain randomization, and reward weights for every task evaluated in the main paper. Tasks are grouped by family: locomotion, motion tracking, manipulation-locomotion, and dexterous-hand in-hand manipulation. When MuJoCoUni and MotrixSim share a value it is reported once; backend-specific differences are called out explicitly.

\subsubsection{Locomotion}
\label{app:task_locomotion}

\paragraph{Go1 Joystick Flat.}
\texttt{Go1JoystickFlat} runs on the flat Go1 scene with simulation step $\Delta t_{\mathrm{sim}}=0.01$\,s, control step $\Delta t_{\mathrm{ctrl}}=0.02$\,s, maximum episode 20\,s, and initial base position $(0,0,0.34)$.

\noindent\textbf{Observation space.}
The actor observation is 49-dimensional:
\begin{equation}
    o_t = [\omega_t,\,-g_t,\,q_t-q_{\mathrm{default}},\,\dot q_t,\,a_{t-1},\,c_t,\,\phi_t],
\end{equation}
where $\omega_t\in\mathbb{R}^3$ is the body-frame gyro, $g_t\in\mathbb{R}^3$ is the up-vector sensor, $q_t-q_{\mathrm{default}}\in\mathbb{R}^{12}$ is the joint-position offset, $\dot q_t\in\mathbb{R}^{12}$ is joint velocity, $a_{t-1}\in\mathbb{R}^{12}$ is the previous action, $c_t\in\mathbb{R}^3$ is the velocity command, and $\phi_t\in\mathbb{R}^4$ is the four-leg gait phase. The critic observation appends local linear velocity, giving 52 dimensions.

\noindent\textbf{Action space.}
The action is a 12-dimensional joint-position offset. The environment maps policy output $a_t$ to actuator targets by $q^{\mathrm{cmd}}_t = q_{\mathrm{default}} + 0.25\,a_t$, using PD gains $K_p=35.0$, $K_d=0.5$.

\noindent\textbf{Commands and termination.}
The velocity-command range is $[(-0.6,-0.4,-0.8),(1.0,0.4,0.8)]$. An episode terminates early when the up-vector $z$ component satisfies $g^z_t \le 0.5$. Gait frequency is 2\,Hz.

\noindent\textbf{Domain randomization.}
Reset-time domain randomization is applied as listed in Table~\ref{tab:app_go1flat_backend_task_values}.

\begin{table}[!htbp]
    \centering
    \caption{Domain randomization for \texttt{go1\_joystick\_flat}.}
    \label{tab:app_go1flat_backend_task_values}
    \begin{tabular}{@{}lc@{}}
        \toprule
        Item & MuJoCoUni \\
        \midrule
        Velocity-command range & $[(-0.6,-0.4,-0.8),(1.0,0.4,0.8)]$ \\
        \texttt{randomize\_kp} & true (default) \\
        \texttt{randomize\_kd} & true (default) \\
        Kp/Kd multiplier range & $[0.9,1.1]$ \\
        \bottomrule
    \end{tabular}
\end{table}

\noindent\textbf{Reward design.}
The reward is $\Delta t_{\mathrm{ctrl}}\sum_i w_i r_i$. Table~\ref{tab:app_go1flat_reward} lists the active reward scales.

\begin{table}[!htbp]
    \centering
    \caption{Reward terms for \texttt{go1\_joystick\_flat}.}
    \label{tab:app_go1flat_reward}
    \begin{tabular}{@{}lc@{}}
        \toprule
        Term & MuJoCoUni \\
        \midrule
        Linear velocity tracking & 1.0 \\
        Yaw angular velocity tracking & 0.2 \\
        Vertical linear velocity & -5.0 \\
        Roll/pitch angular velocity & -0.1 \\
        Base height & -100.0 \\
        Action rate & -0.005 \\
        Joint deviation from default & -0.1 \\
        Contact phase agreement & 0.24 \\
        Swing-foot height & 4.0 \\
        \bottomrule
    \end{tabular}
\end{table}

The velocity-tracking terms use $\exp(-e^2/\sigma^2)$ with $\sigma=0.25$; the base-height penalty uses a target of $0.3$\,m; the swing-foot term uses $\exp(-e_z^2/0.01)$ gated by the swing phase ($\phi_i \ge 0.6$).

\paragraph{Go1 Joystick Rough.}
\texttt{Go1JoystickRough} adds procedurally generated terrain to the Go1 quadruped. The configuration is identical across the two backends. Simulation step $\Delta t_{\mathrm{sim}}=0.01$\,s, control step $\Delta t_{\mathrm{ctrl}}=0.02$\,s, maximum episode 20\,s.

\noindent\textbf{Observation space.}
The actor observation is 45-dimensional (policy group):
\begin{equation}
    o_t = [0.25\omega_t,\,-g_t,\,c_t,\,q_t-q_{\mathrm{default}},\,0.05\dot q_t,\,a_{t-1}],
\end{equation}
where gyro and joint velocity are pre-scaled. The critic observation is 48-dimensional (adds base linear velocity) plus a height-scan vector (default 187 points from an $11\times17$ grid around the robot base).

\noindent\textbf{Action space.}
The action is 12-dimensional with per-joint scaling: hip joints use \texttt{hip\_action\_scale}$=0.125$, non-hip joints use \texttt{non\_hip\_action\_scale}$=0.25$. PD gains $K_p=35.0$, $K_d=0.5$. Actions are clipped to $[-100, 100]$.

\noindent\textbf{Commands and termination.}
The velocity-command range is $[(-1,-1,-1),(1,1,1)]$ with heading command enabled and resampling every 10\,s. Terrain is procedurally generated on an $8\times8$\,m cell grid ($6\times6$ cells, border width 20\,m). Termination occurs when the robot moves more than 3\,m beyond its terrain cell boundary. No gravity-based termination is used.

\noindent\textbf{Domain randomization.}
Reset-time domain randomization is listed in Table~\ref{tab:app_go1rough_dr}.

\begin{table}[!htbp]
    \centering
    \caption{Domain randomization for \texttt{go1\_joystick\_rough}.}
    \label{tab:app_go1rough_dr}
    \begin{tabular}{@{}lcc@{}}
        \toprule
        Item & MuJoCoUni & MotrixSim \\
        \midrule
        \texttt{randomize\_base\_mass} & true & true \\
        Added mass range & $[-1.0, 3.0]$ & $[-1.0, 3.0]$ \\
        \texttt{random\_com} & true & true \\
        \texttt{randomize\_kp} & true & true \\
        Kp multiplier range & $[0.5, 2.0]$ & $[0.5, 2.0]$ \\
        \texttt{randomize\_kd} & true & true \\
        Kd multiplier range & $[0.5, 2.0]$ & $[0.5, 2.0]$ \\
        \texttt{push\_robots} & true & true \\
        Push interval (steps) & 625 & 625 \\
        Max push force & $[1.0, 1.0, 0.5]$ & $[1.0, 1.0, 0.5]$ \\
        \bottomrule
    \end{tabular}
\end{table}

\noindent\textbf{Reward design.}
Table~\ref{tab:app_go1rough_reward} lists the active reward scales.

\begin{table}[!htbp]
    \centering
    \caption{Reward terms for \texttt{go1\_joystick\_rough}.}
    \label{tab:app_go1rough_reward}
    \small
    \begin{tabular}{@{}lcc@{}}
        \toprule
        Term & MuJoCoUni & MotrixSim \\
        \midrule
        Linear velocity tracking & 3.0 & 3.0 \\
        Yaw angular velocity tracking & 1.5 & 1.5 \\
        Vertical linear velocity & -2.0 & -2.0 \\
        Roll/pitch angular velocity & -0.05 & -0.05 \\
        Joint torques L2 & $-2.5{\times}10^{-5}$ & $-2.5{\times}10^{-5}$ \\
        Joint acceleration L2 & $-2.5{\times}10^{-7}$ & $-2.5{\times}10^{-7}$ \\
        Joint position limits & -5.0 & -5.0 \\
        Joint power & $-2.0{\times}10^{-5}$ & $-2.0{\times}10^{-5}$ \\
        Stand still & -2.0 & -2.0 \\
        Hip position & -0.5 & -0.5 \\
        Joint position penalty & -1.0 & -1.0 \\
        Joint mirror & -0.05 & -0.05 \\
        Action rate & -0.01 & -0.01 \\
        Undesired contacts & -1.0 & -1.0 \\
        Contact forces & $-1.5{\times}10^{-4}$ & $-1.5{\times}10^{-4}$ \\
        Feet air time & 0.5 & 0.5 \\
        Feet air time variance & -1.0 & -1.0 \\
        Feet contact without cmd & 0.1 & 0.1 \\
        Feet slide & -0.1 & -0.1 \\
        Feet height body & -5.0 & -5.0 \\
        Feet gait & 0.5 & 0.5 \\
        Upward & 1.0 & 1.0 \\
        \bottomrule
    \end{tabular}
\end{table}

Tracking-style terms use $\sigma=0.25$ and the base-height penalty uses a target of $0.33$\,m on both backends.

\paragraph{Go2 Joystick Flat.}
\texttt{Go2JoystickFlat} runs on the flat Go2 scene with simulation step $\Delta t_{\mathrm{sim}}=0.01$\,s, control step $\Delta t_{\mathrm{ctrl}}=0.02$\,s, maximum episode 20\,s, and initial base position $(0,0,0.42)$.

\noindent\textbf{Observation space.}
The actor observation is 49-dimensional:
\begin{equation}
    o_t = [\omega_t,\,-g_t,\,q_t-q_{\mathrm{default}},\,\dot q_t,\,a_{t-1},\,c_t,\,\phi_t],
\end{equation}
where $\omega_t\in\mathbb{R}^3$ is the body-frame gyro reading, $g_t\in\mathbb{R}^3$ is the up-vector sensor value, $q_t-q_{\mathrm{default}}\in\mathbb{R}^{12}$ is the joint-position offset from the default pose, $\dot q_t\in\mathbb{R}^{12}$ is joint velocity, $a_{t-1}\in\mathbb{R}^{12}$ is the previous action, $c_t\in\mathbb{R}^3$ is the velocity command, and $\phi_t\in\mathbb{R}^4$ is the foot phase. The critic observation appends local linear velocity, giving a 52-dimensional privileged observation. Observation noise uses the default level.

\noindent\textbf{Action space.}
The action is a 12-dimensional joint-position command offset. The environment maps policy output $a_t$ to actuator targets by
\begin{equation}
    q^{\mathrm{cmd}}_t = q_{\mathrm{default}} + 0.25 a_t,
\end{equation}
using the shared Go2 PD gains $K_p=35.0$ and $K_d=0.5$.

\noindent\textbf{Commands and termination.}
The velocity-command range is $[(-0.6,-0.4,-0.8),(1.0,0.4,0.8)]$. An episode terminates early when the up-vector $z$ component satisfies $g^z_t \le 0.5$.

\noindent\textbf{Domain randomization.}
Reset-time domain randomization is applied as listed in Table~\ref{tab:app_go2_backend_task_values}.

\begin{table}[!htbp]
    \centering
    \caption{Domain randomization for \texttt{go2\_joystick\_flat}.}
    \label{tab:app_go2_backend_task_values}
    \begin{tabular}{@{}lc@{}}
        \toprule
        Item & MuJoCoUni \\
        \midrule
        Velocity-command range & $[(-0.6,-0.4,-0.8),(1.0,0.4,0.8)]$ \\
        \texttt{randomize\_kp} & true \\
        \texttt{randomize\_kd} & true \\
        Kp/Kd multiplier range & $[0.9,1.1]$ \\
        \bottomrule
    \end{tabular}
\end{table}

\noindent\textbf{Reward design.}
The reward is the control-step-scaled sum $\Delta t_{\mathrm{ctrl}}\sum_i w_i r_i$. Table~\ref{tab:app_go2_backend_reward} lists the active reward scales.

\begin{table}[!htbp]
    \centering
    \caption{Reward terms for \texttt{go2\_joystick\_flat}.}
    \label{tab:app_go2_backend_reward}
    \begin{tabular}{@{}lc@{}}
        \toprule
        Term & MuJoCoUni \\
        \midrule
        Linear velocity tracking & 1.0 \\
        Yaw angular velocity tracking & 0.2 \\
        Vertical linear velocity & -5.0 \\
        Roll/pitch angular velocity & -0.1 \\
        Base height & -100.0 \\
        Action rate & -0.005 \\
        Joint deviation from default pose & -0.1 \\
        Contact phase agreement & 0.24 \\
        Swing-foot height & 4.0 \\
        \bottomrule
    \end{tabular}
\end{table}

Tracking-style terms use $\sigma=0.25$ and the base-height penalty uses a target of $0.3$\,m. The swing-foot term rewards swing feet near 0.1\,m height; the contact term compares measured foot contact with the gait phase.

\paragraph{Go2 Joystick Rough.}
\texttt{Go2JoystickRough} shares the same architecture as Go1 Joystick Rough (procedural terrain, height scan, heading command) but uses the Go2 robot model. The configuration is identical across the two backends. Simulation step $\Delta t_{\mathrm{sim}}=0.01$\,s, control step $\Delta t_{\mathrm{ctrl}}=0.02$\,s, maximum episode 20\,s.

\noindent\textbf{Observation space.}
Same structure as Go1 Joystick Rough: actor 45-dimensional (pre-scaled gyro, gravity, command, joint offset, joint velocity, last action), critic 48-dimensional plus height-scan (187 points).

\noindent\textbf{Action space.}
12-dimensional with \texttt{hip\_action\_scale}$=0.125$, \texttt{non\_hip\_action\_scale}$=0.25$. PD gains $K_p=35.0$, $K_d=0.5$. Clip to $[-100, 100]$.

\noindent\textbf{Commands and termination.}
Velocity-command range $[(-1,-1,-1),(1,1,1)]$, heading command enabled, resampling every 10\,s. Terrain: $8\times8$\,m cells, $6\times6$ grid, border 20\,m. Termination: terrain out-of-bounds (3\,m buffer). No gravity-based termination.

\noindent\textbf{Domain randomization.}
Identical to Go1 Joystick Rough (Table~\ref{tab:app_go1rough_dr}): base mass $[-1,3]$\,kg, COM offset, Kp/Kd $[0.5,2.0]$, push robots every 625 steps with force $[1,1,0.5]$.

\noindent\textbf{Reward design.}
Same reward terms and weights as Go1 Joystick Rough (Table~\ref{tab:app_go1rough_reward}), with base-height target $0.33$\,m and tracking sigma $0.25$.

\paragraph{Go2W Joystick Flat.}
\texttt{Go2WJoystickFlat} is a wheeled-legged quadruped with 12 leg joints and 2 wheel joints. The configuration is identical across the two backends. Simulation step $\Delta t_{\mathrm{sim}}=0.01$\,s, control step $\Delta t_{\mathrm{ctrl}}=0.02$\,s, maximum episode 20\,s.

\noindent\textbf{Observation space.}
The actor observation is 53-dimensional:
\begin{equation}
    o_t = [\omega_t,\,-g_t,\,q^{leg}_t{-}q^{leg}_{\mathrm{def}},\,\dot q^{leg}_t,\,\dot q^{wheel}_t,\,a_{t-1},\,c_t],
\end{equation}
where the leg joint offset and velocity are 12-dimensional each, wheel velocity is 2-dimensional, and actions include both leg (12) and wheel (2) outputs. The critic observation is 72-dimensional (adds linear velocity, motor control targets, and wheel control targets).

\noindent\textbf{Action space.}
14-dimensional: 12 leg joints with \texttt{action\_scale}$=0.5$ and 2 wheel joints with \texttt{wheel\_action\_scale}$=10.0$. Leg PD gains $K_p=50.0$, $K_d=1.5$; wheel uses velocity control with $K_d^{wheel}=0.5$.

\noindent\textbf{Commands and termination.}
Velocity-command range $[(0,0,-1),(1,0,1)]$ (forward and yaw only). An episode terminates early when $g^z_t \le 0.5$.

\noindent\textbf{Domain randomization.}
Kp/Kd randomization is disabled. No other domain randomization is enabled in the flat variant.

\noindent\textbf{Reward design.}
Table~\ref{tab:app_go2wflat_reward} lists the active reward scales.

\begin{table}[!htbp]
    \centering
    \caption{Reward terms for \texttt{go2w\_joystick\_flat}.}
    \label{tab:app_go2wflat_reward}
    \begin{tabular}{@{}lcc@{}}
        \toprule
        Term & MuJoCoUni & MotrixSim \\
        \midrule
        Linear velocity tracking & 1.0 & 1.0 \\
        Yaw angular velocity tracking & 0.75 & 0.75 \\
        Vertical linear velocity & -5.0 & -5.0 \\
        Roll/pitch angular velocity & -0.1 & -0.1 \\
        Base height & -100.0 & -100.0 \\
        Orientation & -2.0 & -2.0 \\
        Action rate & -0.005 & -0.005 \\
        Joint deviation from default & -0.5 & -0.5 \\
        Torques & $-2.0{\times}10^{-4}$ & $-2.0{\times}10^{-4}$ \\
        Alive & 0.5 & 0.5 \\
        Upward & 1.0 & 1.0 \\
        \bottomrule
    \end{tabular}
\end{table}

Tracking-style terms use $\sigma=0.25$ and the base-height penalty uses a target of $0.4$\,m on both backends.

\paragraph{Go2W Joystick Rough.}
\texttt{Go2WJoystickRough} adds procedural terrain to the wheeled-legged Go2W. Simulation step $\Delta t_{\mathrm{sim}}=0.01$\,s, control step $\Delta t_{\mathrm{ctrl}}=0.02$\,s, maximum episode 20\,s.

\noindent\textbf{Observation space.}
The actor observation is 53-dimensional (pre-scaled gyro $0.25\omega$, gravity, command, leg joint offset, leg velocity $0.05\dot q$, last action including wheel). The critic observation is 56-dimensional (adds linear velocity) plus height-scan (187 points).

\noindent\textbf{Action space.}
14-dimensional: 12 leg joints with \texttt{action\_scale}$=0.5$ and 2 wheel joints with \texttt{wheel\_action\_scale}$=10.0$. Leg PD gains $K_p=35.0$, $K_d=0.5$; wheel $K_d^{wheel}=0.5$. Clip to $[-100, 100]$.

\noindent\textbf{Commands and termination.}
Velocity-command range $[(-1,-1,-1),(1,1,1)]$, heading command enabled, resampling every 10\,s. Terrain: $8\times8$\,m cells, $6\times6$ grid, border 20\,m. Termination: terrain out-of-bounds (3\,m buffer).

\noindent\textbf{Domain randomization.}
Table~\ref{tab:app_go2wrough_dr} lists the domain-randomization settings. Kp/Kd randomization is enabled under MotrixSim and disabled under MuJoCoUni.

\begin{table}[!htbp]
    \centering
    \caption{Domain randomization for \texttt{go2w\_joystick\_rough}.}
    \label{tab:app_go2wrough_dr}
    \begin{tabular}{@{}lcc@{}}
        \toprule
        Item & MuJoCoUni & MotrixSim \\
        \midrule
        \texttt{randomize\_base\_mass} & true & true \\
        Added mass range & $[-1.0, 3.0]$ & $[-1.0, 3.0]$ \\
        \texttt{random\_com} & true & true \\
        COM offset x & $[-0.05, 0.05]$ & $[-0.05, 0.05]$ \\
        \texttt{randomize\_kp} & false & true \\
        Kp multiplier range & $[0.5, 1.0]$ & $[0.5, 1.0]$ \\
        \texttt{randomize\_kd} & false & true \\
        Kd multiplier range & $[0.5, 1.0]$ & $[0.5, 1.0]$ \\
        \texttt{push\_robots} & true & true \\
        Push interval (steps) & 500 & 625 \\
        Max push force & $[0.5, 0.5, 0.0]$ & $[1.0, 1.0, 0.5]$ \\
        Push body & \texttt{base\_link} & \texttt{base\_link} \\
        \bottomrule
    \end{tabular}
\end{table}

\noindent\textbf{Reward design.}
Table~\ref{tab:app_go2wrough_reward} lists the active reward scales. MotrixSim adds an orientation penalty that MuJoCoUni does not use, and the two backends differ on the hip-position penalty weight.

\begin{table}[!htbp]
    \centering
    \caption{Reward terms for \texttt{go2w\_joystick\_rough}.}
    \label{tab:app_go2wrough_reward}
    \small
    \begin{tabular}{@{}lcc@{}}
        \toprule
        Term & MuJoCoUni & MotrixSim \\
        \midrule
        Linear velocity tracking & 3.0 & 3.0 \\
        Yaw angular velocity tracking & 1.5 & 1.5 \\
        Vertical linear velocity & -2.0 & -2.0 \\
        Roll/pitch angular velocity & -0.05 & -0.05 \\
        Orientation & / & -2.0 \\
        Joint torques L2 & $-2.5{\times}10^{-5}$ & $-2.5{\times}10^{-5}$ \\
        Joint acceleration L2 & $-2.5{\times}10^{-7}$ & $-2.5{\times}10^{-7}$ \\
        Wheel-joint acceleration L2 & $-2.5{\times}10^{-9}$ & $-2.5{\times}10^{-9}$ \\
        Joint position limits & -5.0 & -5.0 \\
        Joint power & $-2.0{\times}10^{-5}$ & $-2.0{\times}10^{-5}$ \\
        Action rate & -0.01 & -0.01 \\
        Stand still & -2.0 & -2.0 \\
        Hip position & -2.0 & -0.5 \\
        Joint position penalty & -1.0 & -1.0 \\
        Joint mirror & -0.05 & -0.05 \\
        Upward & 1.0 & 1.0 \\
        \bottomrule
    \end{tabular}
\end{table}

Tracking-style terms use $\sigma=0.25$ and the base-height penalty uses a target of $0.4$\,m on both backends.

\paragraph{G1 Walk Flat.}
\texttt{G1WalkFlat} is a 29-DOF humanoid locomotion task on the flat G1 scene. Simulation step $\Delta t_{\mathrm{sim}}=0.01$\,s, control step $\Delta t_{\mathrm{ctrl}}=0.02$\,s, maximum episode 20\,s, initial base position $(0,0,0.754)$.

\noindent\textbf{Observation space.}
The actor observation is 98-dimensional:
\begin{equation}
    o_t = [\omega_t,\,-g_t,\,q_t-q_{\mathrm{default}},\,\dot q_t,\,a_{t-1},\,c_t,\,\phi_t],
\end{equation}
where joint offset, joint velocity, and last action are 29-dimensional each, and $\phi_t\in\mathbb{R}^2$ is the bipedal gait phase (left, right). The critic observation is 101-dimensional (adds base linear velocity).

\noindent\textbf{Action space.}
29-dimensional joint-position offset. Action mapping $q^{\mathrm{cmd}}_t = q_{\mathrm{default}} + s\,a_t$ with backend-dependent scale: MuJoCoUni uses $s=0.25$, MotrixSim uses $s=0.5$. PD gains $K_p=50.0$, $K_d=1.0$ (from G1 base config).

\noindent\textbf{Commands and termination.}
Under MuJoCoUni the velocity-command range follows the task default; under MotrixSim it is fixed to $[(0.4,0,0),(0.7,0,0)]$ (forward walking only) with the gait phase initialized at the configured offset and the reset base-velocity limited to $0.05$\,m/s. Termination occurs when body tilt exceeds the configured maximum or the base height drops below the configured minimum: MuJoCoUni uses $25^\circ$ and $0.55$\,m, MotrixSim uses $35^\circ$ and $0.5$\,m.

\noindent\textbf{Domain randomization.}
The velocity curriculum is disabled. Under MotrixSim Kp/Kd randomization is additionally disabled. Observation noise is configured identically on both backends: noise level $1.0$, joint-angle scale $0.01$, joint-velocity scale $1.5$, gyro scale $0.2$.

\noindent\textbf{Reward design.}
Table~\ref{tab:app_g1walkflat_reward} lists the active reward scales. MotrixSim introduces several gait-shaping terms (feet phase contrast, feet phase contact, double-stance penalty, under-speed penalty, upper-body pose) that are not used under MuJoCoUni.

\begin{table}[!htbp]
    \centering
    \caption{Reward terms for \texttt{g1\_walk\_flat}.}
    \label{tab:app_g1walkflat_reward}
    \small
    \begin{tabular}{@{}lcc@{}}
        \toprule
        Term & MuJoCoUni & MotrixSim \\
        \midrule
        Linear velocity tracking & 2.0 & 2.0 \\
        Yaw angular velocity tracking & 0.2 & 0.25 \\
        Feet phase & 1.0 & 1.2 \\
        Feet phase contrast & / & 1.5 \\
        Feet phase contact & / & 1.0 \\
        Feet double stance & / & -1.0 \\
        Under speed & / & -0.2 \\
        Upper body pose & / & -0.05 \\
        Vertical linear velocity & -1.0 & -1.0 \\
        Roll/pitch angular velocity & -0.25 & -0.2 \\
        Base height & -500.0 & -120.0 \\
        Orientation & -5.0 & -2.5 \\
        Action rate & -0.01 & -0.005 \\
        Pose (weighted) & -0.1 & -0.05 \\
        \bottomrule
    \end{tabular}
\end{table}

Shaping parameters used by the table above: velocity-tracking $\sigma=0.25$, gait frequency $1.5$\,Hz, feet-phase swing height $0.09$\,m, feet-phase tracking $\sigma=0.008$, base-height target $0.754$\,m (MuJoCoUni) / $0.765$\,m (MotrixSim). The 29-entry pose-weight vector is identical on both backends. Under MotrixSim, the gait reward is gated by a minimum forward speed of $0.05$\,m/s.

\paragraph{G1 Walk Rough.}
\texttt{G1WalkRough} is the rough-terrain variant trained with SAC on both backends. The environment shares the same 29-DOF humanoid structure as G1 Walk Flat with terrain-aware reset behaviour.

\noindent\textbf{Observation space.}
Same structure as G1 Walk Flat: actor 98-dimensional, critic 101-dimensional. Refer to the G1 Walk Flat paragraph for the layout.

\noindent\textbf{Action space.}
29-dimensional joint-position offset with action scale $s=1.0$ (raised from the task default $0.25$). PD gains $K_p=50.0$, $K_d=1.0$.

\noindent\textbf{Commands and termination.}
The gait phase is initialized at the configured offset and the reset base-velocity is limited to $0.5$\,m/s. A base-velocity curriculum is enabled with initial scale $0.5$, maximum scale $1.0$, level-down threshold $150$, level-up threshold $750$, and degree $0.001$. Under MotrixSim, Kp/Kd randomization is disabled and the simulation step is set to $0.01$\,s. Termination uses a maximum tilt of $65^\circ$ and a minimum base height of $0.3$\,m.

\noindent\textbf{Domain randomization.}
Under MuJoCoUni, observation noise uses level $1.0$ with joint-angle scale $0.01$ and joint-velocity scale $0.1$ (other channels zero). Under MotrixSim, the default noise level is used. MuJoCoUni enables policy symmetry at the algorithm level; MotrixSim does not. Mass, COM, and push randomization are not enabled on either backend.

\noindent\textbf{Reward design.}
Table~\ref{tab:app_g1walkrough_reward} lists the active reward scales. MotrixSim uses a tighter feet-phase tracking sigma than MuJoCoUni.

\begin{table}[!htbp]
    \centering
    \caption{Reward terms for \texttt{g1\_walk\_rough}.}
    \label{tab:app_g1walkrough_reward}
    \begin{tabular}{@{}lcc@{}}
        \toprule
        Term & MuJoCoUni & MotrixSim \\
        \midrule
        Linear velocity tracking & 2.0 & 2.2 \\
        Yaw angular velocity tracking & 1.5 & 1.8 \\
        Penalty ang vel xy & -1.0 & -1.2 \\
        Penalty orientation & -10.0 & -12.0 \\
        Penalty action rate & -4.0 & -2.5 \\
        Pose (weighted) & -0.5 & -0.6 \\
        Penalty feet orientation & -20.0 & -5.0 \\
        Feet phase & 5.0 & 6.0 \\
        Alive & 10.0 & 12.0 \\
        \bottomrule
    \end{tabular}
\end{table}

Shaping parameters used by the table above: velocity-tracking $\sigma=0.25$, gait frequency $1.5$\,Hz, feet-phase swing height $0.09$\,m, feet-phase tracking $\sigma=0.04$ (MuJoCoUni) / $0.008$ (MotrixSim), close-feet threshold $0.15$\,m, base-height target $0.754$\,m. Termination thresholds (maximum tilt $65^\circ$, minimum base height $0.3$\,m) are repeated here from the Commands and termination paragraph for reference.

\subsubsection{Motion Tracking}
\label{app:task_motion_tracking}

The motion-tracking family imitates a reference motion clip on the 29-DOF G1 humanoid. All five tasks (\texttt{g1\_motion\_tracking}, \texttt{g1\_climb\_tracking}, \texttt{g1\_flip\_tracking}, \texttt{g1\_wall\_flip\_tracking}, \texttt{g1\_box\_tracking}) share the same observation/action layout and reward-term library; they differ in reference motion clip, scene, sampling mode, and termination thresholds. The shared structure is described once under G1 Motion Tracking; per-variant deltas follow.

\paragraph{G1 Motion Tracking.}
\texttt{G1MotionTracking} runs on the flat G1 scene with a dance reference clip. The configuration is identical across the two backends. Simulation step from the G1 base config, control step $\Delta t_{\mathrm{ctrl}}=0.02$\,s, maximum episode 10\,s.

\noindent\textbf{Observation space.}
The actor observation is 176-dimensional:
\begin{equation}
    o^{actor}_t = [m^{joint}_t,\,p^{ref}_{b,t},\,R^{ref}_{b,t},\,v^{base}_t,\,\omega_t,\,q_t-q_{\mathrm{default}},\,\dot q_t,\,a_{t-1}],
\end{equation}
where $m^{joint}_t\in\mathbb{R}^{58}$ is the reference joint position and velocity (29+29), $p^{ref}_{b,t}\in\mathbb{R}^3$ is the reference anchor position in body frame, $R^{ref}_{b,t}\in\mathbb{R}^6$ is the reference anchor orientation (6D rotation representation), and the remaining channels mirror the locomotion observation layout for 29 joints. The critic observation appends per-body privileged transforms for all 14 tracked bodies (3D position + 6D orientation each, $14\times9=126$ extra dims), giving a 302-dimensional critic.

The 14 tracked bodies are: \texttt{pelvis}, left/right \{\texttt{hip\_roll\_link}, \texttt{knee\_link}, \texttt{ankle\_roll\_link}\}, \texttt{torso\_link} (anchor body), left/right \{\texttt{shoulder\_roll\_link}, \texttt{elbow\_link}, \texttt{wrist\_yaw\_link}\}.

\noindent\textbf{Action space.}
29-dimensional joint-position offset with a per-joint 29-element action scale (not a single scalar). PD gains from the G1 base config ($K_p=50.0$, $K_d=1.0$).

\noindent\textbf{Commands and termination.}
There is no joystick command channel; the reference motion plays the role of command. Termination occurs when any of the following holds: anchor-position $z$-error exceeds $0.25$\,m, end-effector $z$-error exceeds $0.25$\,m, or a non-EE body falls below $0.05$\,m when undesired-contact termination is enabled. Anchor-orientation termination is disabled.

\noindent\textbf{Reference-clip sampling.}
The per-environment start frame is chosen at reset by one of four modes: always frame zero, random clip start, uniform over all frames, or failure-weighted adaptive bin sampling. G1 Motion Tracking uses the adaptive mode.

\noindent\textbf{Domain randomization.}
Under MuJoCoUni, observation noise uses the environment defaults. Under MotrixSim, noise level $1.0$ is enabled with joint-angle scale $0.01$, joint-velocity scale $1.5$, and gyro scale $0.2$. Base-mass, COM, gravity, push, and Kp/Kd randomization are not enabled.

\noindent\textbf{Reward design.}
Each motion-tracking term has the form $\exp(-e^2/\sigma^2)$ where $e$ is the reference-tracking error in the corresponding channel; non-tracking penalties use squared / L2 forms identical to the locomotion library. Table~\ref{tab:app_g1mt_reward} lists the active scales.

\begin{table}[!htbp]
    \centering
    \caption{Reward terms for \texttt{g1\_motion\_tracking}.}
    \label{tab:app_g1mt_reward}
    \begin{tabular}{@{}lcc@{}}
        \toprule
        Term & MuJoCoUni & MotrixSim \\
        \midrule
        motion\_global\_root\_pos & 0.5 & 1.0 \\
        motion\_global\_root\_ori & 0.5 & 0.5 \\
        motion\_body\_pos & 1.0 & 1.0 \\
        motion\_body\_ori & 1.0 & 1.0 \\
        motion\_body\_lin\_vel & 1.0 & 1.0 \\
        motion\_body\_ang\_vel & 1.0 & 1.0 \\
        action\_rate\_l2 & -0.1 & -0.05 \\
        joint\_limit & -10.0 & -10.0 \\
        undesired\_contacts & / & -0.1 \\
        \bottomrule
    \end{tabular}
\end{table}

Shaping parameters (per-channel tracking $\sigma$ used inside the $\exp(-e^2/\sigma^2)$ form) are identical on the two backends: $\sigma_{\mathrm{root\_pos}}=0.3$, $\sigma_{\mathrm{root\_ori}}=0.4$, $\sigma_{\mathrm{body\_pos}}=0.3$, $\sigma_{\mathrm{body\_ori}}=0.4$, $\sigma_{\mathrm{body\_lin\_vel}}=1.0$, $\sigma_{\mathrm{body\_ang\_vel}}=3.14$, $\sigma_{\mathrm{joint\_pos}}=0.2$, $\sigma_{\mathrm{joint\_vel}}=1.0$. The joint-position and joint-velocity tracking terms are not used in this configuration.

\paragraph{G1 Climb Tracking.}
The climb variant uses a scene with a 20-rung wall and a matched climbing reference clip. Maximum episode is $15$\,s, sampling is adaptive, simulation step is $0.005$\,s, undesired-contact termination is enabled, and anchor/end-effector $z$-error thresholds are both $0.3$\,m. The episode is not truncated when the clip ends.

The per-joint action scale is roughly $0.55$ for hip and ankle joints, $0.35$ for the knee, $0.44$ for waist and shoulder joints, and $0.07$ for wrist joints. Observation, action, and termination structure match G1 Motion Tracking.

\noindent\textbf{Reward design.}
Reward scales are identical across the two backends (Table~\ref{tab:app_g1ct_reward}). Compared to G1 Motion Tracking, the climb variant additionally weights end-effector vertical tracking, joint-position tracking, and joint-velocity tracking to encourage limb coordination with the reference clip.

\begin{table}[!htbp]
    \centering
    \caption{Reward terms for \texttt{g1\_climb\_tracking} (mj/mx identical).}
    \label{tab:app_g1ct_reward}
    \begin{tabular}{@{}lc@{}}
        \toprule
        Term & Weight \\
        \midrule
        motion\_global\_root\_pos & 0.5 \\
        motion\_global\_root\_ori & 0.5 \\
        motion\_body\_pos & 2.0 \\
        motion\_body\_ori & 1.5 \\
        motion\_body\_lin\_vel & 1.0 \\
        motion\_body\_ang\_vel & 1.0 \\
        motion\_ee\_body\_pos\_z & 2.0 \\
        motion\_joint\_pos & 0.5 \\
        motion\_joint\_vel & 0.25 \\
        action\_rate\_l2 & -0.005 \\
        joint\_limit & -10.0 \\
        undesired\_contacts & -0.1 \\
        \bottomrule
    \end{tabular}
\end{table}

The sigma values match the G1 Motion Tracking defaults (Table~\ref{tab:app_g1mt_reward}).

\paragraph{G1 Flip Tracking.}
The flip variant uses the flat G1 scene with a 360-degree flip reference clip. Sampling always starts from frame zero, the episode is not truncated when the clip ends, and the simulation step is $0.005$\,s.

Under MuJoCoUni, the anchor and end-effector $z$-error thresholds are both $0.5$\,m, undesired-contact termination is enabled, and the per-joint action scale matches G1 Climb Tracking. Under MotrixSim, the corresponding thresholds and action scale use the baseline environment settings.

\begin{table}[!htbp]
    \centering
    \caption{Reward terms for \texttt{g1\_flip\_tracking}.}
    \label{tab:app_g1ft_reward}
    \begin{tabular}{@{}lcc@{}}
        \toprule
        Term & MuJoCoUni & MotrixSim \\
        \midrule
        motion\_global\_root\_pos & 0.5 & 1.0 \\
        motion\_global\_root\_ori & 0.5 & 0.5 \\
        motion\_body\_pos & 2.0 & 1.0 \\
        motion\_body\_ori & 1.5 & 1.0 \\
        motion\_body\_lin\_vel & 1.0 & 1.0 \\
        motion\_body\_ang\_vel & 1.0 & 1.0 \\
        motion\_ee\_body\_pos\_z & 2.0 & / \\
        action\_rate\_l2 & -0.005 & -0.05 \\
        joint\_limit & -10.0 & -10.0 \\
        undesired\_contacts & -0.1 & / \\
        \bottomrule
    \end{tabular}
\end{table}

\paragraph{G1 Wall Flip Tracking.}
The wall-flip variant uses a flat scene with a wall and a wall-flip reference clip. Sampling always starts from frame zero, the episode is not truncated when the clip ends, the simulation step is $0.005$\,s, anchor and end-effector $z$-error thresholds are both $0.5$\,m, undesired-contact termination is enabled, and the per-joint action scale matches G1 Climb Tracking. Under MotrixSim, the solver runs three substep iterations per control step.

Reward scales are identical across the two backends and match the climb-tracking weights (Table~\ref{tab:app_g1ct_reward}); only the reference clip and the wall-scene termination geometry change.

\paragraph{G1 Box Tracking.}
The box variant uses a flat scene with a large box and a box-manipulation reference clip. It extends G1 Motion Tracking with explicit object-state tracking: the critic observation appends 12 extra dimensions (object position, object 6D orientation, object linear velocity, all in body frame) for a 314-dimensional critic. The actor observation remains 176-dimensional. Under MuJoCoUni, the simulation step is $0.005$\,s; under MotrixSim, the base step is used.

Under MotrixSim, empirical normalization is enabled, an asymmetric critic observation group is declared, and observation noise uses level $1.0$ with joint-angle scale $0.01$, joint-velocity scale $1.5$, and gyro scale $0.2$.

\begin{table}[!htbp]
    \centering
    \caption{Reward terms for \texttt{g1\_box\_tracking}.}
    \label{tab:app_g1bt_reward}
    \small
    \begin{tabular}{@{}lcc@{}}
        \toprule
        Term & MuJoCoUni & MotrixSim \\
        \midrule
        motion\_global\_root\_pos & 0.5 & 1.0 \\
        motion\_global\_root\_ori & 0.5 & 0.5 \\
        motion\_body\_pos & 1.0 & 1.0 \\
        motion\_body\_ori & 1.0 & 1.5 \\
        motion\_body\_lin\_vel & 1.0 & 1.0 \\
        motion\_body\_ang\_vel & 1.0 & 1.5 \\
        action\_rate\_l2 & -0.1 & -0.1 \\
        joint\_limit & -10.0 & -10.0 \\
        undesired\_contacts & -0.1 & -0.1 \\
        object\_global\_ref\_position\_error\_exp & 2.0 & 4.0 \\
        object\_global\_ref\_orientation\_error\_exp & 2.0 & 3.0 \\
        \bottomrule
    \end{tabular}
\end{table}

Body-tracking sigmas inherit the G1 Motion Tracking defaults; the object-tracking sigmas used inside $\exp(-e^2/\sigma^2)$ differ between backends: $\sigma_{\mathrm{object\_pos}}=0.2$ (MuJoCoUni) / $0.12$ (MotrixSim), $\sigma_{\mathrm{object\_ori}}=0.3$ (MuJoCoUni) / $0.2$ (MotrixSim).

\subsubsection{Manipulation-Locomotion}
\label{app:task_manipulation_locomotion}

This subsection covers tasks where locomotion is coupled with an upper-body manipulation or posture objective. Two tasks are included: Go2 Hand Stand (rear-leg balance) and Go2 Arm Manip Loco (locomotion with a 6-DOF arm tracking an end-effector goal).

\paragraph{Go2 Hand Stand.}
\texttt{Go2HandStand} rewards the robot for inverting onto its front legs while maintaining a target torso height. Under MuJoCoUni the simulation step is $0.005$\,s; under MotrixSim it is $0.01$\,s. Control step $\Delta t_{\mathrm{ctrl}}=0.02$\,s, maximum episode 20\,s.

\noindent\textbf{Observation space.}
The actor observation is 42-dimensional:
\begin{equation}
    o_t = [\omega_t,\,-g_t,\,q_t-q_{\mathrm{default}},\,\dot q_t,\,a_{t-1}],
\end{equation}
where joint offset, joint velocity, and last action are 12-dimensional each. No velocity command channel; the task is a fixed posture-tracking objective. The critic observation is 46-dimensional (adds base linear velocity 3 and torso height 1).

\noindent\textbf{Action space.}
12-dimensional joint-position offset with default \texttt{action\_scale}. PD gains $K_p=35.0$, $K_d=0.5$.

\noindent\textbf{Commands and termination.}
The target pose is inverted handstand: target torso height $z_{des}=0.55$\,m, desired gravity $g_{des}=(-1,0,0)$ (body $x$-axis aligned with world gravity). Termination occurs when the up-vector $z$-component satisfies $g^z_t \le -0.25$ (robot fully inverted past the target) or when undesired contacts on front legs/hips/thighs occur. A rear-leg gait at 2\,Hz (RL phase 0, RR phase 0.5) provides a phase signal for the gait-aware reward terms.

\noindent\textbf{Domain randomization.}
Under MotrixSim, Kp/Kd randomization is disabled. No additional domain randomization is enabled on top of the environment defaults.

\noindent\textbf{Reward design.}
Table~\ref{tab:app_go2hs_reward} lists the active reward scales. The two backends differ only in the front-leg contact weight.

\begin{table}[!htbp]
    \centering
    \caption{Reward terms for \texttt{go2\_handstand}.}
    \label{tab:app_go2hs_reward}
    \begin{tabular}{@{}lcc@{}}
        \toprule
        Term & MuJoCoUni & MotrixSim \\
        \midrule
        Contact (front-leg) & -1.0 & -0.5 \\
        Height & 1.0 & 1.0 \\
        Orientation (alignment to target gravity) & 1.0 & 1.0 \\
        Pose (deviation from default) & -0.3 & -0.3 \\
        Penalty contact (penalty bodies) & -0.2 & -0.2 \\
        Action rate & -0.01 & -0.01 \\
        Target pose (\texttt{tar}) & 0.3 & 0.3 \\
        Feet air time (rear legs) & 1.0 & 1.0 \\
        World $z$-velocity penalty & -1.0 & -1.0 \\
        \bottomrule
    \end{tabular}
\end{table}

Shaping parameters: velocity-tracking $\sigma=0.25$ and base-height target $0.3$\,m on both backends. The \texttt{height} term uses $\exp(-|z_{des}-h|/0.1)$, the \texttt{orientation} term uses $[0.5\cos\angle(g,g_{des})+0.5]^2$, and the \texttt{tar} reward is gated by $h \ge 0.8\,z_{des}$.

\paragraph{Go2 Arm Manip Loco.}
\texttt{Go2ArmManipLoco} is available only on the MuJoCoUni backend. Simulation step $\Delta t_{\mathrm{sim}}=0.01$\,s, control step $\Delta t_{\mathrm{ctrl}}=0.02$\,s, maximum episode 20\,s.

\noindent\textbf{Observation space.}
The per-step observation is 79-dimensional:
\begin{equation}
    o_t = [v^{base}_t,\,\omega_t,\,-g_t,\,c_t,\,\phi_t,\,q_t-q_{\mathrm{default}},\,\dot q_t,\,p^{ee}_t,\,p^{goal}_t,\,e^{ee}_t,\,a_{t-1}],
\end{equation}
where $\phi_t\in\mathbb{R}^4$ is the four-foot gait phase, joint offset/velocity are 18-dimensional each (12 leg + 6 arm), $p^{ee}_t,\,p^{goal}_t,\,e^{ee}_t\in\mathbb{R}^3$ are end-effector position, goal, and error in body frame, and the action history is 18-dimensional. The actor observation drops base linear velocity (to avoid bypassing the on-board estimator) and uses a per-step history of $H_a$ frames; the critic observation keeps linear velocity and uses $H_c$ frames. Default history length is $H_a=H_c=1$.

\noindent\textbf{Action space.}
18-dimensional: 12 leg-joint offsets with action scale $0.25$ (hip-joint scale $0.125$) and 6 arm-joint offsets with arm action scale zero. Leg PD gains $K_p=35.0$, $K_d=0.5$. With the arm scale set to zero, the policy controls only the legs; the arm follows the IK-derived target from the end-effector goal.

\noindent\textbf{End-effector goal sampling.}
The end-effector goal is sampled in spherical coordinates around the body: radius $\in[0.3,0.6]$\,m, azimuth $\in[-1.26,1.05]$\,rad, polar angle $\in[-2.36,2.36]$\,rad. Trajectory time $\in[1.0,3.0]$\,s, hold time $\in[0.5,2.0]$\,s. Collision bounds: upper $[0.3,0.15,-0.115]$, lower $[-0.2,-0.15,-0.515]$, underground limit $z=-0.57$. The IK uses damping $0.05$, gain $1.0$, $\Delta q$-clip $0.2$, with target-orientation tracking.

\noindent\textbf{Commands and termination.}
Velocity-command range $[(-0.6,-0.4,-0.8),(1.0,0.4,0.8)]$, zero-command probability $0.15$ (for stable standing), command resampling every $4.0$\,s. The velocity curriculum is disabled. Termination: $g^z_t \le 0.5$.

\noindent\textbf{Domain randomization.}
The following terms are enabled: body-mass multiplier $[0.9, 1.1]$, random COM offset $x\in[-0.03,0.03]$, ground-friction multiplier $[0.8,1.2]$, DOF-armature multiplier $[0.8,1.2]$, base pushes every 500 steps with maximum force $[1.2,1.2,0.6]$, and Kp/Kd multipliers $[0.9,1.1]$. Base-mass and gravity randomization are not enabled.

\noindent\textbf{Reward design.}
Table~\ref{tab:app_go2arml_reward} lists the active reward scales.

\begin{table}[!htbp]
    \centering
    \caption{Reward terms for \texttt{go2\_arm\_manip\_loco}.}
    \label{tab:app_go2arml_reward}
    \begin{tabular}{@{}lc@{}}
        \toprule
        Term & MuJoCoUni \\
        \midrule
        Linear velocity tracking & 2.0 \\
        Yaw angular velocity tracking & 0.5 \\
        Vertical linear velocity & -5.0 \\
        Roll/pitch angular velocity & -0.1 \\
        Roll & -5.0 \\
        Base height & -100.0 \\
        Leg pose & -0.1 \\
        Action rate & -0.005 \\
        Stand still & -0.5 \\
        Contact phase agreement & 0.24 \\
        Swing-foot height & 4.0 \\
        Foot drag & -0.1 \\
        Object distance (to EE goal) & 2.0 \\
        Object distance L2 & -0.5 \\
        Arm collision & -1.0 \\
        \bottomrule
    \end{tabular}
\end{table}

Shaping parameters: velocity-tracking $\sigma=0.25$, base-height target $0.3$\,m, object-distance kernel $\sigma=0.1$.

\subsubsection{Dexterous-Hand and In-Hand Manipulation}
\label{app:task_dexterous_hand}

This subsection covers in-hand manipulation tasks where a multi-finger hand rotates a free object about a specified axis. Two tasks are included: Allegro Inhand Rotation (16-DOF hand, ball) and Sharpa Inhand Rotation (22-DOF hand with tactile sensing).

\paragraph{Allegro Inhand Rotation.}
\texttt{AllegroInhandRotation} rotates a free ball about a fixed world-axis using the 16-DOF Allegro hand. The configuration is identical across the two backends. Simulation step $\Delta t_{\mathrm{sim}}=0.005$\,s, control step $\Delta t_{\mathrm{ctrl}}=0.05$\,s (10 simulator steps per control step), maximum episode 20\,s.

\noindent\textbf{Observation space.}
The observation is 105-dimensional, organized as a lag-history of 3 steps of a 35-dimensional per-step frame:
\begin{equation}
    f_t = [\widetilde q^{hand}_t,\,q^{target}_t,\,p^{ball}_t],
\end{equation}
where $\widetilde q^{hand}_t\in\mathbb{R}^{16}$ is the normalized hand joint position (mapped from joint limits to $[-2,2]$), $q^{target}_t\in\mathbb{R}^{16}$ is the current incremental joint target, and $p^{ball}_t\in\mathbb{R}^3$ is the ball position. Actor and critic share a single observation group; the critic has no privileged channel.

\noindent\textbf{Action space.}
16-dimensional in $[-1,1]$. The environment maps actions to actuator targets incrementally: $q^{target}_t = q^{target}_{t-1} + s\,\mathrm{clip}(a_t)$ with $s = 1/24 \approx 0.0417$, then clipped to the actuator-range limits. PD gains $K_p=1.0$, $K_d=0.1$. Torque is clipped to $[-0.5, 0.5]$.

\noindent\textbf{Commands and termination.}
The rotation axis is the world $z$-axis, $\hat n=(0,0,1)$. The episode terminates when the ball height drops below $0.125$\,m.

\noindent\textbf{Domain randomization.}
All online domain randomization is disabled (base-mass, COM, gravity, push, joint noise, ball-velocity noise, ball-$z$ offset). Reset-time grasp variation is the only source of initialization diversity.

\noindent\textbf{Reward design.}
Reward scales are identical across the two backends (Table~\ref{tab:app_allegro_reward}).

\begin{table}[!htbp]
    \centering
    \caption{Reward terms for \texttt{allegro\_inhand} (mj/mx identical).}
    \label{tab:app_allegro_reward}
    \begin{tabular}{@{}lc@{}}
        \toprule
        Term & Weight \\
        \midrule
        rotate (\texttt{clip}$(\boldsymbol\omega^{ball}\cdot\hat n,-0.5,0.5)$) & 1.25 \\
        obj\_linvel ($\sum_i |v^{ball}_i|$) & -0.3 \\
        pose\_diff ($\sum_j(q_j-q_j^{init})^2$) & -0.3 \\
        torque ($\sum_j \tau_j^2$) & -0.1 \\
        work ($(\sum_j \tau_j \dot q_j)^2$) & -2.0 \\
        \bottomrule
    \end{tabular}
\end{table}

Shaping parameters: angular-velocity clip range $[-0.5, 0.5]$\,rad/s inside the rotate term, and ball-height reset threshold $0.125$\,m used by the termination check. The reward is $\Delta t_{\mathrm{ctrl}}\sum_i w_i r_i$.

\paragraph{Sharpa Inhand Rotation.}
\texttt{SharpaInhandRotation} rotates a cylinder using the 22-DOF Sharpa hand with tactile sensing. The numbers reported here correspond to the MuJoCoUni HORA teacher configuration, which is shared by the APPO, SAC, and PPO HORA comparisons. Simulation step $1/240$\,s, control step $\Delta t_{\mathrm{ctrl}}=12/240=0.05$\,s, maximum episode 20\,s.

\noindent\textbf{Observation space.}
The per-step policy frame is 49-dimensional:
\begin{equation}
    f_t = [\widetilde q^{hand}_t,\,q^{target}_t,\,F^{tactile}_t],
\end{equation}
with $\widetilde q^{hand}_t\in\mathbb{R}^{22}$, $q^{target}_t\in\mathbb{R}^{22}$, and tactile forces $F^{tactile}_t\in\mathbb{R}^5$ (one per fingertip). The frame is stacked over a 3-step lag history, giving a 147-dimensional policy observation. The privileged tail is 9-dimensional: object position delta (3), friction scale (1), mass (1), COM offset (3), and object scale (1). In flattened mode the single observation group is $147+9=156$-dimensional. In separated mode the actor receives the 147-dimensional policy observation, while the critic receives the 156-dimensional concatenation.

\noindent\textbf{Action space.}
22-dimensional in $[-1,1]$. Incremental position control: $q^{target}_t = q^{target}_{t-1} + s\,\mathrm{clip}(a_t)$, $s=1/24$, with joint limits scaled by $0.9$. PD gains are set per actuator and randomized at reset within $[0.5, 2.0]$ around their nominal values.

\noindent\textbf{Commands and termination.}
Rotation axis $\hat n = (0,0,1)$. Termination uses object world-$z$ height bounds $[p^{obj}_z - 0.5\Delta h, p^{obj}_z + 0.5\Delta h]$ with $\Delta h = 0.04$\,m centered on the reset object position; the fallback bounds are $[0.59906, 0.63906]$\,m. The rotation rollout does not use angular-violation termination; angular deviation is used only during offline grasp-state filtering.

\noindent\textbf{Domain randomization.}
A rich randomization stack is enabled on both backends (Table~\ref{tab:app_sharpa_dr}). The reported Sharpa teacher runs use eight cylinder scales $\{0.8\ldots1.5\}$, excluding 1.6 to align with the external baseline setup. The active gravity setting is fixed-magnitude direction randomization; full-vector gravity randomization is disabled.

\begin{table}[!htbp]
    \centering
    \caption{Domain randomization for \texttt{sharpa\_inhand}.}
    \label{tab:app_sharpa_dr}
    \begin{tabular}{@{}lcc@{}}
        \toprule
        Item & MuJoCoUni & MotrixSim \\
        \midrule
        Scale list (cylinder sizes) & $\{0.8\ldots1.5\}$ & $\{0.8\ldots1.5\}$ \\
        \texttt{randomize\_gravity\_direction} & true & true \\
        Gravity magnitude & 9.81 & 9.81 \\
        \texttt{randomize\_gravity} (full vector) & false & false \\
        \texttt{randomize\_pd\_gains} & true & true \\
        $K_p$ scale range & $[0.5, 2.0]$ & $[0.5, 2.0]$ \\
        $K_d$ scale range & $[0.5, 2.0]$ & $[0.5, 2.0]$ \\
        \texttt{randomize\_friction} & true & true \\
        Friction scale range & $[0.75, 1.25]$ & $[0.75, 1.25]$ \\
        Elastomer/metal/object base friction & $2.0, 1.0, 2.0$ & $2.0, 1.0, 2.0$ \\
        \texttt{randomize\_com} & true & true \\
        COM offset range & $[-0.01, 0.01]$ & $[-0.01, 0.01]$ \\
        \texttt{randomize\_mass} & true & true \\
        Mass range & $[0.01, 0.25]$ & $[0.01, 0.25]$ \\
        Force perturbation scale & 2.0 & 2.0 \\
        Force probability per step & 0.25 & 0.25 \\
        Force decay / interval & $0.9 / 0.08$ & $0.9 / 0.08$ \\
        Joint observation noise scale & 0.02 & 0.02 \\
        Contact latency & 0.005 & 0.005 \\
        Contact sensor noise & 0.01 & 0.01 \\
        \bottomrule
    \end{tabular}
\end{table}

\noindent\textbf{Reward design.}
Reward scales are identical across the two backends (Table~\ref{tab:app_sharpa_reward}).

\begin{table}[!htbp]
    \centering
    \caption{Reward terms for \texttt{sharpa\_inhand} (mj/mx identical).}
    \label{tab:app_sharpa_reward}
    \begin{tabular}{@{}lc@{}}
        \toprule
        Term & Weight \\
        \midrule
        rotate (\texttt{clip}$(\boldsymbol\omega^{obj}\cdot\hat n,-0.5,0.5)$) & 2.5 \\
        obj\_linvel ($\sum_i |v^{obj}_i|$) & -0.3 \\
        pose\_diff ($\sum_j(q_j-q_j^{def})^2$) & -0.4 \\
        torque (squared virtual torque) & -0.1 \\
        work ($(\sum_j \tau_j \dot q_j)^2$) & -0.5 \\
        object\_pos ($1/(\|p^{obj}-p^{anchor}\|+10^{-3})$) & 0.003 \\
        \bottomrule
    \end{tabular}
\end{table}

The rotate term clips its angular-velocity argument to $[-0.5, 0.5]$\,rad/s before applying the weight.

\subsection{Algorithm Hyperparameters}
\label{app:training_curves_algorithms}

This subsection lists the per-algorithm global defaults and the per-task overrides applied on top of them. Reward weights and environment-side hyperparameters are documented in Section~\ref{app:training_curves_tasks}; only algorithm-side training hyperparameters appear here.

\subsubsection{PPO}
\label{app:algorithm_ppo}

We report PPO hyperparameters as global defaults followed by per-task overrides.

\paragraph{PPO global defaults.}
Table~\ref{tab:app_ppo_default} lists the global defaults inherited by every PPO task before any per-task override.

\begin{table}[!htbp]
    \centering
    \small
    \caption{PPO global default hyperparameters.}
    \label{tab:app_ppo_default}
    \begin{tabular}{@{}ll@{}}
        \toprule
        Field & Default Value \\
        \midrule
        \multicolumn{2}{l}{\emph{Runner / Environment}} \\
        \texttt{algo} & ppo \\
        \texttt{algo\_log\_name} & rsl\_rl\_ppo \\
        \texttt{seed} & $1$ \\
        \texttt{num\_envs} & $4096$ \\
        \texttt{num\_steps\_per\_env} & $24$ \\
        \texttt{max\_iterations} & $101$ \\
        \texttt{save\_interval} & $100$ \\
        \texttt{empirical\_normalization} & false \\
        \texttt{runner\_class\_name} & \texttt{OnPolicyRunner} \\
        \texttt{obs\_groups.default} & \texttt{[policy]} \\
        \midrule
        \multicolumn{2}{l}{\emph{Policy network}} \\
        \texttt{policy.class\_name} & \texttt{ActorCritic} \\
        \texttt{policy.actor\_hidden\_dims} & $[512, 256, 128]$ \\
        \texttt{policy.critic\_hidden\_dims} & $[512, 256, 128]$ \\
        \texttt{policy.activation} & elu \\
        \texttt{policy.init\_noise\_std} & $1.0$ \\
        \midrule
        \multicolumn{2}{l}{\emph{Algorithm}} \\
        \texttt{algorithm.class\_name} & \texttt{FinalObservationAwarePPO} \\
        \texttt{algorithm.value\_loss\_coef} & $1.0$ \\
        \texttt{algorithm.use\_clipped\_value\_loss} & true \\
        \texttt{algorithm.clip\_param} & $0.2$ \\
        \texttt{algorithm.entropy\_coef} & $0.01$ \\
        \texttt{algorithm.num\_learning\_epochs} & $5$ \\
        \texttt{algorithm.num\_mini\_batches} & $4$ \\
        \texttt{algorithm.learning\_rate} & $1.0\times10^{-3}$ \\
        \texttt{algorithm.schedule} & adaptive \\
        \texttt{algorithm.gamma} & $0.99$ \\
        \texttt{algorithm.lam} & $0.95$ \\
        \texttt{algorithm.desired\_kl} & $0.01$ \\
        \texttt{algorithm.max\_grad\_norm} & $1.0$ \\
        \texttt{algorithm.adaptive\_kl\_beta} & $0.9$ \\
        \texttt{algorithm.adaptive\_lr\_growth} & $1.1$ \\
        \texttt{algorithm.adaptive\_lr\_decay} & $1.2$ \\
        \texttt{algorithm.adaptive\_lr\_update\_interval} & $5$ \\
        \bottomrule
    \end{tabular}
\end{table}

\paragraph{PPO overrides across tasks.}
Tables~\ref{tab:app_ppo_loco_overrides}--\ref{tab:app_ppo_hand_overrides} summarize the PPO-side overrides for each task. Fields not listed are inherited from Table~\ref{tab:app_ppo_default}. When the two backends differ, the value is written as ``mj / mx''; identical values are written once.

\begin{table}[!htbp]
    \centering
    \caption{PPO overrides for locomotion tasks (Go1, Go2, Go2W families). Cells with a slash report ``mj~/~mx'' values; single values are shared between the two backends.}
    \label{tab:app_ppo_loco_overrides}
    \resizebox{\textwidth}{!}{%
    \begin{tabular}{@{}lcccccc@{}}
        \toprule
        Field & Go1 Flat & Go1 Rough & Go2 Flat & Go2 Rough & Go2W Flat & Go2W Rough \\
        \midrule
        \texttt{num\_envs}              & $4096$               & $4096$       & $1024$       & $4096$       & $1024$       & $2048$ \\
        \texttt{num\_steps\_per\_env}   & $24$                 & $24$         & $24$         & $24$         & $24$         & $48 / 24$ \\
        \texttt{max\_iterations}        & $151$                & $600$        & $151$        & $1000$       & $151$        & $5000 / 2000$ \\
        \texttt{empirical\_normalization} & false / true       & false        & true         & false        & true         & false \\
        \texttt{init\_noise\_std}       & inherited / $0.5$    & $1.0$        & $0.5$        & $1.0$        & $0.5$        & inherited \\
        \texttt{learning\_rate}         & $10^{-3} / 3{\times}10^{-4}$ & $10^{-3}$ & $3{\times}10^{-4}$ & $10^{-3}$ & $3{\times}10^{-4}$ & inherited \\
        \texttt{entropy\_coef}          & $0.01 / 10^{-3}$     & $0.01$       & $10^{-3}$    & $0.01$       & $10^{-3}$    & inherited \\
        \bottomrule
    \end{tabular}}
\end{table}

For Go1 Joystick Flat, empirical normalization, the lower action-noise std, and the lower learning rate / entropy coefficient are applied only under MotrixSim. Go2 Joystick Flat uses the same lowered values on both backends. Go1 / Go2 Joystick Rough share a single hyperparameter set between the two backends with action-noise std $1.0$ and entropy coefficient $0.01$. Go2W Joystick Flat and Rough use the same hyperparameters on both backends apart from rollout length and iteration count in the Rough case.

\begin{table}[!htbp]
    \centering
    \caption{PPO overrides for humanoid locomotion and tracking tasks. Cells with a slash report ``mj~/~mx'' values; single values are shared between the two backends.}
    \label{tab:app_ppo_g1_overrides}
    \resizebox{\textwidth}{!}{%
    \begin{tabular}{@{}lccccc@{}}
        \toprule
        Field & G1 Walk Flat & G1 Motion & G1 Climb & G1 Flip & G1 Wall Flip \\
        \midrule
        \texttt{num\_envs}              & $2048$                       & $1024$       & $1024$       & $1024$              & $1024$ \\
        \texttt{num\_steps\_per\_env}   & $24$                         & $24$         & $24$         & $24$                & $24$ \\
        \texttt{max\_iterations}        & $2200$                       & $15000$      & $20000$      & $20000 / 30000$     & $20000 / 12000$ \\
        \texttt{empirical\_normalization} & false / true               & false        & true         & true / false        & true \\
        \texttt{init\_noise\_std}       & inherited / $0.5$            & inherited    & inherited    & inherited           & inherited \\
        \texttt{learning\_rate}         & $10^{-3} / 3{\times}10^{-4}$ & $10^{-3}$    & $10^{-3}$    & $10^{-3}$           & $10^{-3}$ \\
        \texttt{entropy\_coef}          & $0.01 / 5{\times}10^{-3}$    & $0.005$      & $0.005$      & $0.005$             & $0.005$ \\
        \texttt{desired\_kl}            & inherited                    & inherited    & $0.01$       & $0.01 / $ inh.      & $0.01$ \\
        \texttt{save\_interval}         & $100$                        & $500$        & $500$        & $500$               & $500$ \\
        \texttt{obs\_groups}            & symmetric / asymmetric       & symmetric    & asymmetric   & asymmetric          & asymmetric \\
        \bottomrule
    \end{tabular}}
\end{table}

Asymmetric observation groups means the actor and critic see different channels, enabling privileged critic observations. G1 Walk Flat enables this only under MotrixSim. G1 Box Tracking uses \texttt{num\_envs}$=1024$, \texttt{max\_iterations}$=30000 / 40000$, empirical normalization false / true, entropy coefficient $0.005 / 0.002$, save interval $500$, and asymmetric observation groups under MotrixSim.

\begin{table}[!htbp]
    \centering
    \caption{PPO overrides for handstand, arm-loco, and dexterous tasks.}
    \label{tab:app_ppo_hand_overrides}
    \begingroup
    \small
    \setlength{\tabcolsep}{3pt}
    \resizebox{\textwidth}{!}{%
    \begin{tabular}{@{}lcccc@{}}
        \toprule
        Field & Go2 HandStand & Go2 Arm Loco & Allegro & Sharpa HORA PPO \\
        \midrule
        \texttt{num\_envs}              & $1024$       & $4096$               & $16384$      & $2048$ \\
        \texttt{num\_steps\_per\_env}   & $24$         & $24$                 & $8$          & $24$ \\
        \texttt{max\_iterations}        & $3000$       & $151$                & $201$        & $301$ \\
        \texttt{empirical\_normalization} & inherited & true                  & true         & true \\
        \texttt{init\_noise\_std}       & $0.5$        & $0.5$                & inherited    & inherited \\
        \texttt{learning\_rate}         & inherited    & $3{\times}10^{-4}$   & inherited    & $10^{-3}$ \\
        \texttt{entropy\_coef}          & $0.005$      & $10^{-3}$            & $0.01$       & $0.01$ \\
        \texttt{value\_loss\_coef}      & inherited    & inherited            & $4.0$        & $4.0$ \\
        \texttt{desired\_kl}            & inherited    & inherited            & $0.02$       & $0.02$ \\
        \texttt{save\_interval}         & inherited    & inherited            & inherited    & $50$ \\
        \texttt{obs\_groups}            & asymmetric   & symmetric            & symmetric    & actor/critic both [actor] \\
        \bottomrule
    \end{tabular}}
    \endgroup
\end{table}

Go2 Arm Manip Loco is available only under MuJoCoUni; the MotrixSim column does not apply. Allegro Inhand and generic Sharpa Inhand use identical hyperparameters on both backends. The Sharpa column reports the HORA PPO setting used for the main Sharpa PPO comparison.

\subsubsection{APPO}
\label{app:algorithm_appo}

APPO is the asynchronous on-policy variant used in UniLab; it shares PPO's clipped-surrogate objective but allows the learner to consume rollouts produced with a slightly stale policy. Only APPO training hyperparameters appear here; task-side values (rewards, observation/action spaces, domain randomization) are documented in the task specifications above.

\paragraph{APPO global defaults.}
Table~\ref{tab:app_appo_default} lists the global defaults inherited by every APPO task before any per-task override.

\begin{table}[!htbp]
    \centering
    \small
    \caption{APPO global default hyperparameters.}
    \label{tab:app_appo_default}
    \begin{tabular}{@{}ll@{}}
        \toprule
        Field & Default Value \\
        \midrule
        \multicolumn{2}{l}{\emph{Runner / Environment}} \\
        \texttt{algo} & appo \\
        \texttt{algo\_log\_name} & appo \\
        \texttt{seed} & $1$ \\
        \texttt{num\_envs} & $2048$ \\
        \texttt{steps\_per\_env} & $24$ \\
        \texttt{max\_iterations} & $150$ \\
        \texttt{save\_interval} & $50$ \\
        \texttt{obs\_groups.actor} & \texttt{\{policy: 0\}} \\
        \midrule
        \multicolumn{2}{l}{\emph{Actor / Critic networks}} \\
        \texttt{actor.class\_name} & \texttt{rsl\_rl.models.MLPModel} \\
        \texttt{actor.hidden\_dims} & $[512, 256, 128]$ \\
        \texttt{actor.activation} & elu \\
        \texttt{actor.obs\_normalization} & false \\
        \texttt{actor.distribution\_cfg.class\_name} & \texttt{GaussianDistribution} \\
        \texttt{actor.distribution\_cfg.init\_std} & $1.0$ \\
        \texttt{actor.distribution\_cfg.std\_type} & scalar \\
        \texttt{critic.class\_name} & \texttt{rsl\_rl.models.MLPModel} \\
        \texttt{critic.hidden\_dims} & $[512, 256, 128]$ \\
        \texttt{critic.activation} & elu \\
        \texttt{critic.obs\_normalization} & false \\
        \midrule
        \multicolumn{2}{l}{\emph{Algorithm}} \\
        \texttt{algorithm.num\_learning\_epochs} & $5$ \\
        \texttt{algorithm.num\_mini\_batches} & $4$ \\
        \texttt{algorithm.clip\_param} & $0.2$ \\
        \texttt{algorithm.gamma} & $0.99$ \\
        \texttt{algorithm.lam} & $0.95$ \\
        \texttt{algorithm.value\_loss\_coef} & $1.0$ \\
        \texttt{algorithm.entropy\_coef} & $0.01$ \\
        \texttt{algorithm.learning\_rate} & $1.0\times10^{-3}$ \\
        \texttt{algorithm.max\_grad\_norm} & $1.0$ \\
        \texttt{algorithm.use\_clipped\_value\_loss} & true \\
        \texttt{algorithm.schedule} & adaptive \\
        \texttt{algorithm.desired\_kl} & $0.01$ \\
        \texttt{algorithm.adaptive\_kl\_factor} & $1.2$ \\
        \texttt{algorithm.adaptive\_lr\_factor} & $1.1$ \\
        \texttt{algorithm.optimizer} & adam \\
        \texttt{algorithm.tau} (target update) & $1.0$ \\
        \texttt{algorithm.target\_update\_freq} & $1$ \\
        \texttt{algorithm.vtrace\_clip\_rho} & $1.0$ \\
        \texttt{algorithm.vtrace\_clip\_c} & $1.0$ \\
        \bottomrule
    \end{tabular}
\end{table}

\paragraph{APPO overrides across tasks.}
Tables~\ref{tab:app_appo_loco_overrides} and ~\ref{tab:app_appo_tracking_overrides} list the per-task overrides. Fields not listed are inherited from Table~\ref{tab:app_appo_default}. When the two backends differ, the value is written as ``mj / mx''; identical values appear once.

\begin{table}[!htbp]
    \centering
    \small
    \caption{APPO overrides for locomotion and dexterous tasks.}
    \label{tab:app_appo_loco_overrides}
    \begin{tabular}{@{}lcccc@{}}
        \toprule
        Field & Go1 Flat & Go2 Flat & Allegro MuJoCo & Sharpa HORA \\
        \midrule
        \texttt{num\_envs} & inherited & inherited & $1024$ & $2048$ \\
        \texttt{steps\_per\_env} & inherited & inherited & $8$ & $8$ \\
        \texttt{max\_iterations} & $150$ & $150$ & $3000$ & $1360$ \\
        \texttt{save\_interval} & inherited & inherited & $5000$ & $170$ \\
        \texttt{training.replay\_queue\_size} & inherited & inherited & $4$ & $8$ \\
        \texttt{actor.obs\_normalization} & inherited & inherited & true & true \\
        \texttt{critic.obs\_normalization} & inherited & inherited & true & true \\
        \texttt{algorithm.value\_loss\_coef} & inherited & inherited & $4.0$ & $4.0$ \\
        \texttt{algorithm.desired\_kl} & inherited & inherited & $0.025$ & $0.04$ \\
        \bottomrule
    \end{tabular}
\end{table}

Go1/Go2 Joystick Flat run under MuJoCoUni only. The Sharpa HORA setting uses \texttt{runtime\_impl=hora\_appo}, separated actor/critic observations, a 9-dimensional privileged embedding, and HORA actor/critic model classes. The generic non-HORA Sharpa APPO setting is not the teacher recipe reported for the Sharpa HORA curves.

\begin{table}[!htbp]
    \centering
    \small
    \caption{APPO overrides for motion-tracking tasks (mj/mx identical for all four).}
    \label{tab:app_appo_tracking_overrides}
    \begin{tabular}{@{}lcccc@{}}
        \toprule
        Field & G1 Motion & G1 Climb & G1 Flip & G1 Wall Flip \\
        \midrule
        \texttt{num\_envs} & $1024$ & $1024$ & $1024$ & $1024$ \\
        \texttt{steps\_per\_env} & inherited & inherited & inherited & inherited \\
        \texttt{max\_iterations} & $5000$ & $20000$ & $5000$ & $5000$ \\
        \texttt{save\_interval} & $500$ & $500$ & $500$ & $500$ \\
        \bottomrule
    \end{tabular}
\end{table}

All four motion-tracking tasks use the same APPO configuration on both backends. G1 Box Tracking is not available under APPO.

\subsubsection{SAC}
\label{app:algorithm_sac}

SAC is the entropy-regularized off-policy actor-critic used in UniLab for replay-buffer experiments. The shared family contains two implementation variants: the standard SAC trainer (\texttt{algo: sac}) and the FlashSAC accelerated variant (\texttt{algo: flashsac}). Both consume rollouts via a replay buffer and respect the off-policy producer/consumer protocol described in the main text.

\paragraph{SAC global defaults.}
Table~\ref{tab:app_sac_default} lists the global defaults inherited by every SAC task before any per-task override.

\begin{table}[!htbp]
    \centering
    \small
    \caption{SAC global default hyperparameters.}
    \label{tab:app_sac_default}
    \begin{tabular}{@{}ll@{}}
        \toprule
        Field & Default Value \\
        \midrule
        \multicolumn{2}{l}{\emph{Runner / Replay}} \\
        \texttt{algo} & sac \\
        \texttt{algo\_log\_name} & fast\_sac \\
        \texttt{seed} & $1$ \\
        \texttt{num\_envs} & $4096$ \\
        \texttt{batch\_size} & $8192$ \\
        \texttt{replay\_buffer\_n} & $512$ \\
        \texttt{updates\_per\_step} & $4$ \\
        \texttt{learning\_starts} & $1$ \\
        \texttt{policy\_frequency} & $4$ \\
        \texttt{env\_steps\_per\_sync} & $1$ \\
        \texttt{max\_iterations} & $500$ \\
        \texttt{save\_interval} & $500$ \\
        \midrule
        \multicolumn{2}{l}{\emph{Network}} \\
        \texttt{actor\_hidden\_dim} & $512$ \\
        \texttt{critic\_hidden\_dim} & $768$ \\
        \texttt{num\_atoms} & $101$ \\
        \texttt{obs\_normalization} & true \\
        \texttt{use\_layer\_norm} & true \\
        \texttt{use\_symmetry} & false \\
        \midrule
        \multicolumn{2}{l}{\emph{Algorithm}} \\
        \texttt{gamma} & $0.97$ \\
        \texttt{tau} & $0.125$ \\
        \texttt{actor\_lr} & $3.0\times10^{-4}$ \\
        \texttt{critic\_lr} & $3.0\times10^{-4}$ \\
        \texttt{algo\_params.alpha\_lr} & $3.0\times10^{-4}$ \\
        \texttt{algo\_params.alpha\_init} & $0.01$ \\
        \texttt{algo\_params.target\_entropy\_ratio} & $0.0$ \\
        \texttt{algo\_params.max\_grad\_norm} & $0.0$ \\
        \texttt{algo\_params.amp\_dtype} & auto \\
        \texttt{algo\_params.use\_compile} & true \\
        \bottomrule
    \end{tabular}
\end{table}

\paragraph{FlashSAC global defaults.}
Table~\ref{tab:app_flashsac_default} gives the resolved FlashSAC defaults. The two recipes differ in actor/critic capacity, replay-buffer warmup length, and the addition of FlashSAC-specific reward / temperature parameters.

\begin{table}[!htbp]
    \centering
    \small
    \caption{FlashSAC global default hyperparameters.}
    \label{tab:app_flashsac_default}
    \begin{tabular}{@{}ll@{}}
        \toprule
        Field & Default Value \\
        \midrule
        \multicolumn{2}{l}{\emph{Runner / Replay}} \\
        \texttt{algo} & flashsac \\
        \texttt{algo\_log\_name} & flash\_sac \\
        \texttt{num\_envs} & $1024$ \\
        \texttt{batch\_size} & $2048$ \\
        \texttt{replay\_buffer\_n} & $512$ \\
        \texttt{updates\_per\_step} & $2$ \\
        \texttt{learning\_starts} & $98$ \\
        \texttt{policy\_frequency} & $2$ \\
        \texttt{max\_iterations} & $5000$ \\
        \texttt{save\_interval} & $1000$ \\
        \midrule
        \multicolumn{2}{l}{\emph{Network}} \\
        \texttt{actor\_hidden\_dim} & $128$ \\
        \texttt{critic\_hidden\_dim} & $256$ \\
        \texttt{num\_atoms} & $101$ \\
        \texttt{obs\_normalization} & false \\
        \texttt{use\_layer\_norm} & false \\
        \texttt{algo\_params.actor\_num\_blocks} & $2$ \\
        \texttt{algo\_params.critic\_num\_blocks} & $2$ \\
        \midrule
        \multicolumn{2}{l}{\emph{Algorithm}} \\
        \texttt{gamma} & $0.97$ \\
        \texttt{tau} & $0.01$ \\
        \texttt{actor\_lr} & $3.0\times10^{-4}$ \\
        \texttt{critic\_lr} & $3.0\times10^{-4}$ \\
        \texttt{algo\_params.normalize\_reward} & true \\
        \texttt{algo\_params.normalized\_g\_max} & $5.0$ \\
        \texttt{algo\_params.actor\_bc\_alpha} & $0.0$ \\
        \texttt{algo\_params.actor\_noise\_zeta\_mu} & $2.0$ \\
        \texttt{algo\_params.actor\_noise\_zeta\_max} & $16$ \\
        \texttt{algo\_params.critic\_min\_v} / \texttt{critic\_max\_v} & $-5.0 / 5.0$ \\
        \texttt{algo\_params.temp\_initial\_value} & $0.01$ \\
        \texttt{algo\_params.temp\_target\_sigma} & $0.15$ \\
        \texttt{algo\_params.temp\_target\_entropy} & null \\
        \texttt{algo\_params.learning\_rate\_init / peak / end} & $3{\times}10^{-4} / 3{\times}10^{-4} / 1.5{\times}10^{-4}$ \\
        \texttt{algo\_params.learning\_rate\_warmup\_steps} & $0$ \\
        \texttt{algo\_params.learning\_rate\_decay\_steps} & $500{,}000$ \\
        \texttt{algo\_params.n\_step} & $1$ \\
        \bottomrule
    \end{tabular}
\end{table}

\paragraph{SAC and FlashSAC overrides across tasks.}
Tables~\ref{tab:app_sac_overrides} and ~\ref{tab:app_flashsac_overrides} summarize the per-task overrides. Fields not listed are inherited from the corresponding default tables. When the two backends differ, the value is written as ``mj / mx''; identical values appear once.

\begin{table}[!htbp]
    \centering
    \small
    \caption{SAC overrides for G1 walk and motion-tracking tasks.}
    \label{tab:app_sac_overrides}
    \begin{tabular}{@{}lccc@{}}
        \toprule
        Field & G1 Walk Flat & G1 Walk Rough & G1 Motion Tracking \\
        \midrule
        \texttt{num\_envs} & $2048$ & $2048$ & $2048$ \\
        \texttt{learning\_starts} & $10 / 1$ & $10 / 1$ & inherited \\
        \texttt{max\_iterations} & $5000$ & $5000$ & $25000$ \\
        \texttt{save\_interval} & $1000$ & $1000$ & $1000$ \\
        \texttt{updates\_per\_step} & $8$ & $8$ & $4$ \\
        \texttt{policy\_frequency} & inherited & inherited & $2$ \\
        \texttt{use\_symmetry} & true / false & true / false & false \\
        \texttt{gamma} & inherited & inherited & $0.99$ \\
        \texttt{tau} & inherited & inherited & $0.05$ \\
        \texttt{num\_atoms} & inherited & inherited & $501$ \\
        \texttt{algo\_params.alpha\_init} & $0.001$ & $0.001$ & $0.1$ \\
        \texttt{algo\_params.target\_entropy\_ratio} & $0.0$ & $0.0$ & $0.5$ \\
        \texttt{algo\_params.max\_grad\_norm} & inherited & inherited & $10.0$ \\
        \bottomrule
    \end{tabular}
\end{table}

G1 Motion Tracking under SAC shares the same environment as the PPO/APPO version; under MotrixSim only the backend identity and the Kp/Kd randomization switches differ from MuJoCoUni.

\begin{table}[!htbp]
    \centering
    \small
    \caption{HORA SAC overrides for Sharpa Inhand Rotation.}
    \label{tab:app_sac_sharpa_hora_overrides}
    \begin{tabular}{@{}ll@{}}
        \toprule
        Field & Sharpa HORA SAC \\
        \midrule
        \texttt{runtime\_impl} & \texttt{hora\_sac} \\
        \texttt{num\_envs} & $1024$ \\
        \texttt{batch\_size} & $2048$ \\
        \texttt{replay\_buffer\_n} & $1280$ \\
        \texttt{training.env\_steps\_per\_sync} & $2$ \\
        \texttt{updates\_per\_step} & $14$ \\
        \texttt{policy\_frequency} & $2$ \\
        \texttt{learning\_starts} & $1$ \\
        \texttt{max\_iterations} & $39063$ \\
        \texttt{save\_interval} & $1000$ \\
        \texttt{actor\_lr}, \texttt{critic\_lr}, \texttt{alpha\_lr} & $4.5{\times}10^{-4}$ \\
        \texttt{training.use\_amp} & true \\
        \texttt{algo\_params.use\_compile} & true \\
        \texttt{actor.priv\_info\_embed\_dim} & $9$ \\
        \texttt{actor.priv\_mlp\_hidden\_dims} & $[256,128,9]$ \\
        \bottomrule
    \end{tabular}
\end{table}

The Sharpa HORA SAC setting keeps the standard SAC replay objective and uses a HORA-style SAC actor that consumes the 9-dimensional privileged tail described in Section~\ref{app:task_dexterous_hand}. Task-side reward, observation, action, and domain-randomization values are therefore documented once in the Sharpa task subsection rather than repeated here.

\begin{table}[!htbp]
    \centering
    \small
    \caption{FlashSAC overrides for G1 Walk Flat and Go2 Joystick Flat.}
    \label{tab:app_flashsac_overrides}
    \begin{tabular}{@{}lcc@{}}
        \toprule
        Field & G1 Walk Flat & Go2 Joystick Flat \\
        \midrule
        \texttt{num\_envs} & $4096$ & $1024$ \\
        \texttt{batch\_size} & inherited & inherited \\
        \texttt{replay\_buffer\_n} & $256$ & $4096$ \\
        \texttt{learning\_starts} & $49$ & $50$ \\
        \texttt{updates\_per\_step} & $8$ & $2$ \\
        \texttt{max\_iterations} & $5000$ & $4000$ \\
        \texttt{save\_interval} & $1000$ & $1000$ \\
        \texttt{tau} & $0.05$ & $0.05$ \\
        \bottomrule
    \end{tabular}
\end{table}

Both FlashSAC tasks are available only under MuJoCoUni.
