# Supplementary material for: UniLab: A Heterogeneous Architecture for Robot RL Beyond GPU-Dominant Paradigms
Source: arXiv:2605.30313 source file (2026-06-02)
Supplement: Supplementary file 5 [file 0_Sim2SimCrossValidation.tex]

\subsection{Bidirectional Sim2Sim Cross-Backend Validation}
\label{app:sim2sim_cross_validation}

\paragraph{Objective.}
This subsection evaluates whether a policy trained against one simulation backend transfers to the other without retraining. We rollout each checkpoint on both MuJoCoUni and MotrixSim and compare its behaviour. Because each task uses backend-specific reward shaping at training time, the absolute reward values from different training backends are not directly comparable; what is meaningful is the change of each metric when the same policy is moved between backends, since this isolates the gap introduced by the simulator rather than by the policy.

\paragraph{Metrics.}
We report three quantities per (policy, evaluation-backend) pair:
\begin{itemize}
    \item \textbf{Mean episodic return:} the mean cumulative reward over 100 evaluation episodes, computed with the reward scale stored with the checkpoint at training time.
    \item \textbf{Success rate:} the fraction of the 100 episodes that finish without early termination.
    \item \textbf{MPJPE (m):} the mean per-joint position error against the reference trajectory, averaged over time and joints. MPJPE is only defined for motion-tracking tasks; locomotion rows report a dash.
\end{itemize}

\paragraph{Protocol.}
All numbers come from zero-shot rollouts of a single trained checkpoint per policy: no fine-tuning, no retraining, and no per-backend adaptation. For each task we evaluate two checkpoints---one trained on MuJoCoUni and one trained on MotrixSim---and run each checkpoint on both backends, yielding four rows per task. The native rows (train backend $=$ test backend) act as the reference; the cross rows (train backend $\ne$ test backend) measure the sim2sim gap. Each cell aggregates 100 episodes. Cross-backend evaluation uses the reward weights and normalization constants associated with the policy's training backend, ensuring that changes reflect simulator transfer rather than reward-definition changes.

\begin{table}[!htbp]
    \centering
    \small
    \caption{Bidirectional sim2sim cross-backend evaluation. For each task, the four rows correspond to: native MotrixSim (train$=$test$=$MotrixSim), forward transfer (MotrixSim$\to$MuJoCoUni), native MuJoCoUni (train$=$test$=$MuJoCoUni), and reverse transfer (MuJoCoUni$\to$MotrixSim). Mean return is comparable only within the four rows of a single task: reward scales are task- and training-backend-specific. A dash in the MPJPE column marks locomotion rows, where no reference trajectory exists.}
    \label{tab:app_sim2sim_cross}
    \resizebox{\textwidth}{!}{%
    \begin{tabular}{@{}llllcccc@{}}
        \toprule
        Test type & Task & Train backend & Test backend & Mean return & Success & MPJPE\,(m) & Episodes \\
        \midrule
        \multicolumn{8}{l}{\emph{G1 Walk Flat (SAC)}} \\
        Native      & G1 Walk Flat       & MotrixSim & MotrixSim & 408.38 & 1.00 & --- & 100 \\
        Forward     & G1 Walk Flat       & MotrixSim & MuJoCoUni & 405.46 & 1.00 & --- & 100 \\
        Native      & G1 Walk Flat       & MuJoCoUni & MuJoCoUni & 354.41 & 1.00 & --- & 100 \\
        Reverse     & G1 Walk Flat       & MuJoCoUni & MotrixSim & 354.00 & 1.00 & --- & 100 \\
        \midrule
        \multicolumn{8}{l}{\emph{G1 Motion Tracking, dance reference (SAC)}} \\
        Native      & G1 Motion Tracking & MotrixSim & MotrixSim & 45.26 & 1.00 & 0.0217 & 100 \\
        Forward     & G1 Motion Tracking & MotrixSim & MuJoCoUni & 45.17 & 1.00 & 0.0219 & 100 \\
        Native      & G1 Motion Tracking & MuJoCoUni & MuJoCoUni & 45.36 & 1.00 & 0.0197 & 100 \\
        Reverse     & G1 Motion Tracking & MuJoCoUni & MotrixSim & 45.34 & 1.00 & 0.0204 & 100 \\
        \midrule
        \multicolumn{8}{l}{\emph{G1 Shuttle-Run Tracking (PPO)}} \\
        Native      & G1 Shuttle-Run     & MotrixSim & MotrixSim & 45.80 & 1.00 & 0.0515 & 100 \\
        Forward     & G1 Shuttle-Run     & MotrixSim & MuJoCoUni & 42.28 & 0.92 & 0.0568 & 100 \\
        Native      & G1 Shuttle-Run     & MuJoCoUni & MuJoCoUni & 32.64 & 0.97 & 0.0519 & 100 \\
        Reverse     & G1 Shuttle-Run     & MuJoCoUni & MotrixSim & 31.95 & 0.91 & 0.0532 & 100 \\
        \midrule
        \multicolumn{8}{l}{\emph{G1 Wall Flip Tracking (PPO)}} \\
        Native      & G1 Wall Flip       & MotrixSim & MotrixSim & 84.46 & 1.00 & 0.0447 & 100 \\
        Forward     & G1 Wall Flip       & MotrixSim & MuJoCoUni & 79.46 & 1.00 & 0.0596 & 100 \\
        Native      & G1 Wall Flip       & MuJoCoUni & MuJoCoUni & 80.61 & 1.00 & 0.0431 & 100 \\
        Reverse     & G1 Wall Flip       & MuJoCoUni & MotrixSim & 77.44 & 1.00 & 0.0620 & 100 \\
        \bottomrule
    \end{tabular}}
\end{table}

Across the four tasks, success rate stays at 1.00 for both locomotion and the two acyclic tracking tasks (dance and wall flip); only the shuttle-run policies drop noticeably (0.97/1.00 native vs.\ 0.92/0.91 cross), and MPJPE remains within $0.0030$\,m of the native baseline for the dance clip, within $0.0053$\,m for the shuttle run, and within $0.0189$\,m for the wall flip. These margins are small relative to the per-joint reference scale and indicate that the policies generalize across the two backends without backend-specific adaptation.
