# Supplementary material for: UniLab: A Heterogeneous Architecture for Robot RL Beyond GPU-Dominant Paradigms
Source: arXiv:2605.30313 source file (2026-06-02)
Supplement: Supplementary file 6 [file 4_TrainingCurves.tex]

\subsection{Training Curves}
\label{app:training_curves_figures}

This subsection collects per-task training curves for the three on-policy and off-policy algorithm families used in the main paper. Each panel plots episode reward against environment steps; the curves are aggregated over seeds and smoothed with a fixed-width moving average. Rewards use the same task-side scales as in Section~\ref{app:training_curves_tasks}, so absolute values are comparable across seeds for the same task but not across tasks. The task subsets shown for each algorithm match the per-task override tables in Section~\ref{app:training_curves_algorithms}: PPO is reported on all sixteen benchmark tasks, APPO on the six tasks with a registered APPO configuration, and SAC / FlashSAC on the five tasks with a replay configuration.

\begin{figure}[H]
    \centering
    \includegraphics[width=0.95\textwidth]{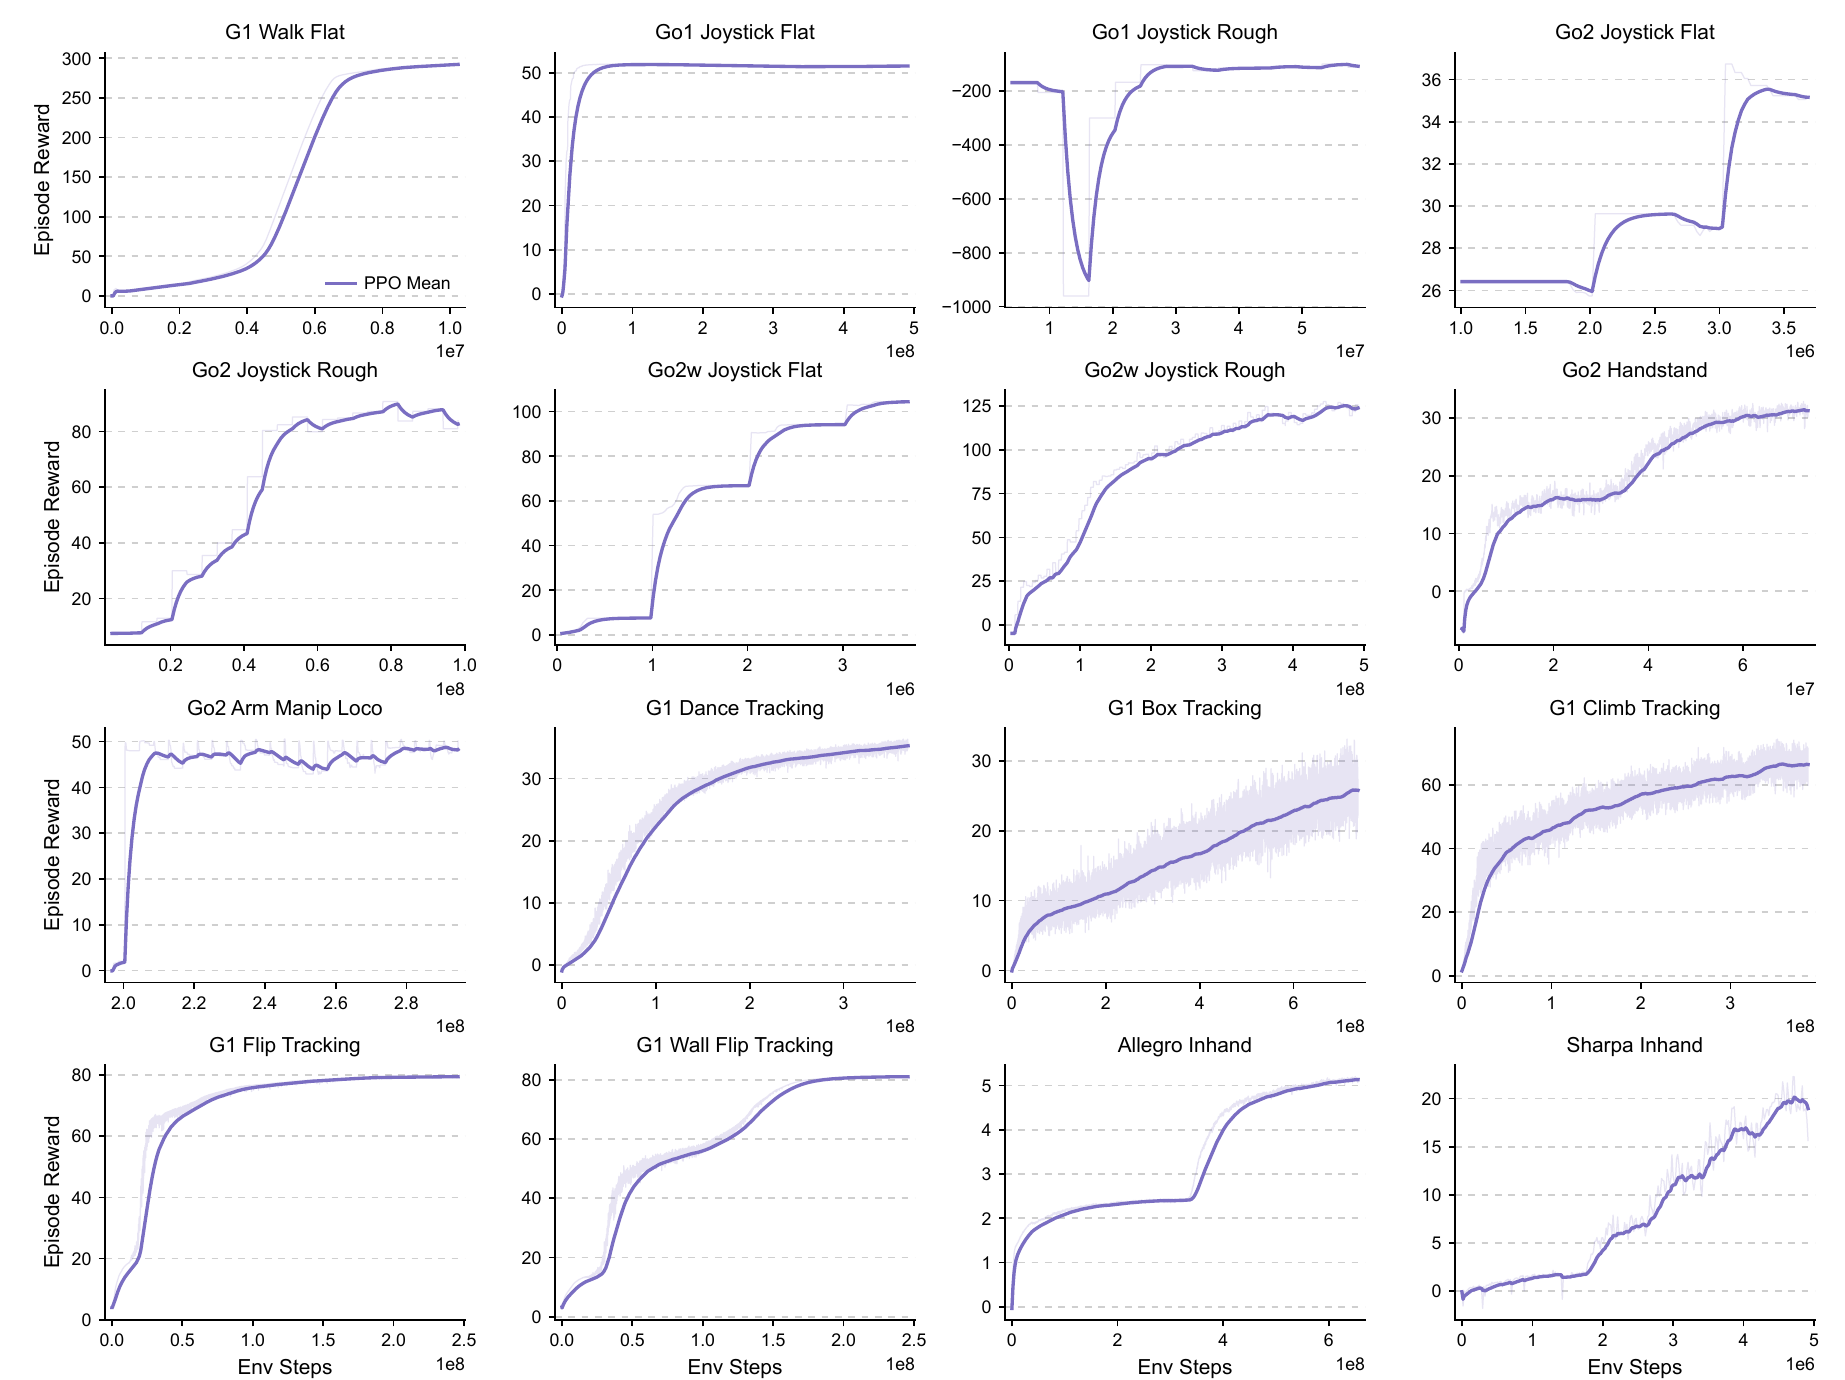}
    \caption{PPO training curves across the sixteen benchmark tasks. Each panel reports episode reward against environment steps; the $x$-axis units differ per panel because environment-step budgets are task-dependent (see Section~\ref{app:training_curves_algorithms}).}
    \label{fig:app_ppo_task_grid}
\end{figure}

\begin{figure}[H]
    \centering
    \includegraphics[width=0.95\textwidth]{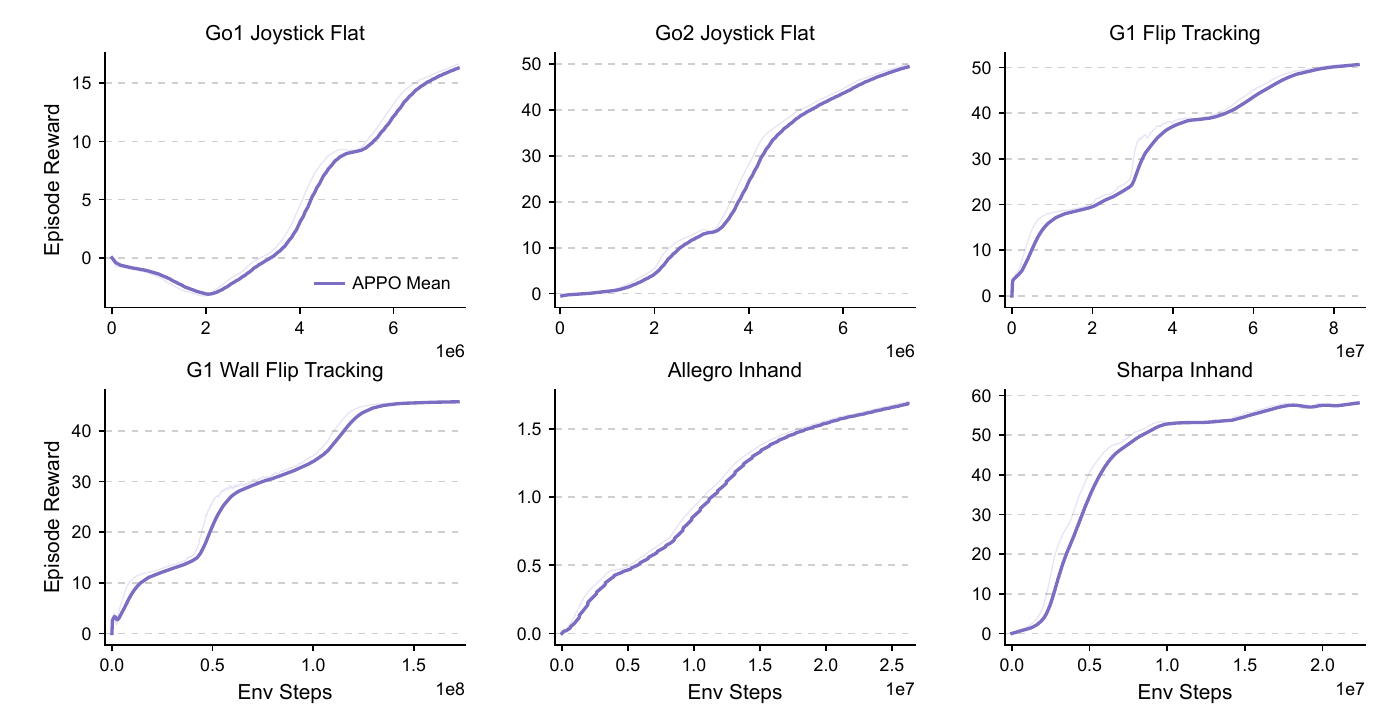}
    \caption{APPO training curves for the six tasks with a registered APPO configuration: Go1 / Go2 Joystick Flat, G1 Flip and Wall Flip Tracking, Allegro Inhand, and Sharpa Inhand (HORA teacher).}
    \label{fig:app_appo_task_grid}
\end{figure}

\begin{figure}[H]
    \centering
    \includegraphics[width=0.95\textwidth]{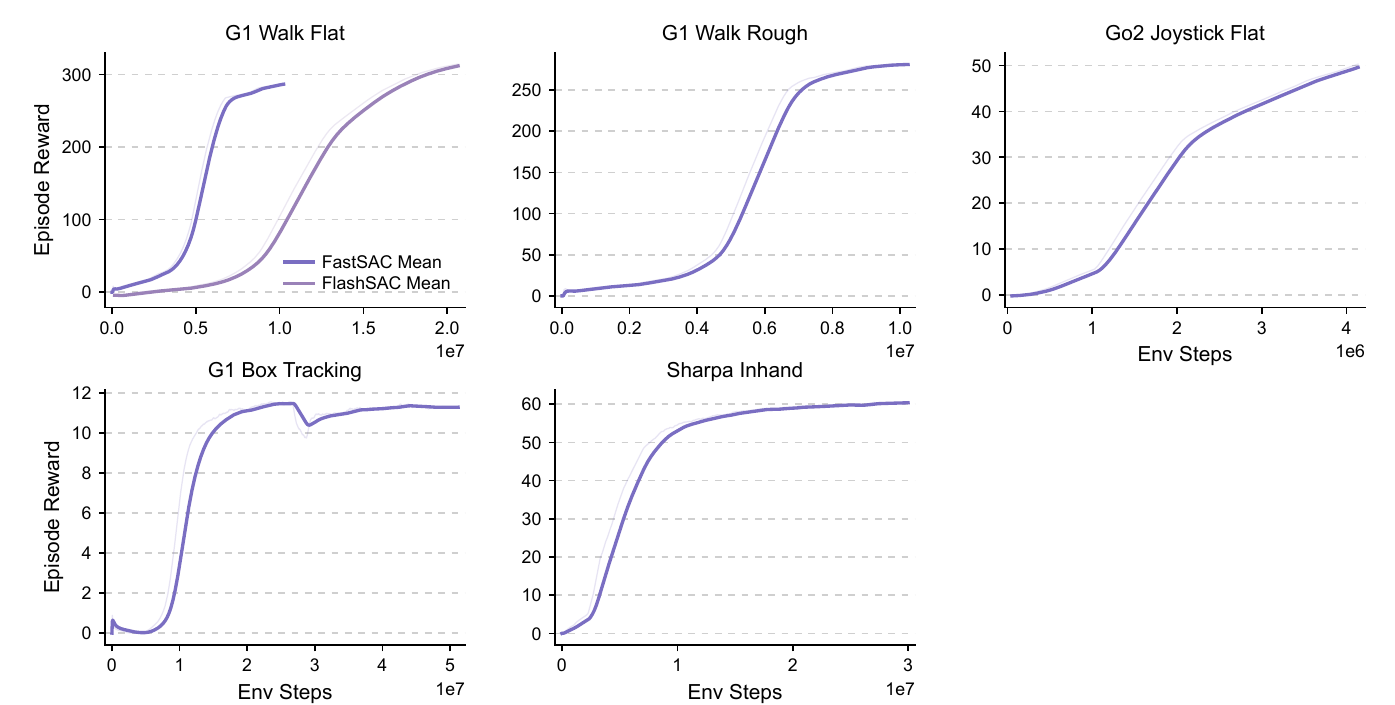}
    \caption{FastSAC and FlashSAC training curves for the five tasks with a replay configuration. G1 Walk Flat reports both FastSAC and FlashSAC; the remaining four tasks (G1 Walk Rough, Go2 Joystick Flat, G1 Box Tracking, Sharpa Inhand) report FastSAC only.}
    \label{fig:app_sac_task_grid}
\end{figure}
