# Supplementary material for: UniLab: A Heterogeneous Architecture for Robot RL Beyond GPU-Dominant Paradigms
Source: arXiv:2605.30313 source file (2026-06-02)
Supplement: Supplementary file 7 [file APPO.tex]

\subsubsection{APPO}
\label{app:algorithm_appo}

APPO is the asynchronous on-policy variant used in UniLab; it shares PPO's clipped-surrogate objective but allows the learner to consume rollouts produced with a slightly stale policy. Only APPO training hyperparameters appear here; task-side values (rewards, observation/action spaces, domain randomization) are documented in the task specifications above.

\paragraph{APPO global defaults.}
Table~\ref{tab:app_appo_default} lists the global defaults inherited by every APPO task before any per-task override.

\begin{table}[!htbp]
    \centering
    \small
    \caption{APPO global default hyperparameters.}
    \label{tab:app_appo_default}
    \begin{tabular}{@{}ll@{}}
        \toprule
        Field & Default Value \\
        \midrule
        \multicolumn{2}{l}{\emph{Runner / Environment}} \\
        \texttt{algo} & appo \\
        \texttt{algo\_log\_name} & appo \\
        \texttt{seed} & $1$ \\
        \texttt{num\_envs} & $2048$ \\
        \texttt{steps\_per\_env} & $24$ \\
        \texttt{max\_iterations} & $150$ \\
        \texttt{save\_interval} & $50$ \\
        \texttt{obs\_groups.actor} & \texttt{\{policy: 0\}} \\
        \midrule
        \multicolumn{2}{l}{\emph{Actor / Critic networks}} \\
        \texttt{actor.class\_name} & \texttt{rsl\_rl.models.MLPModel} \\
        \texttt{actor.hidden\_dims} & $[512, 256, 128]$ \\
        \texttt{actor.activation} & elu \\
        \texttt{actor.obs\_normalization} & false \\
        \texttt{actor.distribution\_cfg.class\_name} & \texttt{GaussianDistribution} \\
        \texttt{actor.distribution\_cfg.init\_std} & $1.0$ \\
        \texttt{actor.distribution\_cfg.std\_type} & scalar \\
        \texttt{critic.class\_name} & \texttt{rsl\_rl.models.MLPModel} \\
        \texttt{critic.hidden\_dims} & $[512, 256, 128]$ \\
        \texttt{critic.activation} & elu \\
        \texttt{critic.obs\_normalization} & false \\
        \midrule
        \multicolumn{2}{l}{\emph{Algorithm}} \\
        \texttt{algorithm.num\_learning\_epochs} & $5$ \\
        \texttt{algorithm.num\_mini\_batches} & $4$ \\
        \texttt{algorithm.clip\_param} & $0.2$ \\
        \texttt{algorithm.gamma} & $0.99$ \\
        \texttt{algorithm.lam} & $0.95$ \\
        \texttt{algorithm.value\_loss\_coef} & $1.0$ \\
        \texttt{algorithm.entropy\_coef} & $0.01$ \\
        \texttt{algorithm.learning\_rate} & $1.0\times10^{-3}$ \\
        \texttt{algorithm.max\_grad\_norm} & $1.0$ \\
        \texttt{algorithm.use\_clipped\_value\_loss} & true \\
        \texttt{algorithm.schedule} & adaptive \\
        \texttt{algorithm.desired\_kl} & $0.01$ \\
        \texttt{algorithm.adaptive\_kl\_factor} & $1.2$ \\
        \texttt{algorithm.adaptive\_lr\_factor} & $1.1$ \\
        \texttt{algorithm.optimizer} & adam \\
        \texttt{algorithm.tau} (target update) & $1.0$ \\
        \texttt{algorithm.target\_update\_freq} & $1$ \\
        \texttt{algorithm.vtrace\_clip\_rho} & $1.0$ \\
        \texttt{algorithm.vtrace\_clip\_c} & $1.0$ \\
        \bottomrule
    \end{tabular}
\end{table}

\paragraph{APPO overrides across tasks.}
Tables~\ref{tab:app_appo_loco_overrides} and ~\ref{tab:app_appo_tracking_overrides} list the per-task overrides. Fields not listed are inherited from Table~\ref{tab:app_appo_default}. When the two backends differ, the value is written as ``mj / mx''; identical values appear once.

\begin{table}[!htbp]
    \centering
    \small
    \caption{APPO overrides for locomotion and dexterous tasks.}
    \label{tab:app_appo_loco_overrides}
    \begin{tabular}{@{}lcccc@{}}
        \toprule
        Field & Go1 Flat & Go2 Flat & Allegro MuJoCo & Sharpa HORA \\
        \midrule
        \texttt{num\_envs} & inherited & inherited & $1024$ & $2048$ \\
        \texttt{steps\_per\_env} & inherited & inherited & $8$ & $8$ \\
        \texttt{max\_iterations} & $150$ & $150$ & $3000$ & $1360$ \\
        \texttt{save\_interval} & inherited & inherited & $5000$ & $170$ \\
        \texttt{training.replay\_queue\_size} & inherited & inherited & $4$ & $8$ \\
        \texttt{actor.obs\_normalization} & inherited & inherited & true & true \\
        \texttt{critic.obs\_normalization} & inherited & inherited & true & true \\
        \texttt{algorithm.value\_loss\_coef} & inherited & inherited & $4.0$ & $4.0$ \\
        \texttt{algorithm.desired\_kl} & inherited & inherited & $0.025$ & $0.04$ \\
        \bottomrule
    \end{tabular}
\end{table}

Go1/Go2 Joystick Flat run under MuJoCoUni only. The Sharpa HORA setting uses \texttt{runtime\_impl=hora\_appo}, separated actor/critic observations, a 9-dimensional privileged embedding, and HORA actor/critic model classes. The generic non-HORA Sharpa APPO setting is not the teacher recipe reported for the Sharpa HORA curves.

\begin{table}[!htbp]
    \centering
    \small
    \caption{APPO overrides for motion-tracking tasks (mj/mx identical for all four).}
    \label{tab:app_appo_tracking_overrides}
    \begin{tabular}{@{}lcccc@{}}
        \toprule
        Field & G1 Motion & G1 Climb & G1 Flip & G1 Wall Flip \\
        \midrule
        \texttt{num\_envs} & $1024$ & $1024$ & $1024$ & $1024$ \\
        \texttt{steps\_per\_env} & inherited & inherited & inherited & inherited \\
        \texttt{max\_iterations} & $5000$ & $20000$ & $5000$ & $5000$ \\
        \texttt{save\_interval} & $500$ & $500$ & $500$ & $500$ \\
        \bottomrule
    \end{tabular}
\end{table}

All four motion-tracking tasks use the same APPO configuration on both backends. G1 Box Tracking is not available under APPO.
