# Supplementary material for: UniLab: A Heterogeneous Architecture for Robot RL Beyond GPU-Dominant Paradigms
Source: arXiv:2605.30313 source file (2026-06-02)
Supplement: Supplementary file 8 [file PPO.tex]

\subsubsection{PPO}
\label{app:algorithm_ppo}

We report PPO hyperparameters as global defaults followed by per-task overrides.

\paragraph{PPO global defaults.}
Table~\ref{tab:app_ppo_default} lists the global defaults inherited by every PPO task before any per-task override.

\begin{table}[!htbp]
    \centering
    \small
    \caption{PPO global default hyperparameters.}
    \label{tab:app_ppo_default}
    \begin{tabular}{@{}ll@{}}
        \toprule
        Field & Default Value \\
        \midrule
        \multicolumn{2}{l}{\emph{Runner / Environment}} \\
        \texttt{algo} & ppo \\
        \texttt{algo\_log\_name} & rsl\_rl\_ppo \\
        \texttt{seed} & $1$ \\
        \texttt{num\_envs} & $4096$ \\
        \texttt{num\_steps\_per\_env} & $24$ \\
        \texttt{max\_iterations} & $101$ \\
        \texttt{save\_interval} & $100$ \\
        \texttt{empirical\_normalization} & false \\
        \texttt{runner\_class\_name} & \texttt{OnPolicyRunner} \\
        \texttt{obs\_groups.default} & \texttt{[policy]} \\
        \midrule
        \multicolumn{2}{l}{\emph{Policy network}} \\
        \texttt{policy.class\_name} & \texttt{ActorCritic} \\
        \texttt{policy.actor\_hidden\_dims} & $[512, 256, 128]$ \\
        \texttt{policy.critic\_hidden\_dims} & $[512, 256, 128]$ \\
        \texttt{policy.activation} & elu \\
        \texttt{policy.init\_noise\_std} & $1.0$ \\
        \midrule
        \multicolumn{2}{l}{\emph{Algorithm}} \\
        \texttt{algorithm.class\_name} & \texttt{FinalObservationAwarePPO} \\
        \texttt{algorithm.value\_loss\_coef} & $1.0$ \\
        \texttt{algorithm.use\_clipped\_value\_loss} & true \\
        \texttt{algorithm.clip\_param} & $0.2$ \\
        \texttt{algorithm.entropy\_coef} & $0.01$ \\
        \texttt{algorithm.num\_learning\_epochs} & $5$ \\
        \texttt{algorithm.num\_mini\_batches} & $4$ \\
        \texttt{algorithm.learning\_rate} & $1.0\times10^{-3}$ \\
        \texttt{algorithm.schedule} & adaptive \\
        \texttt{algorithm.gamma} & $0.99$ \\
        \texttt{algorithm.lam} & $0.95$ \\
        \texttt{algorithm.desired\_kl} & $0.01$ \\
        \texttt{algorithm.max\_grad\_norm} & $1.0$ \\
        \texttt{algorithm.adaptive\_kl\_beta} & $0.9$ \\
        \texttt{algorithm.adaptive\_lr\_growth} & $1.1$ \\
        \texttt{algorithm.adaptive\_lr\_decay} & $1.2$ \\
        \texttt{algorithm.adaptive\_lr\_update\_interval} & $5$ \\
        \bottomrule
    \end{tabular}
\end{table}

\paragraph{PPO overrides across tasks.}
Tables~\ref{tab:app_ppo_loco_overrides}--\ref{tab:app_ppo_hand_overrides} summarize the PPO-side overrides for each task. Fields not listed are inherited from Table~\ref{tab:app_ppo_default}. When the two backends differ, the value is written as ``mj / mx''; identical values are written once.

\begin{table}[!htbp]
    \centering
    \caption{PPO overrides for locomotion tasks (Go1, Go2, Go2W families). Cells with a slash report ``mj~/~mx'' values; single values are shared between the two backends.}
    \label{tab:app_ppo_loco_overrides}
    \resizebox{\textwidth}{!}{%
    \begin{tabular}{@{}lcccccc@{}}
        \toprule
        Field & Go1 Flat & Go1 Rough & Go2 Flat & Go2 Rough & Go2W Flat & Go2W Rough \\
        \midrule
        \texttt{num\_envs}              & $4096$               & $4096$       & $1024$       & $4096$       & $1024$       & $2048$ \\
        \texttt{num\_steps\_per\_env}   & $24$                 & $24$         & $24$         & $24$         & $24$         & $48 / 24$ \\
        \texttt{max\_iterations}        & $151$                & $600$        & $151$        & $1000$       & $151$        & $5000 / 2000$ \\
        \texttt{empirical\_normalization} & false / true       & false        & true         & false        & true         & false \\
        \texttt{init\_noise\_std}       & inherited / $0.5$    & $1.0$        & $0.5$        & $1.0$        & $0.5$        & inherited \\
        \texttt{learning\_rate}         & $10^{-3} / 3{\times}10^{-4}$ & $10^{-3}$ & $3{\times}10^{-4}$ & $10^{-3}$ & $3{\times}10^{-4}$ & inherited \\
        \texttt{entropy\_coef}          & $0.01 / 10^{-3}$     & $0.01$       & $10^{-3}$    & $0.01$       & $10^{-3}$    & inherited \\
        \bottomrule
    \end{tabular}}
\end{table}

For Go1 Joystick Flat, empirical normalization, the lower action-noise std, and the lower learning rate / entropy coefficient are applied only under MotrixSim. Go2 Joystick Flat uses the same lowered values on both backends. Go1 / Go2 Joystick Rough share a single hyperparameter set between the two backends with action-noise std $1.0$ and entropy coefficient $0.01$. Go2W Joystick Flat and Rough use the same hyperparameters on both backends apart from rollout length and iteration count in the Rough case.

\begin{table}[!htbp]
    \centering
    \caption{PPO overrides for humanoid locomotion and tracking tasks. Cells with a slash report ``mj~/~mx'' values; single values are shared between the two backends.}
    \label{tab:app_ppo_g1_overrides}
    \resizebox{\textwidth}{!}{%
    \begin{tabular}{@{}lccccc@{}}
        \toprule
        Field & G1 Walk Flat & G1 Motion & G1 Climb & G1 Flip & G1 Wall Flip \\
        \midrule
        \texttt{num\_envs}              & $2048$                       & $1024$       & $1024$       & $1024$              & $1024$ \\
        \texttt{num\_steps\_per\_env}   & $24$                         & $24$         & $24$         & $24$                & $24$ \\
        \texttt{max\_iterations}        & $2200$                       & $15000$      & $20000$      & $20000 / 30000$     & $20000 / 12000$ \\
        \texttt{empirical\_normalization} & false / true               & false        & true         & true / false        & true \\
        \texttt{init\_noise\_std}       & inherited / $0.5$            & inherited    & inherited    & inherited           & inherited \\
        \texttt{learning\_rate}         & $10^{-3} / 3{\times}10^{-4}$ & $10^{-3}$    & $10^{-3}$    & $10^{-3}$           & $10^{-3}$ \\
        \texttt{entropy\_coef}          & $0.01 / 5{\times}10^{-3}$    & $0.005$      & $0.005$      & $0.005$             & $0.005$ \\
        \texttt{desired\_kl}            & inherited                    & inherited    & $0.01$       & $0.01 / $ inh.      & $0.01$ \\
        \texttt{save\_interval}         & $100$                        & $500$        & $500$        & $500$               & $500$ \\
        \texttt{obs\_groups}            & symmetric / asymmetric       & symmetric    & asymmetric   & asymmetric          & asymmetric \\
        \bottomrule
    \end{tabular}}
\end{table}

Asymmetric observation groups means the actor and critic see different channels, enabling privileged critic observations. G1 Walk Flat enables this only under MotrixSim. G1 Box Tracking uses \texttt{num\_envs}$=1024$, \texttt{max\_iterations}$=30000 / 40000$, empirical normalization false / true, entropy coefficient $0.005 / 0.002$, save interval $500$, and asymmetric observation groups under MotrixSim.

\begin{table}[!htbp]
    \centering
    \caption{PPO overrides for handstand, arm-loco, and dexterous tasks.}
    \label{tab:app_ppo_hand_overrides}
    \begingroup
    \small
    \setlength{\tabcolsep}{3pt}
    \resizebox{\textwidth}{!}{%
    \begin{tabular}{@{}lcccc@{}}
        \toprule
        Field & Go2 HandStand & Go2 Arm Loco & Allegro & Sharpa HORA PPO \\
        \midrule
        \texttt{num\_envs}              & $1024$       & $4096$               & $16384$      & $2048$ \\
        \texttt{num\_steps\_per\_env}   & $24$         & $24$                 & $8$          & $24$ \\
        \texttt{max\_iterations}        & $3000$       & $151$                & $201$        & $301$ \\
        \texttt{empirical\_normalization} & inherited & true                  & true         & true \\
        \texttt{init\_noise\_std}       & $0.5$        & $0.5$                & inherited    & inherited \\
        \texttt{learning\_rate}         & inherited    & $3{\times}10^{-4}$   & inherited    & $10^{-3}$ \\
        \texttt{entropy\_coef}          & $0.005$      & $10^{-3}$            & $0.01$       & $0.01$ \\
        \texttt{value\_loss\_coef}      & inherited    & inherited            & $4.0$        & $4.0$ \\
        \texttt{desired\_kl}            & inherited    & inherited            & $0.02$       & $0.02$ \\
        \texttt{save\_interval}         & inherited    & inherited            & inherited    & $50$ \\
        \texttt{obs\_groups}            & asymmetric   & symmetric            & symmetric    & actor/critic both [actor] \\
        \bottomrule
    \end{tabular}}
    \endgroup
\end{table}

Go2 Arm Manip Loco is available only under MuJoCoUni; the MotrixSim column does not apply. Allegro Inhand and generic Sharpa Inhand use identical hyperparameters on both backends. The Sharpa column reports the HORA PPO setting used for the main Sharpa PPO comparison.
