# Supplementary material for: UniLab: A Heterogeneous Architecture for Robot RL Beyond GPU-Dominant Paradigms
Source: arXiv:2605.30313 source file (2026-06-02)
Supplement: Supplementary file 9 [file SAC.tex]

\subsubsection{SAC}
\label{app:algorithm_sac}

SAC is the entropy-regularized off-policy actor-critic used in UniLab for replay-buffer experiments. The shared family contains two implementation variants: the standard SAC trainer (\texttt{algo: sac}) and the FlashSAC accelerated variant (\texttt{algo: flashsac}). Both consume rollouts via a replay buffer and respect the off-policy producer/consumer protocol described in the main text.

\paragraph{SAC global defaults.}
Table~\ref{tab:app_sac_default} lists the global defaults inherited by every SAC task before any per-task override.

\begin{table}[!htbp]
    \centering
    \small
    \caption{SAC global default hyperparameters.}
    \label{tab:app_sac_default}
    \begin{tabular}{@{}ll@{}}
        \toprule
        Field & Default Value \\
        \midrule
        \multicolumn{2}{l}{\emph{Runner / Replay}} \\
        \texttt{algo} & sac \\
        \texttt{algo\_log\_name} & fast\_sac \\
        \texttt{seed} & $1$ \\
        \texttt{num\_envs} & $4096$ \\
        \texttt{batch\_size} & $8192$ \\
        \texttt{replay\_buffer\_n} & $512$ \\
        \texttt{updates\_per\_step} & $4$ \\
        \texttt{learning\_starts} & $1$ \\
        \texttt{policy\_frequency} & $4$ \\
        \texttt{env\_steps\_per\_sync} & $1$ \\
        \texttt{max\_iterations} & $500$ \\
        \texttt{save\_interval} & $500$ \\
        \midrule
        \multicolumn{2}{l}{\emph{Network}} \\
        \texttt{actor\_hidden\_dim} & $512$ \\
        \texttt{critic\_hidden\_dim} & $768$ \\
        \texttt{num\_atoms} & $101$ \\
        \texttt{obs\_normalization} & true \\
        \texttt{use\_layer\_norm} & true \\
        \texttt{use\_symmetry} & false \\
        \midrule
        \multicolumn{2}{l}{\emph{Algorithm}} \\
        \texttt{gamma} & $0.97$ \\
        \texttt{tau} & $0.125$ \\
        \texttt{actor\_lr} & $3.0\times10^{-4}$ \\
        \texttt{critic\_lr} & $3.0\times10^{-4}$ \\
        \texttt{algo\_params.alpha\_lr} & $3.0\times10^{-4}$ \\
        \texttt{algo\_params.alpha\_init} & $0.01$ \\
        \texttt{algo\_params.target\_entropy\_ratio} & $0.0$ \\
        \texttt{algo\_params.max\_grad\_norm} & $0.0$ \\
        \texttt{algo\_params.amp\_dtype} & auto \\
        \texttt{algo\_params.use\_compile} & true \\
        \bottomrule
    \end{tabular}
\end{table}

\paragraph{FlashSAC global defaults.}
Table~\ref{tab:app_flashsac_default} gives the resolved FlashSAC defaults. The two recipes differ in actor/critic capacity, replay-buffer warmup length, and the addition of FlashSAC-specific reward / temperature parameters.

\begin{table}[!htbp]
    \centering
    \small
    \caption{FlashSAC global default hyperparameters.}
    \label{tab:app_flashsac_default}
    \begin{tabular}{@{}ll@{}}
        \toprule
        Field & Default Value \\
        \midrule
        \multicolumn{2}{l}{\emph{Runner / Replay}} \\
        \texttt{algo} & flashsac \\
        \texttt{algo\_log\_name} & flash\_sac \\
        \texttt{num\_envs} & $1024$ \\
        \texttt{batch\_size} & $2048$ \\
        \texttt{replay\_buffer\_n} & $512$ \\
        \texttt{updates\_per\_step} & $2$ \\
        \texttt{learning\_starts} & $98$ \\
        \texttt{policy\_frequency} & $2$ \\
        \texttt{max\_iterations} & $5000$ \\
        \texttt{save\_interval} & $1000$ \\
        \midrule
        \multicolumn{2}{l}{\emph{Network}} \\
        \texttt{actor\_hidden\_dim} & $128$ \\
        \texttt{critic\_hidden\_dim} & $256$ \\
        \texttt{num\_atoms} & $101$ \\
        \texttt{obs\_normalization} & false \\
        \texttt{use\_layer\_norm} & false \\
        \texttt{algo\_params.actor\_num\_blocks} & $2$ \\
        \texttt{algo\_params.critic\_num\_blocks} & $2$ \\
        \midrule
        \multicolumn{2}{l}{\emph{Algorithm}} \\
        \texttt{gamma} & $0.97$ \\
        \texttt{tau} & $0.01$ \\
        \texttt{actor\_lr} & $3.0\times10^{-4}$ \\
        \texttt{critic\_lr} & $3.0\times10^{-4}$ \\
        \texttt{algo\_params.normalize\_reward} & true \\
        \texttt{algo\_params.normalized\_g\_max} & $5.0$ \\
        \texttt{algo\_params.actor\_bc\_alpha} & $0.0$ \\
        \texttt{algo\_params.actor\_noise\_zeta\_mu} & $2.0$ \\
        \texttt{algo\_params.actor\_noise\_zeta\_max} & $16$ \\
        \texttt{algo\_params.critic\_min\_v} / \texttt{critic\_max\_v} & $-5.0 / 5.0$ \\
        \texttt{algo\_params.temp\_initial\_value} & $0.01$ \\
        \texttt{algo\_params.temp\_target\_sigma} & $0.15$ \\
        \texttt{algo\_params.temp\_target\_entropy} & null \\
        \texttt{algo\_params.learning\_rate\_init / peak / end} & $3{\times}10^{-4} / 3{\times}10^{-4} / 1.5{\times}10^{-4}$ \\
        \texttt{algo\_params.learning\_rate\_warmup\_steps} & $0$ \\
        \texttt{algo\_params.learning\_rate\_decay\_steps} & $500{,}000$ \\
        \texttt{algo\_params.n\_step} & $1$ \\
        \bottomrule
    \end{tabular}
\end{table}

\paragraph{SAC and FlashSAC overrides across tasks.}
Tables~\ref{tab:app_sac_overrides} and ~\ref{tab:app_flashsac_overrides} summarize the per-task overrides. Fields not listed are inherited from the corresponding default tables. When the two backends differ, the value is written as ``mj / mx''; identical values appear once.

\begin{table}[!htbp]
    \centering
    \small
    \caption{SAC overrides for G1 walk and motion-tracking tasks.}
    \label{tab:app_sac_overrides}
    \begin{tabular}{@{}lccc@{}}
        \toprule
        Field & G1 Walk Flat & G1 Walk Rough & G1 Motion Tracking \\
        \midrule
        \texttt{num\_envs} & $2048$ & $2048$ & $2048$ \\
        \texttt{learning\_starts} & $10 / 1$ & $10 / 1$ & inherited \\
        \texttt{max\_iterations} & $5000$ & $5000$ & $25000$ \\
        \texttt{save\_interval} & $1000$ & $1000$ & $1000$ \\
        \texttt{updates\_per\_step} & $8$ & $8$ & $4$ \\
        \texttt{policy\_frequency} & inherited & inherited & $2$ \\
        \texttt{use\_symmetry} & true / false & true / false & false \\
        \texttt{gamma} & inherited & inherited & $0.99$ \\
        \texttt{tau} & inherited & inherited & $0.05$ \\
        \texttt{num\_atoms} & inherited & inherited & $501$ \\
        \texttt{algo\_params.alpha\_init} & $0.001$ & $0.001$ & $0.1$ \\
        \texttt{algo\_params.target\_entropy\_ratio} & $0.0$ & $0.0$ & $0.5$ \\
        \texttt{algo\_params.max\_grad\_norm} & inherited & inherited & $10.0$ \\
        \bottomrule
    \end{tabular}
\end{table}

G1 Motion Tracking under SAC shares the same environment as the PPO/APPO version; under MotrixSim only the backend identity and the Kp/Kd randomization switches differ from MuJoCoUni.

\begin{table}[!htbp]
    \centering
    \small
    \caption{HORA SAC overrides for Sharpa Inhand Rotation.}
    \label{tab:app_sac_sharpa_hora_overrides}
    \begin{tabular}{@{}ll@{}}
        \toprule
        Field & Sharpa HORA SAC \\
        \midrule
        \texttt{runtime\_impl} & \texttt{hora\_sac} \\
        \texttt{num\_envs} & $1024$ \\
        \texttt{batch\_size} & $2048$ \\
        \texttt{replay\_buffer\_n} & $1280$ \\
        \texttt{training.env\_steps\_per\_sync} & $2$ \\
        \texttt{updates\_per\_step} & $14$ \\
        \texttt{policy\_frequency} & $2$ \\
        \texttt{learning\_starts} & $1$ \\
        \texttt{max\_iterations} & $39063$ \\
        \texttt{save\_interval} & $1000$ \\
        \texttt{actor\_lr}, \texttt{critic\_lr}, \texttt{alpha\_lr} & $4.5{\times}10^{-4}$ \\
        \texttt{training.use\_amp} & true \\
        \texttt{algo\_params.use\_compile} & true \\
        \texttt{actor.priv\_info\_embed\_dim} & $9$ \\
        \texttt{actor.priv\_mlp\_hidden\_dims} & $[256,128,9]$ \\
        \bottomrule
    \end{tabular}
\end{table}

The Sharpa HORA SAC setting keeps the standard SAC replay objective and uses a HORA-style SAC actor that consumes the 9-dimensional privileged tail described in Section~\ref{app:task_dexterous_hand}. Task-side reward, observation, action, and domain-randomization values are therefore documented once in the Sharpa task subsection rather than repeated here.

\begin{table}[!htbp]
    \centering
    \small
    \caption{FlashSAC overrides for G1 Walk Flat and Go2 Joystick Flat.}
    \label{tab:app_flashsac_overrides}
    \begin{tabular}{@{}lcc@{}}
        \toprule
        Field & G1 Walk Flat & Go2 Joystick Flat \\
        \midrule
        \texttt{num\_envs} & $4096$ & $1024$ \\
        \texttt{batch\_size} & inherited & inherited \\
        \texttt{replay\_buffer\_n} & $256$ & $4096$ \\
        \texttt{learning\_starts} & $49$ & $50$ \\
        \texttt{updates\_per\_step} & $8$ & $2$ \\
        \texttt{max\_iterations} & $5000$ & $4000$ \\
        \texttt{save\_interval} & $1000$ & $1000$ \\
        \texttt{tau} & $0.05$ & $0.05$ \\
        \bottomrule
    \end{tabular}
\end{table}

Both FlashSAC tasks are available only under MuJoCoUni.
