# Supplementary material for: UniLab: A Heterogeneous Architecture for Robot RL Beyond GPU-Dominant Paradigms
Source: arXiv:2605.30313 source file (2026-06-02)
Supplement: Supplementary file 10 [file DexterousHand.tex]

\subsubsection{Dexterous-Hand and In-Hand Manipulation}
\label{app:task_dexterous_hand}

This subsection covers in-hand manipulation tasks where a multi-finger hand rotates a free object about a specified axis. Two tasks are included: Allegro Inhand Rotation (16-DOF hand, ball) and Sharpa Inhand Rotation (22-DOF hand with tactile sensing).

\paragraph{Allegro Inhand Rotation.}
\texttt{AllegroInhandRotation} rotates a free ball about a fixed world-axis using the 16-DOF Allegro hand. The configuration is identical across the two backends. Simulation step $\Delta t_{\mathrm{sim}}=0.005$\,s, control step $\Delta t_{\mathrm{ctrl}}=0.05$\,s (10 simulator steps per control step), maximum episode 20\,s.

\noindent\textbf{Observation space.}
The observation is 105-dimensional, organized as a lag-history of 3 steps of a 35-dimensional per-step frame:
\begin{equation}
    f_t = [\widetilde q^{hand}_t,\,q^{target}_t,\,p^{ball}_t],
\end{equation}
where $\widetilde q^{hand}_t\in\mathbb{R}^{16}$ is the normalized hand joint position (mapped from joint limits to $[-2,2]$), $q^{target}_t\in\mathbb{R}^{16}$ is the current incremental joint target, and $p^{ball}_t\in\mathbb{R}^3$ is the ball position. Actor and critic share a single observation group; the critic has no privileged channel.

\noindent\textbf{Action space.}
16-dimensional in $[-1,1]$. The environment maps actions to actuator targets incrementally: $q^{target}_t = q^{target}_{t-1} + s\,\mathrm{clip}(a_t)$ with $s = 1/24 \approx 0.0417$, then clipped to the actuator-range limits. PD gains $K_p=1.0$, $K_d=0.1$. Torque is clipped to $[-0.5, 0.5]$.

\noindent\textbf{Commands and termination.}
The rotation axis is the world $z$-axis, $\hat n=(0,0,1)$. The episode terminates when the ball height drops below $0.125$\,m.

\noindent\textbf{Domain randomization.}
All online domain randomization is disabled (base-mass, COM, gravity, push, joint noise, ball-velocity noise, ball-$z$ offset). Reset-time grasp variation is the only source of initialization diversity.

\noindent\textbf{Reward design.}
Reward scales are identical across the two backends (Table~\ref{tab:app_allegro_reward}).

\begin{table}[!htbp]
    \centering
    \caption{Reward terms for \texttt{allegro\_inhand} (mj/mx identical).}
    \label{tab:app_allegro_reward}
    \begin{tabular}{@{}lc@{}}
        \toprule
        Term & Weight \\
        \midrule
        rotate (\texttt{clip}$(\boldsymbol\omega^{ball}\cdot\hat n,-0.5,0.5)$) & 1.25 \\
        obj\_linvel ($\sum_i |v^{ball}_i|$) & -0.3 \\
        pose\_diff ($\sum_j(q_j-q_j^{init})^2$) & -0.3 \\
        torque ($\sum_j \tau_j^2$) & -0.1 \\
        work ($(\sum_j \tau_j \dot q_j)^2$) & -2.0 \\
        \bottomrule
    \end{tabular}
\end{table}

Shaping parameters: angular-velocity clip range $[-0.5, 0.5]$\,rad/s inside the rotate term, and ball-height reset threshold $0.125$\,m used by the termination check. The reward is $\Delta t_{\mathrm{ctrl}}\sum_i w_i r_i$.

\paragraph{Sharpa Inhand Rotation.}
\texttt{SharpaInhandRotation} rotates a cylinder using the 22-DOF Sharpa hand with tactile sensing. The numbers reported here correspond to the MuJoCoUni HORA teacher configuration, which is shared by the APPO, SAC, and PPO HORA comparisons. Simulation step $1/240$\,s, control step $\Delta t_{\mathrm{ctrl}}=12/240=0.05$\,s, maximum episode 20\,s.

\noindent\textbf{Observation space.}
The per-step policy frame is 49-dimensional:
\begin{equation}
    f_t = [\widetilde q^{hand}_t,\,q^{target}_t,\,F^{tactile}_t],
\end{equation}
with $\widetilde q^{hand}_t\in\mathbb{R}^{22}$, $q^{target}_t\in\mathbb{R}^{22}$, and tactile forces $F^{tactile}_t\in\mathbb{R}^5$ (one per fingertip). The frame is stacked over a 3-step lag history, giving a 147-dimensional policy observation. The privileged tail is 9-dimensional: object position delta (3), friction scale (1), mass (1), COM offset (3), and object scale (1). In flattened mode the single observation group is $147+9=156$-dimensional. In separated mode the actor receives the 147-dimensional policy observation, while the critic receives the 156-dimensional concatenation.

\noindent\textbf{Action space.}
22-dimensional in $[-1,1]$. Incremental position control: $q^{target}_t = q^{target}_{t-1} + s\,\mathrm{clip}(a_t)$, $s=1/24$, with joint limits scaled by $0.9$. PD gains are set per actuator and randomized at reset within $[0.5, 2.0]$ around their nominal values.

\noindent\textbf{Commands and termination.}
Rotation axis $\hat n = (0,0,1)$. Termination uses object world-$z$ height bounds $[p^{obj}_z - 0.5\Delta h, p^{obj}_z + 0.5\Delta h]$ with $\Delta h = 0.04$\,m centered on the reset object position; the fallback bounds are $[0.59906, 0.63906]$\,m. The rotation rollout does not use angular-violation termination; angular deviation is used only during offline grasp-state filtering.

\noindent\textbf{Domain randomization.}
A rich randomization stack is enabled on both backends (Table~\ref{tab:app_sharpa_dr}). The reported Sharpa teacher runs use eight cylinder scales $\{0.8\ldots1.5\}$, excluding 1.6 to align with the external baseline setup. The active gravity setting is fixed-magnitude direction randomization; full-vector gravity randomization is disabled.

\begin{table}[!htbp]
    \centering
    \caption{Domain randomization for \texttt{sharpa\_inhand}.}
    \label{tab:app_sharpa_dr}
    \begin{tabular}{@{}lcc@{}}
        \toprule
        Item & MuJoCoUni & MotrixSim \\
        \midrule
        Scale list (cylinder sizes) & $\{0.8\ldots1.5\}$ & $\{0.8\ldots1.5\}$ \\
        \texttt{randomize\_gravity\_direction} & true & true \\
        Gravity magnitude & 9.81 & 9.81 \\
        \texttt{randomize\_gravity} (full vector) & false & false \\
        \texttt{randomize\_pd\_gains} & true & true \\
        $K_p$ scale range & $[0.5, 2.0]$ & $[0.5, 2.0]$ \\
        $K_d$ scale range & $[0.5, 2.0]$ & $[0.5, 2.0]$ \\
        \texttt{randomize\_friction} & true & true \\
        Friction scale range & $[0.75, 1.25]$ & $[0.75, 1.25]$ \\
        Elastomer/metal/object base friction & $2.0, 1.0, 2.0$ & $2.0, 1.0, 2.0$ \\
        \texttt{randomize\_com} & true & true \\
        COM offset range & $[-0.01, 0.01]$ & $[-0.01, 0.01]$ \\
        \texttt{randomize\_mass} & true & true \\
        Mass range & $[0.01, 0.25]$ & $[0.01, 0.25]$ \\
        Force perturbation scale & 2.0 & 2.0 \\
        Force probability per step & 0.25 & 0.25 \\
        Force decay / interval & $0.9 / 0.08$ & $0.9 / 0.08$ \\
        Joint observation noise scale & 0.02 & 0.02 \\
        Contact latency & 0.005 & 0.005 \\
        Contact sensor noise & 0.01 & 0.01 \\
        \bottomrule
    \end{tabular}
\end{table}

\noindent\textbf{Reward design.}
Reward scales are identical across the two backends (Table~\ref{tab:app_sharpa_reward}).

\begin{table}[!htbp]
    \centering
    \caption{Reward terms for \texttt{sharpa\_inhand} (mj/mx identical).}
    \label{tab:app_sharpa_reward}
    \begin{tabular}{@{}lc@{}}
        \toprule
        Term & Weight \\
        \midrule
        rotate (\texttt{clip}$(\boldsymbol\omega^{obj}\cdot\hat n,-0.5,0.5)$) & 2.5 \\
        obj\_linvel ($\sum_i |v^{obj}_i|$) & -0.3 \\
        pose\_diff ($\sum_j(q_j-q_j^{def})^2$) & -0.4 \\
        torque (squared virtual torque) & -0.1 \\
        work ($(\sum_j \tau_j \dot q_j)^2$) & -0.5 \\
        object\_pos ($1/(\|p^{obj}-p^{anchor}\|+10^{-3})$) & 0.003 \\
        \bottomrule
    \end{tabular}
\end{table}

The rotate term clips its angular-velocity argument to $[-0.5, 0.5]$\,rad/s before applying the weight.
