# Supplementary material for: UniLab: A Heterogeneous Architecture for Robot RL Beyond GPU-Dominant Paradigms
Source: arXiv:2605.30313 source file (2026-06-02)
Supplement: Supplementary file 11 [file Locomotion.tex]

\subsubsection{Locomotion}
\label{app:task_locomotion}

\paragraph{Go1 Joystick Flat.}
\texttt{Go1JoystickFlat} runs on the flat Go1 scene with simulation step $\Delta t_{\mathrm{sim}}=0.01$\,s, control step $\Delta t_{\mathrm{ctrl}}=0.02$\,s, maximum episode 20\,s, and initial base position $(0,0,0.34)$.

\noindent\textbf{Observation space.}
The actor observation is 49-dimensional:
\begin{equation}
    o_t = [\omega_t,\,-g_t,\,q_t-q_{\mathrm{default}},\,\dot q_t,\,a_{t-1},\,c_t,\,\phi_t],
\end{equation}
where $\omega_t\in\mathbb{R}^3$ is the body-frame gyro, $g_t\in\mathbb{R}^3$ is the up-vector sensor, $q_t-q_{\mathrm{default}}\in\mathbb{R}^{12}$ is the joint-position offset, $\dot q_t\in\mathbb{R}^{12}$ is joint velocity, $a_{t-1}\in\mathbb{R}^{12}$ is the previous action, $c_t\in\mathbb{R}^3$ is the velocity command, and $\phi_t\in\mathbb{R}^4$ is the four-leg gait phase. The critic observation appends local linear velocity, giving 52 dimensions.

\noindent\textbf{Action space.}
The action is a 12-dimensional joint-position offset. The environment maps policy output $a_t$ to actuator targets by $q^{\mathrm{cmd}}_t = q_{\mathrm{default}} + 0.25\,a_t$, using PD gains $K_p=35.0$, $K_d=0.5$.

\noindent\textbf{Commands and termination.}
The velocity-command range is $[(-0.6,-0.4,-0.8),(1.0,0.4,0.8)]$. An episode terminates early when the up-vector $z$ component satisfies $g^z_t \le 0.5$. Gait frequency is 2\,Hz.

\noindent\textbf{Domain randomization.}
Reset-time domain randomization is applied as listed in Table~\ref{tab:app_go1flat_backend_task_values}.

\begin{table}[!htbp]
    \centering
    \caption{Domain randomization for \texttt{go1\_joystick\_flat}.}
    \label{tab:app_go1flat_backend_task_values}
    \begin{tabular}{@{}lc@{}}
        \toprule
        Item & MuJoCoUni \\
        \midrule
        Velocity-command range & $[(-0.6,-0.4,-0.8),(1.0,0.4,0.8)]$ \\
        \texttt{randomize\_kp} & true (default) \\
        \texttt{randomize\_kd} & true (default) \\
        Kp/Kd multiplier range & $[0.9,1.1]$ \\
        \bottomrule
    \end{tabular}
\end{table}

\noindent\textbf{Reward design.}
The reward is $\Delta t_{\mathrm{ctrl}}\sum_i w_i r_i$. Table~\ref{tab:app_go1flat_reward} lists the active reward scales.

\begin{table}[!htbp]
    \centering
    \caption{Reward terms for \texttt{go1\_joystick\_flat}.}
    \label{tab:app_go1flat_reward}
    \begin{tabular}{@{}lc@{}}
        \toprule
        Term & MuJoCoUni \\
        \midrule
        Linear velocity tracking & 1.0 \\
        Yaw angular velocity tracking & 0.2 \\
        Vertical linear velocity & -5.0 \\
        Roll/pitch angular velocity & -0.1 \\
        Base height & -100.0 \\
        Action rate & -0.005 \\
        Joint deviation from default & -0.1 \\
        Contact phase agreement & 0.24 \\
        Swing-foot height & 4.0 \\
        \bottomrule
    \end{tabular}
\end{table}

The velocity-tracking terms use $\exp(-e^2/\sigma^2)$ with $\sigma=0.25$; the base-height penalty uses a target of $0.3$\,m; the swing-foot term uses $\exp(-e_z^2/0.01)$ gated by the swing phase ($\phi_i \ge 0.6$).

\paragraph{Go1 Joystick Rough.}
\texttt{Go1JoystickRough} adds procedurally generated terrain to the Go1 quadruped. The configuration is identical across the two backends. Simulation step $\Delta t_{\mathrm{sim}}=0.01$\,s, control step $\Delta t_{\mathrm{ctrl}}=0.02$\,s, maximum episode 20\,s.

\noindent\textbf{Observation space.}
The actor observation is 45-dimensional (policy group):
\begin{equation}
    o_t = [0.25\omega_t,\,-g_t,\,c_t,\,q_t-q_{\mathrm{default}},\,0.05\dot q_t,\,a_{t-1}],
\end{equation}
where gyro and joint velocity are pre-scaled. The critic observation is 48-dimensional (adds base linear velocity) plus a height-scan vector (default 187 points from an $11\times17$ grid around the robot base).

\noindent\textbf{Action space.}
The action is 12-dimensional with per-joint scaling: hip joints use \texttt{hip\_action\_scale}$=0.125$, non-hip joints use \texttt{non\_hip\_action\_scale}$=0.25$. PD gains $K_p=35.0$, $K_d=0.5$. Actions are clipped to $[-100, 100]$.

\noindent\textbf{Commands and termination.}
The velocity-command range is $[(-1,-1,-1),(1,1,1)]$ with heading command enabled and resampling every 10\,s. Terrain is procedurally generated on an $8\times8$\,m cell grid ($6\times6$ cells, border width 20\,m). Termination occurs when the robot moves more than 3\,m beyond its terrain cell boundary. No gravity-based termination is used.

\noindent\textbf{Domain randomization.}
Reset-time domain randomization is listed in Table~\ref{tab:app_go1rough_dr}.

\begin{table}[!htbp]
    \centering
    \caption{Domain randomization for \texttt{go1\_joystick\_rough}.}
    \label{tab:app_go1rough_dr}
    \begin{tabular}{@{}lcc@{}}
        \toprule
        Item & MuJoCoUni & MotrixSim \\
        \midrule
        \texttt{randomize\_base\_mass} & true & true \\
        Added mass range & $[-1.0, 3.0]$ & $[-1.0, 3.0]$ \\
        \texttt{random\_com} & true & true \\
        \texttt{randomize\_kp} & true & true \\
        Kp multiplier range & $[0.5, 2.0]$ & $[0.5, 2.0]$ \\
        \texttt{randomize\_kd} & true & true \\
        Kd multiplier range & $[0.5, 2.0]$ & $[0.5, 2.0]$ \\
        \texttt{push\_robots} & true & true \\
        Push interval (steps) & 625 & 625 \\
        Max push force & $[1.0, 1.0, 0.5]$ & $[1.0, 1.0, 0.5]$ \\
        \bottomrule
    \end{tabular}
\end{table}

\noindent\textbf{Reward design.}
Table~\ref{tab:app_go1rough_reward} lists the active reward scales.

\begin{table}[!htbp]
    \centering
    \caption{Reward terms for \texttt{go1\_joystick\_rough}.}
    \label{tab:app_go1rough_reward}
    \small
    \begin{tabular}{@{}lcc@{}}
        \toprule
        Term & MuJoCoUni & MotrixSim \\
        \midrule
        Linear velocity tracking & 3.0 & 3.0 \\
        Yaw angular velocity tracking & 1.5 & 1.5 \\
        Vertical linear velocity & -2.0 & -2.0 \\
        Roll/pitch angular velocity & -0.05 & -0.05 \\
        Joint torques L2 & $-2.5{\times}10^{-5}$ & $-2.5{\times}10^{-5}$ \\
        Joint acceleration L2 & $-2.5{\times}10^{-7}$ & $-2.5{\times}10^{-7}$ \\
        Joint position limits & -5.0 & -5.0 \\
        Joint power & $-2.0{\times}10^{-5}$ & $-2.0{\times}10^{-5}$ \\
        Stand still & -2.0 & -2.0 \\
        Hip position & -0.5 & -0.5 \\
        Joint position penalty & -1.0 & -1.0 \\
        Joint mirror & -0.05 & -0.05 \\
        Action rate & -0.01 & -0.01 \\
        Undesired contacts & -1.0 & -1.0 \\
        Contact forces & $-1.5{\times}10^{-4}$ & $-1.5{\times}10^{-4}$ \\
        Feet air time & 0.5 & 0.5 \\
        Feet air time variance & -1.0 & -1.0 \\
        Feet contact without cmd & 0.1 & 0.1 \\
        Feet slide & -0.1 & -0.1 \\
        Feet height body & -5.0 & -5.0 \\
        Feet gait & 0.5 & 0.5 \\
        Upward & 1.0 & 1.0 \\
        \bottomrule
    \end{tabular}
\end{table}

Tracking-style terms use $\sigma=0.25$ and the base-height penalty uses a target of $0.33$\,m on both backends.

\paragraph{Go2 Joystick Flat.}
\texttt{Go2JoystickFlat} runs on the flat Go2 scene with simulation step $\Delta t_{\mathrm{sim}}=0.01$\,s, control step $\Delta t_{\mathrm{ctrl}}=0.02$\,s, maximum episode 20\,s, and initial base position $(0,0,0.42)$.

\noindent\textbf{Observation space.}
The actor observation is 49-dimensional:
\begin{equation}
    o_t = [\omega_t,\,-g_t,\,q_t-q_{\mathrm{default}},\,\dot q_t,\,a_{t-1},\,c_t,\,\phi_t],
\end{equation}
where $\omega_t\in\mathbb{R}^3$ is the body-frame gyro reading, $g_t\in\mathbb{R}^3$ is the up-vector sensor value, $q_t-q_{\mathrm{default}}\in\mathbb{R}^{12}$ is the joint-position offset from the default pose, $\dot q_t\in\mathbb{R}^{12}$ is joint velocity, $a_{t-1}\in\mathbb{R}^{12}$ is the previous action, $c_t\in\mathbb{R}^3$ is the velocity command, and $\phi_t\in\mathbb{R}^4$ is the foot phase. The critic observation appends local linear velocity, giving a 52-dimensional privileged observation. Observation noise uses the default level.

\noindent\textbf{Action space.}
The action is a 12-dimensional joint-position command offset. The environment maps policy output $a_t$ to actuator targets by
\begin{equation}
    q^{\mathrm{cmd}}_t = q_{\mathrm{default}} + 0.25 a_t,
\end{equation}
using the shared Go2 PD gains $K_p=35.0$ and $K_d=0.5$.

\noindent\textbf{Commands and termination.}
The velocity-command range is $[(-0.6,-0.4,-0.8),(1.0,0.4,0.8)]$. An episode terminates early when the up-vector $z$ component satisfies $g^z_t \le 0.5$.

\noindent\textbf{Domain randomization.}
Reset-time domain randomization is applied as listed in Table~\ref{tab:app_go2_backend_task_values}.

\begin{table}[!htbp]
    \centering
    \caption{Domain randomization for \texttt{go2\_joystick\_flat}.}
    \label{tab:app_go2_backend_task_values}
    \begin{tabular}{@{}lc@{}}
        \toprule
        Item & MuJoCoUni \\
        \midrule
        Velocity-command range & $[(-0.6,-0.4,-0.8),(1.0,0.4,0.8)]$ \\
        \texttt{randomize\_kp} & true \\
        \texttt{randomize\_kd} & true \\
        Kp/Kd multiplier range & $[0.9,1.1]$ \\
        \bottomrule
    \end{tabular}
\end{table}

\noindent\textbf{Reward design.}
The reward is the control-step-scaled sum $\Delta t_{\mathrm{ctrl}}\sum_i w_i r_i$. Table~\ref{tab:app_go2_backend_reward} lists the active reward scales.

\begin{table}[!htbp]
    \centering
    \caption{Reward terms for \texttt{go2\_joystick\_flat}.}
    \label{tab:app_go2_backend_reward}
    \begin{tabular}{@{}lc@{}}
        \toprule
        Term & MuJoCoUni \\
        \midrule
        Linear velocity tracking & 1.0 \\
        Yaw angular velocity tracking & 0.2 \\
        Vertical linear velocity & -5.0 \\
        Roll/pitch angular velocity & -0.1 \\
        Base height & -100.0 \\
        Action rate & -0.005 \\
        Joint deviation from default pose & -0.1 \\
        Contact phase agreement & 0.24 \\
        Swing-foot height & 4.0 \\
        \bottomrule
    \end{tabular}
\end{table}

Tracking-style terms use $\sigma=0.25$ and the base-height penalty uses a target of $0.3$\,m. The swing-foot term rewards swing feet near 0.1\,m height; the contact term compares measured foot contact with the gait phase.

\paragraph{Go2 Joystick Rough.}
\texttt{Go2JoystickRough} shares the same architecture as Go1 Joystick Rough (procedural terrain, height scan, heading command) but uses the Go2 robot model. The configuration is identical across the two backends. Simulation step $\Delta t_{\mathrm{sim}}=0.01$\,s, control step $\Delta t_{\mathrm{ctrl}}=0.02$\,s, maximum episode 20\,s.

\noindent\textbf{Observation space.}
Same structure as Go1 Joystick Rough: actor 45-dimensional (pre-scaled gyro, gravity, command, joint offset, joint velocity, last action), critic 48-dimensional plus height-scan (187 points).

\noindent\textbf{Action space.}
12-dimensional with \texttt{hip\_action\_scale}$=0.125$, \texttt{non\_hip\_action\_scale}$=0.25$. PD gains $K_p=35.0$, $K_d=0.5$. Clip to $[-100, 100]$.

\noindent\textbf{Commands and termination.}
Velocity-command range $[(-1,-1,-1),(1,1,1)]$, heading command enabled, resampling every 10\,s. Terrain: $8\times8$\,m cells, $6\times6$ grid, border 20\,m. Termination: terrain out-of-bounds (3\,m buffer). No gravity-based termination.

\noindent\textbf{Domain randomization.}
Identical to Go1 Joystick Rough (Table~\ref{tab:app_go1rough_dr}): base mass $[-1,3]$\,kg, COM offset, Kp/Kd $[0.5,2.0]$, push robots every 625 steps with force $[1,1,0.5]$.

\noindent\textbf{Reward design.}
Same reward terms and weights as Go1 Joystick Rough (Table~\ref{tab:app_go1rough_reward}), with base-height target $0.33$\,m and tracking sigma $0.25$.

\paragraph{Go2W Joystick Flat.}
\texttt{Go2WJoystickFlat} is a wheeled-legged quadruped with 12 leg joints and 2 wheel joints. The configuration is identical across the two backends. Simulation step $\Delta t_{\mathrm{sim}}=0.01$\,s, control step $\Delta t_{\mathrm{ctrl}}=0.02$\,s, maximum episode 20\,s.

\noindent\textbf{Observation space.}
The actor observation is 53-dimensional:
\begin{equation}
    o_t = [\omega_t,\,-g_t,\,q^{leg}_t{-}q^{leg}_{\mathrm{def}},\,\dot q^{leg}_t,\,\dot q^{wheel}_t,\,a_{t-1},\,c_t],
\end{equation}
where the leg joint offset and velocity are 12-dimensional each, wheel velocity is 2-dimensional, and actions include both leg (12) and wheel (2) outputs. The critic observation is 72-dimensional (adds linear velocity, motor control targets, and wheel control targets).

\noindent\textbf{Action space.}
14-dimensional: 12 leg joints with \texttt{action\_scale}$=0.5$ and 2 wheel joints with \texttt{wheel\_action\_scale}$=10.0$. Leg PD gains $K_p=50.0$, $K_d=1.5$; wheel uses velocity control with $K_d^{wheel}=0.5$.

\noindent\textbf{Commands and termination.}
Velocity-command range $[(0,0,-1),(1,0,1)]$ (forward and yaw only). An episode terminates early when $g^z_t \le 0.5$.

\noindent\textbf{Domain randomization.}
Kp/Kd randomization is disabled. No other domain randomization is enabled in the flat variant.

\noindent\textbf{Reward design.}
Table~\ref{tab:app_go2wflat_reward} lists the active reward scales.

\begin{table}[!htbp]
    \centering
    \caption{Reward terms for \texttt{go2w\_joystick\_flat}.}
    \label{tab:app_go2wflat_reward}
    \begin{tabular}{@{}lcc@{}}
        \toprule
        Term & MuJoCoUni & MotrixSim \\
        \midrule
        Linear velocity tracking & 1.0 & 1.0 \\
        Yaw angular velocity tracking & 0.75 & 0.75 \\
        Vertical linear velocity & -5.0 & -5.0 \\
        Roll/pitch angular velocity & -0.1 & -0.1 \\
        Base height & -100.0 & -100.0 \\
        Orientation & -2.0 & -2.0 \\
        Action rate & -0.005 & -0.005 \\
        Joint deviation from default & -0.5 & -0.5 \\
        Torques & $-2.0{\times}10^{-4}$ & $-2.0{\times}10^{-4}$ \\
        Alive & 0.5 & 0.5 \\
        Upward & 1.0 & 1.0 \\
        \bottomrule
    \end{tabular}
\end{table}

Tracking-style terms use $\sigma=0.25$ and the base-height penalty uses a target of $0.4$\,m on both backends.

\paragraph{Go2W Joystick Rough.}
\texttt{Go2WJoystickRough} adds procedural terrain to the wheeled-legged Go2W. Simulation step $\Delta t_{\mathrm{sim}}=0.01$\,s, control step $\Delta t_{\mathrm{ctrl}}=0.02$\,s, maximum episode 20\,s.

\noindent\textbf{Observation space.}
The actor observation is 53-dimensional (pre-scaled gyro $0.25\omega$, gravity, command, leg joint offset, leg velocity $0.05\dot q$, last action including wheel). The critic observation is 56-dimensional (adds linear velocity) plus height-scan (187 points).

\noindent\textbf{Action space.}
14-dimensional: 12 leg joints with \texttt{action\_scale}$=0.5$ and 2 wheel joints with \texttt{wheel\_action\_scale}$=10.0$. Leg PD gains $K_p=35.0$, $K_d=0.5$; wheel $K_d^{wheel}=0.5$. Clip to $[-100, 100]$.

\noindent\textbf{Commands and termination.}
Velocity-command range $[(-1,-1,-1),(1,1,1)]$, heading command enabled, resampling every 10\,s. Terrain: $8\times8$\,m cells, $6\times6$ grid, border 20\,m. Termination: terrain out-of-bounds (3\,m buffer).

\noindent\textbf{Domain randomization.}
Table~\ref{tab:app_go2wrough_dr} lists the domain-randomization settings. Kp/Kd randomization is enabled under MotrixSim and disabled under MuJoCoUni.

\begin{table}[!htbp]
    \centering
    \caption{Domain randomization for \texttt{go2w\_joystick\_rough}.}
    \label{tab:app_go2wrough_dr}
    \begin{tabular}{@{}lcc@{}}
        \toprule
        Item & MuJoCoUni & MotrixSim \\
        \midrule
        \texttt{randomize\_base\_mass} & true & true \\
        Added mass range & $[-1.0, 3.0]$ & $[-1.0, 3.0]$ \\
        \texttt{random\_com} & true & true \\
        COM offset x & $[-0.05, 0.05]$ & $[-0.05, 0.05]$ \\
        \texttt{randomize\_kp} & false & true \\
        Kp multiplier range & $[0.5, 1.0]$ & $[0.5, 1.0]$ \\
        \texttt{randomize\_kd} & false & true \\
        Kd multiplier range & $[0.5, 1.0]$ & $[0.5, 1.0]$ \\
        \texttt{push\_robots} & true & true \\
        Push interval (steps) & 500 & 625 \\
        Max push force & $[0.5, 0.5, 0.0]$ & $[1.0, 1.0, 0.5]$ \\
        Push body & \texttt{base\_link} & \texttt{base\_link} \\
        \bottomrule
    \end{tabular}
\end{table}

\noindent\textbf{Reward design.}
Table~\ref{tab:app_go2wrough_reward} lists the active reward scales. MotrixSim adds an orientation penalty that MuJoCoUni does not use, and the two backends differ on the hip-position penalty weight.

\begin{table}[!htbp]
    \centering
    \caption{Reward terms for \texttt{go2w\_joystick\_rough}.}
    \label{tab:app_go2wrough_reward}
    \small
    \begin{tabular}{@{}lcc@{}}
        \toprule
        Term & MuJoCoUni & MotrixSim \\
        \midrule
        Linear velocity tracking & 3.0 & 3.0 \\
        Yaw angular velocity tracking & 1.5 & 1.5 \\
        Vertical linear velocity & -2.0 & -2.0 \\
        Roll/pitch angular velocity & -0.05 & -0.05 \\
        Orientation & / & -2.0 \\
        Joint torques L2 & $-2.5{\times}10^{-5}$ & $-2.5{\times}10^{-5}$ \\
        Joint acceleration L2 & $-2.5{\times}10^{-7}$ & $-2.5{\times}10^{-7}$ \\
        Wheel-joint acceleration L2 & $-2.5{\times}10^{-9}$ & $-2.5{\times}10^{-9}$ \\
        Joint position limits & -5.0 & -5.0 \\
        Joint power & $-2.0{\times}10^{-5}$ & $-2.0{\times}10^{-5}$ \\
        Action rate & -0.01 & -0.01 \\
        Stand still & -2.0 & -2.0 \\
        Hip position & -2.0 & -0.5 \\
        Joint position penalty & -1.0 & -1.0 \\
        Joint mirror & -0.05 & -0.05 \\
        Upward & 1.0 & 1.0 \\
        \bottomrule
    \end{tabular}
\end{table}

Tracking-style terms use $\sigma=0.25$ and the base-height penalty uses a target of $0.4$\,m on both backends.

\paragraph{G1 Walk Flat.}
\texttt{G1WalkFlat} is a 29-DOF humanoid locomotion task on the flat G1 scene. Simulation step $\Delta t_{\mathrm{sim}}=0.01$\,s, control step $\Delta t_{\mathrm{ctrl}}=0.02$\,s, maximum episode 20\,s, initial base position $(0,0,0.754)$.

\noindent\textbf{Observation space.}
The actor observation is 98-dimensional:
\begin{equation}
    o_t = [\omega_t,\,-g_t,\,q_t-q_{\mathrm{default}},\,\dot q_t,\,a_{t-1},\,c_t,\,\phi_t],
\end{equation}
where joint offset, joint velocity, and last action are 29-dimensional each, and $\phi_t\in\mathbb{R}^2$ is the bipedal gait phase (left, right). The critic observation is 101-dimensional (adds base linear velocity).

\noindent\textbf{Action space.}
29-dimensional joint-position offset. Action mapping $q^{\mathrm{cmd}}_t = q_{\mathrm{default}} + s\,a_t$ with backend-dependent scale: MuJoCoUni uses $s=0.25$, MotrixSim uses $s=0.5$. PD gains $K_p=50.0$, $K_d=1.0$ (from G1 base config).

\noindent\textbf{Commands and termination.}
Under MuJoCoUni the velocity-command range follows the task default; under MotrixSim it is fixed to $[(0.4,0,0),(0.7,0,0)]$ (forward walking only) with the gait phase initialized at the configured offset and the reset base-velocity limited to $0.05$\,m/s. Termination occurs when body tilt exceeds the configured maximum or the base height drops below the configured minimum: MuJoCoUni uses $25^\circ$ and $0.55$\,m, MotrixSim uses $35^\circ$ and $0.5$\,m.

\noindent\textbf{Domain randomization.}
The velocity curriculum is disabled. Under MotrixSim Kp/Kd randomization is additionally disabled. Observation noise is configured identically on both backends: noise level $1.0$, joint-angle scale $0.01$, joint-velocity scale $1.5$, gyro scale $0.2$.

\noindent\textbf{Reward design.}
Table~\ref{tab:app_g1walkflat_reward} lists the active reward scales. MotrixSim introduces several gait-shaping terms (feet phase contrast, feet phase contact, double-stance penalty, under-speed penalty, upper-body pose) that are not used under MuJoCoUni.

\begin{table}[!htbp]
    \centering
    \caption{Reward terms for \texttt{g1\_walk\_flat}.}
    \label{tab:app_g1walkflat_reward}
    \small
    \begin{tabular}{@{}lcc@{}}
        \toprule
        Term & MuJoCoUni & MotrixSim \\
        \midrule
        Linear velocity tracking & 2.0 & 2.0 \\
        Yaw angular velocity tracking & 0.2 & 0.25 \\
        Feet phase & 1.0 & 1.2 \\
        Feet phase contrast & / & 1.5 \\
        Feet phase contact & / & 1.0 \\
        Feet double stance & / & -1.0 \\
        Under speed & / & -0.2 \\
        Upper body pose & / & -0.05 \\
        Vertical linear velocity & -1.0 & -1.0 \\
        Roll/pitch angular velocity & -0.25 & -0.2 \\
        Base height & -500.0 & -120.0 \\
        Orientation & -5.0 & -2.5 \\
        Action rate & -0.01 & -0.005 \\
        Pose (weighted) & -0.1 & -0.05 \\
        \bottomrule
    \end{tabular}
\end{table}

Shaping parameters used by the table above: velocity-tracking $\sigma=0.25$, gait frequency $1.5$\,Hz, feet-phase swing height $0.09$\,m, feet-phase tracking $\sigma=0.008$, base-height target $0.754$\,m (MuJoCoUni) / $0.765$\,m (MotrixSim). The 29-entry pose-weight vector is identical on both backends. Under MotrixSim, the gait reward is gated by a minimum forward speed of $0.05$\,m/s.

\paragraph{G1 Walk Rough.}
\texttt{G1WalkRough} is the rough-terrain variant trained with SAC on both backends. The environment shares the same 29-DOF humanoid structure as G1 Walk Flat with terrain-aware reset behaviour.

\noindent\textbf{Observation space.}
Same structure as G1 Walk Flat: actor 98-dimensional, critic 101-dimensional. Refer to the G1 Walk Flat paragraph for the layout.

\noindent\textbf{Action space.}
29-dimensional joint-position offset with action scale $s=1.0$ (raised from the task default $0.25$). PD gains $K_p=50.0$, $K_d=1.0$.

\noindent\textbf{Commands and termination.}
The gait phase is initialized at the configured offset and the reset base-velocity is limited to $0.5$\,m/s. A base-velocity curriculum is enabled with initial scale $0.5$, maximum scale $1.0$, level-down threshold $150$, level-up threshold $750$, and degree $0.001$. Under MotrixSim, Kp/Kd randomization is disabled and the simulation step is set to $0.01$\,s. Termination uses a maximum tilt of $65^\circ$ and a minimum base height of $0.3$\,m.

\noindent\textbf{Domain randomization.}
Under MuJoCoUni, observation noise uses level $1.0$ with joint-angle scale $0.01$ and joint-velocity scale $0.1$ (other channels zero). Under MotrixSim, the default noise level is used. MuJoCoUni enables policy symmetry at the algorithm level; MotrixSim does not. Mass, COM, and push randomization are not enabled on either backend.

\noindent\textbf{Reward design.}
Table~\ref{tab:app_g1walkrough_reward} lists the active reward scales. MotrixSim uses a tighter feet-phase tracking sigma than MuJoCoUni.

\begin{table}[!htbp]
    \centering
    \caption{Reward terms for \texttt{g1\_walk\_rough}.}
    \label{tab:app_g1walkrough_reward}
    \begin{tabular}{@{}lcc@{}}
        \toprule
        Term & MuJoCoUni & MotrixSim \\
        \midrule
        Linear velocity tracking & 2.0 & 2.2 \\
        Yaw angular velocity tracking & 1.5 & 1.8 \\
        Penalty ang vel xy & -1.0 & -1.2 \\
        Penalty orientation & -10.0 & -12.0 \\
        Penalty action rate & -4.0 & -2.5 \\
        Pose (weighted) & -0.5 & -0.6 \\
        Penalty feet orientation & -20.0 & -5.0 \\
        Feet phase & 5.0 & 6.0 \\
        Alive & 10.0 & 12.0 \\
        \bottomrule
    \end{tabular}
\end{table}

Shaping parameters used by the table above: velocity-tracking $\sigma=0.25$, gait frequency $1.5$\,Hz, feet-phase swing height $0.09$\,m, feet-phase tracking $\sigma=0.04$ (MuJoCoUni) / $0.008$ (MotrixSim), close-feet threshold $0.15$\,m, base-height target $0.754$\,m. Termination thresholds (maximum tilt $65^\circ$, minimum base height $0.3$\,m) are repeated here from the Commands and termination paragraph for reference.
