# Supplementary material for: UniLab: A Heterogeneous Architecture for Robot RL Beyond GPU-Dominant Paradigms
Source: arXiv:2605.30313 source file (2026-06-02)
Supplement: Supplementary file 12 [file ManipulationLocomotion.tex]

\subsubsection{Manipulation-Locomotion}
\label{app:task_manipulation_locomotion}

This subsection covers tasks where locomotion is coupled with an upper-body manipulation or posture objective. Two tasks are included: Go2 Hand Stand (rear-leg balance) and Go2 Arm Manip Loco (locomotion with a 6-DOF arm tracking an end-effector goal).

\paragraph{Go2 Hand Stand.}
\texttt{Go2HandStand} rewards the robot for inverting onto its front legs while maintaining a target torso height. Under MuJoCoUni the simulation step is $0.005$\,s; under MotrixSim it is $0.01$\,s. Control step $\Delta t_{\mathrm{ctrl}}=0.02$\,s, maximum episode 20\,s.

\noindent\textbf{Observation space.}
The actor observation is 42-dimensional:
\begin{equation}
    o_t = [\omega_t,\,-g_t,\,q_t-q_{\mathrm{default}},\,\dot q_t,\,a_{t-1}],
\end{equation}
where joint offset, joint velocity, and last action are 12-dimensional each. No velocity command channel; the task is a fixed posture-tracking objective. The critic observation is 46-dimensional (adds base linear velocity 3 and torso height 1).

\noindent\textbf{Action space.}
12-dimensional joint-position offset with default \texttt{action\_scale}. PD gains $K_p=35.0$, $K_d=0.5$.

\noindent\textbf{Commands and termination.}
The target pose is inverted handstand: target torso height $z_{des}=0.55$\,m, desired gravity $g_{des}=(-1,0,0)$ (body $x$-axis aligned with world gravity). Termination occurs when the up-vector $z$-component satisfies $g^z_t \le -0.25$ (robot fully inverted past the target) or when undesired contacts on front legs/hips/thighs occur. A rear-leg gait at 2\,Hz (RL phase 0, RR phase 0.5) provides a phase signal for the gait-aware reward terms.

\noindent\textbf{Domain randomization.}
Under MotrixSim, Kp/Kd randomization is disabled. No additional domain randomization is enabled on top of the environment defaults.

\noindent\textbf{Reward design.}
Table~\ref{tab:app_go2hs_reward} lists the active reward scales. The two backends differ only in the front-leg contact weight.

\begin{table}[!htbp]
    \centering
    \caption{Reward terms for \texttt{go2\_handstand}.}
    \label{tab:app_go2hs_reward}
    \begin{tabular}{@{}lcc@{}}
        \toprule
        Term & MuJoCoUni & MotrixSim \\
        \midrule
        Contact (front-leg) & -1.0 & -0.5 \\
        Height & 1.0 & 1.0 \\
        Orientation (alignment to target gravity) & 1.0 & 1.0 \\
        Pose (deviation from default) & -0.3 & -0.3 \\
        Penalty contact (penalty bodies) & -0.2 & -0.2 \\
        Action rate & -0.01 & -0.01 \\
        Target pose (\texttt{tar}) & 0.3 & 0.3 \\
        Feet air time (rear legs) & 1.0 & 1.0 \\
        World $z$-velocity penalty & -1.0 & -1.0 \\
        \bottomrule
    \end{tabular}
\end{table}

Shaping parameters: velocity-tracking $\sigma=0.25$ and base-height target $0.3$\,m on both backends. The \texttt{height} term uses $\exp(-|z_{des}-h|/0.1)$, the \texttt{orientation} term uses $[0.5\cos\angle(g,g_{des})+0.5]^2$, and the \texttt{tar} reward is gated by $h \ge 0.8\,z_{des}$.

\paragraph{Go2 Arm Manip Loco.}
\texttt{Go2ArmManipLoco} is available only on the MuJoCoUni backend. Simulation step $\Delta t_{\mathrm{sim}}=0.01$\,s, control step $\Delta t_{\mathrm{ctrl}}=0.02$\,s, maximum episode 20\,s.

\noindent\textbf{Observation space.}
The per-step observation is 79-dimensional:
\begin{equation}
    o_t = [v^{base}_t,\,\omega_t,\,-g_t,\,c_t,\,\phi_t,\,q_t-q_{\mathrm{default}},\,\dot q_t,\,p^{ee}_t,\,p^{goal}_t,\,e^{ee}_t,\,a_{t-1}],
\end{equation}
where $\phi_t\in\mathbb{R}^4$ is the four-foot gait phase, joint offset/velocity are 18-dimensional each (12 leg + 6 arm), $p^{ee}_t,\,p^{goal}_t,\,e^{ee}_t\in\mathbb{R}^3$ are end-effector position, goal, and error in body frame, and the action history is 18-dimensional. The actor observation drops base linear velocity (to avoid bypassing the on-board estimator) and uses a per-step history of $H_a$ frames; the critic observation keeps linear velocity and uses $H_c$ frames. Default history length is $H_a=H_c=1$.

\noindent\textbf{Action space.}
18-dimensional: 12 leg-joint offsets with action scale $0.25$ (hip-joint scale $0.125$) and 6 arm-joint offsets with arm action scale zero. Leg PD gains $K_p=35.0$, $K_d=0.5$. With the arm scale set to zero, the policy controls only the legs; the arm follows the IK-derived target from the end-effector goal.

\noindent\textbf{End-effector goal sampling.}
The end-effector goal is sampled in spherical coordinates around the body: radius $\in[0.3,0.6]$\,m, azimuth $\in[-1.26,1.05]$\,rad, polar angle $\in[-2.36,2.36]$\,rad. Trajectory time $\in[1.0,3.0]$\,s, hold time $\in[0.5,2.0]$\,s. Collision bounds: upper $[0.3,0.15,-0.115]$, lower $[-0.2,-0.15,-0.515]$, underground limit $z=-0.57$. The IK uses damping $0.05$, gain $1.0$, $\Delta q$-clip $0.2$, with target-orientation tracking.

\noindent\textbf{Commands and termination.}
Velocity-command range $[(-0.6,-0.4,-0.8),(1.0,0.4,0.8)]$, zero-command probability $0.15$ (for stable standing), command resampling every $4.0$\,s. The velocity curriculum is disabled. Termination: $g^z_t \le 0.5$.

\noindent\textbf{Domain randomization.}
The following terms are enabled: body-mass multiplier $[0.9, 1.1]$, random COM offset $x\in[-0.03,0.03]$, ground-friction multiplier $[0.8,1.2]$, DOF-armature multiplier $[0.8,1.2]$, base pushes every 500 steps with maximum force $[1.2,1.2,0.6]$, and Kp/Kd multipliers $[0.9,1.1]$. Base-mass and gravity randomization are not enabled.

\noindent\textbf{Reward design.}
Table~\ref{tab:app_go2arml_reward} lists the active reward scales.

\begin{table}[!htbp]
    \centering
    \caption{Reward terms for \texttt{go2\_arm\_manip\_loco}.}
    \label{tab:app_go2arml_reward}
    \begin{tabular}{@{}lc@{}}
        \toprule
        Term & MuJoCoUni \\
        \midrule
        Linear velocity tracking & 2.0 \\
        Yaw angular velocity tracking & 0.5 \\
        Vertical linear velocity & -5.0 \\
        Roll/pitch angular velocity & -0.1 \\
        Roll & -5.0 \\
        Base height & -100.0 \\
        Leg pose & -0.1 \\
        Action rate & -0.005 \\
        Stand still & -0.5 \\
        Contact phase agreement & 0.24 \\
        Swing-foot height & 4.0 \\
        Foot drag & -0.1 \\
        Object distance (to EE goal) & 2.0 \\
        Object distance L2 & -0.5 \\
        Arm collision & -1.0 \\
        \bottomrule
    \end{tabular}
\end{table}

Shaping parameters: velocity-tracking $\sigma=0.25$, base-height target $0.3$\,m, object-distance kernel $\sigma=0.1$.
