# Supplementary material for: UniLab: A Heterogeneous Architecture for Robot RL Beyond GPU-Dominant Paradigms
Source: arXiv:2605.30313 source file (2026-06-02)
Supplement: Supplementary file 13 [file MotionTracking.tex]

\subsubsection{Motion Tracking}
\label{app:task_motion_tracking}

The motion-tracking family imitates a reference motion clip on the 29-DOF G1 humanoid. All five tasks (\texttt{g1\_motion\_tracking}, \texttt{g1\_climb\_tracking}, \texttt{g1\_flip\_tracking}, \texttt{g1\_wall\_flip\_tracking}, \texttt{g1\_box\_tracking}) share the same observation/action layout and reward-term library; they differ in reference motion clip, scene, sampling mode, and termination thresholds. The shared structure is described once under G1 Motion Tracking; per-variant deltas follow.

\paragraph{G1 Motion Tracking.}
\texttt{G1MotionTracking} runs on the flat G1 scene with a dance reference clip. The configuration is identical across the two backends. Simulation step from the G1 base config, control step $\Delta t_{\mathrm{ctrl}}=0.02$\,s, maximum episode 10\,s.

\noindent\textbf{Observation space.}
The actor observation is 176-dimensional:
\begin{equation}
    o^{actor}_t = [m^{joint}_t,\,p^{ref}_{b,t},\,R^{ref}_{b,t},\,v^{base}_t,\,\omega_t,\,q_t-q_{\mathrm{default}},\,\dot q_t,\,a_{t-1}],
\end{equation}
where $m^{joint}_t\in\mathbb{R}^{58}$ is the reference joint position and velocity (29+29), $p^{ref}_{b,t}\in\mathbb{R}^3$ is the reference anchor position in body frame, $R^{ref}_{b,t}\in\mathbb{R}^6$ is the reference anchor orientation (6D rotation representation), and the remaining channels mirror the locomotion observation layout for 29 joints. The critic observation appends per-body privileged transforms for all 14 tracked bodies (3D position + 6D orientation each, $14\times9=126$ extra dims), giving a 302-dimensional critic.

The 14 tracked bodies are: \texttt{pelvis}, left/right \{\texttt{hip\_roll\_link}, \texttt{knee\_link}, \texttt{ankle\_roll\_link}\}, \texttt{torso\_link} (anchor body), left/right \{\texttt{shoulder\_roll\_link}, \texttt{elbow\_link}, \texttt{wrist\_yaw\_link}\}.

\noindent\textbf{Action space.}
29-dimensional joint-position offset with a per-joint 29-element action scale (not a single scalar). PD gains from the G1 base config ($K_p=50.0$, $K_d=1.0$).

\noindent\textbf{Commands and termination.}
There is no joystick command channel; the reference motion plays the role of command. Termination occurs when any of the following holds: anchor-position $z$-error exceeds $0.25$\,m, end-effector $z$-error exceeds $0.25$\,m, or a non-EE body falls below $0.05$\,m when undesired-contact termination is enabled. Anchor-orientation termination is disabled.

\noindent\textbf{Reference-clip sampling.}
The per-environment start frame is chosen at reset by one of four modes: always frame zero, random clip start, uniform over all frames, or failure-weighted adaptive bin sampling. G1 Motion Tracking uses the adaptive mode.

\noindent\textbf{Domain randomization.}
Under MuJoCoUni, observation noise uses the environment defaults. Under MotrixSim, noise level $1.0$ is enabled with joint-angle scale $0.01$, joint-velocity scale $1.5$, and gyro scale $0.2$. Base-mass, COM, gravity, push, and Kp/Kd randomization are not enabled.

\noindent\textbf{Reward design.}
Each motion-tracking term has the form $\exp(-e^2/\sigma^2)$ where $e$ is the reference-tracking error in the corresponding channel; non-tracking penalties use squared / L2 forms identical to the locomotion library. Table~\ref{tab:app_g1mt_reward} lists the active scales.

\begin{table}[!htbp]
    \centering
    \caption{Reward terms for \texttt{g1\_motion\_tracking}.}
    \label{tab:app_g1mt_reward}
    \begin{tabular}{@{}lcc@{}}
        \toprule
        Term & MuJoCoUni & MotrixSim \\
        \midrule
        motion\_global\_root\_pos & 0.5 & 1.0 \\
        motion\_global\_root\_ori & 0.5 & 0.5 \\
        motion\_body\_pos & 1.0 & 1.0 \\
        motion\_body\_ori & 1.0 & 1.0 \\
        motion\_body\_lin\_vel & 1.0 & 1.0 \\
        motion\_body\_ang\_vel & 1.0 & 1.0 \\
        action\_rate\_l2 & -0.1 & -0.05 \\
        joint\_limit & -10.0 & -10.0 \\
        undesired\_contacts & / & -0.1 \\
        \bottomrule
    \end{tabular}
\end{table}

Shaping parameters (per-channel tracking $\sigma$ used inside the $\exp(-e^2/\sigma^2)$ form) are identical on the two backends: $\sigma_{\mathrm{root\_pos}}=0.3$, $\sigma_{\mathrm{root\_ori}}=0.4$, $\sigma_{\mathrm{body\_pos}}=0.3$, $\sigma_{\mathrm{body\_ori}}=0.4$, $\sigma_{\mathrm{body\_lin\_vel}}=1.0$, $\sigma_{\mathrm{body\_ang\_vel}}=3.14$, $\sigma_{\mathrm{joint\_pos}}=0.2$, $\sigma_{\mathrm{joint\_vel}}=1.0$. The joint-position and joint-velocity tracking terms are not used in this configuration.

\paragraph{G1 Climb Tracking.}
The climb variant uses a scene with a 20-rung wall and a matched climbing reference clip. Maximum episode is $15$\,s, sampling is adaptive, simulation step is $0.005$\,s, undesired-contact termination is enabled, and anchor/end-effector $z$-error thresholds are both $0.3$\,m. The episode is not truncated when the clip ends.

The per-joint action scale is roughly $0.55$ for hip and ankle joints, $0.35$ for the knee, $0.44$ for waist and shoulder joints, and $0.07$ for wrist joints. Observation, action, and termination structure match G1 Motion Tracking.

\noindent\textbf{Reward design.}
Reward scales are identical across the two backends (Table~\ref{tab:app_g1ct_reward}). Compared to G1 Motion Tracking, the climb variant additionally weights end-effector vertical tracking, joint-position tracking, and joint-velocity tracking to encourage limb coordination with the reference clip.

\begin{table}[!htbp]
    \centering
    \caption{Reward terms for \texttt{g1\_climb\_tracking} (mj/mx identical).}
    \label{tab:app_g1ct_reward}
    \begin{tabular}{@{}lc@{}}
        \toprule
        Term & Weight \\
        \midrule
        motion\_global\_root\_pos & 0.5 \\
        motion\_global\_root\_ori & 0.5 \\
        motion\_body\_pos & 2.0 \\
        motion\_body\_ori & 1.5 \\
        motion\_body\_lin\_vel & 1.0 \\
        motion\_body\_ang\_vel & 1.0 \\
        motion\_ee\_body\_pos\_z & 2.0 \\
        motion\_joint\_pos & 0.5 \\
        motion\_joint\_vel & 0.25 \\
        action\_rate\_l2 & -0.005 \\
        joint\_limit & -10.0 \\
        undesired\_contacts & -0.1 \\
        \bottomrule
    \end{tabular}
\end{table}

The sigma values match the G1 Motion Tracking defaults (Table~\ref{tab:app_g1mt_reward}).

\paragraph{G1 Flip Tracking.}
The flip variant uses the flat G1 scene with a 360-degree flip reference clip. Sampling always starts from frame zero, the episode is not truncated when the clip ends, and the simulation step is $0.005$\,s.

Under MuJoCoUni, the anchor and end-effector $z$-error thresholds are both $0.5$\,m, undesired-contact termination is enabled, and the per-joint action scale matches G1 Climb Tracking. Under MotrixSim, the corresponding thresholds and action scale use the baseline environment settings.

\begin{table}[!htbp]
    \centering
    \caption{Reward terms for \texttt{g1\_flip\_tracking}.}
    \label{tab:app_g1ft_reward}
    \begin{tabular}{@{}lcc@{}}
        \toprule
        Term & MuJoCoUni & MotrixSim \\
        \midrule
        motion\_global\_root\_pos & 0.5 & 1.0 \\
        motion\_global\_root\_ori & 0.5 & 0.5 \\
        motion\_body\_pos & 2.0 & 1.0 \\
        motion\_body\_ori & 1.5 & 1.0 \\
        motion\_body\_lin\_vel & 1.0 & 1.0 \\
        motion\_body\_ang\_vel & 1.0 & 1.0 \\
        motion\_ee\_body\_pos\_z & 2.0 & / \\
        action\_rate\_l2 & -0.005 & -0.05 \\
        joint\_limit & -10.0 & -10.0 \\
        undesired\_contacts & -0.1 & / \\
        \bottomrule
    \end{tabular}
\end{table}

\paragraph{G1 Wall Flip Tracking.}
The wall-flip variant uses a flat scene with a wall and a wall-flip reference clip. Sampling always starts from frame zero, the episode is not truncated when the clip ends, the simulation step is $0.005$\,s, anchor and end-effector $z$-error thresholds are both $0.5$\,m, undesired-contact termination is enabled, and the per-joint action scale matches G1 Climb Tracking. Under MotrixSim, the solver runs three substep iterations per control step.

Reward scales are identical across the two backends and match the climb-tracking weights (Table~\ref{tab:app_g1ct_reward}); only the reference clip and the wall-scene termination geometry change.

\paragraph{G1 Box Tracking.}
The box variant uses a flat scene with a large box and a box-manipulation reference clip. It extends G1 Motion Tracking with explicit object-state tracking: the critic observation appends 12 extra dimensions (object position, object 6D orientation, object linear velocity, all in body frame) for a 314-dimensional critic. The actor observation remains 176-dimensional. Under MuJoCoUni, the simulation step is $0.005$\,s; under MotrixSim, the base step is used.

Under MotrixSim, empirical normalization is enabled, an asymmetric critic observation group is declared, and observation noise uses level $1.0$ with joint-angle scale $0.01$, joint-velocity scale $1.5$, and gyro scale $0.2$.

\begin{table}[!htbp]
    \centering
    \caption{Reward terms for \texttt{g1\_box\_tracking}.}
    \label{tab:app_g1bt_reward}
    \small
    \begin{tabular}{@{}lcc@{}}
        \toprule
        Term & MuJoCoUni & MotrixSim \\
        \midrule
        motion\_global\_root\_pos & 0.5 & 1.0 \\
        motion\_global\_root\_ori & 0.5 & 0.5 \\
        motion\_body\_pos & 1.0 & 1.0 \\
        motion\_body\_ori & 1.0 & 1.5 \\
        motion\_body\_lin\_vel & 1.0 & 1.0 \\
        motion\_body\_ang\_vel & 1.0 & 1.5 \\
        action\_rate\_l2 & -0.1 & -0.1 \\
        joint\_limit & -10.0 & -10.0 \\
        undesired\_contacts & -0.1 & -0.1 \\
        object\_global\_ref\_position\_error\_exp & 2.0 & 4.0 \\
        object\_global\_ref\_orientation\_error\_exp & 2.0 & 3.0 \\
        \bottomrule
    \end{tabular}
\end{table}

Body-tracking sigmas inherit the G1 Motion Tracking defaults; the object-tracking sigmas used inside $\exp(-e^2/\sigma^2)$ differ between backends: $\sigma_{\mathrm{object\_pos}}=0.2$ (MuJoCoUni) / $0.12$ (MotrixSim), $\sigma_{\mathrm{object\_ori}}=0.3$ (MuJoCoUni) / $0.2$ (MotrixSim).
